# Supplementary material for: Resource-constrained knowledge diffusion processes inspired by human peer learning
Source: arXiv:2312.00660 source file (2023-12-01)
Supplement: Supplementary file 1 [file appendix.tex]

\newpage

~ \vfill 

\newpage

\appendix
\onecolumn

\section{Appendix. Additional Results}
\label{sec:appendix}

%\subsection{Omitted Plots}
%This section contains some plots omitted from Section~\ref{sec:results}.

\begin{figure*}[h!]
    \centering
    {\includegraphics[width=0.32\textwidth]{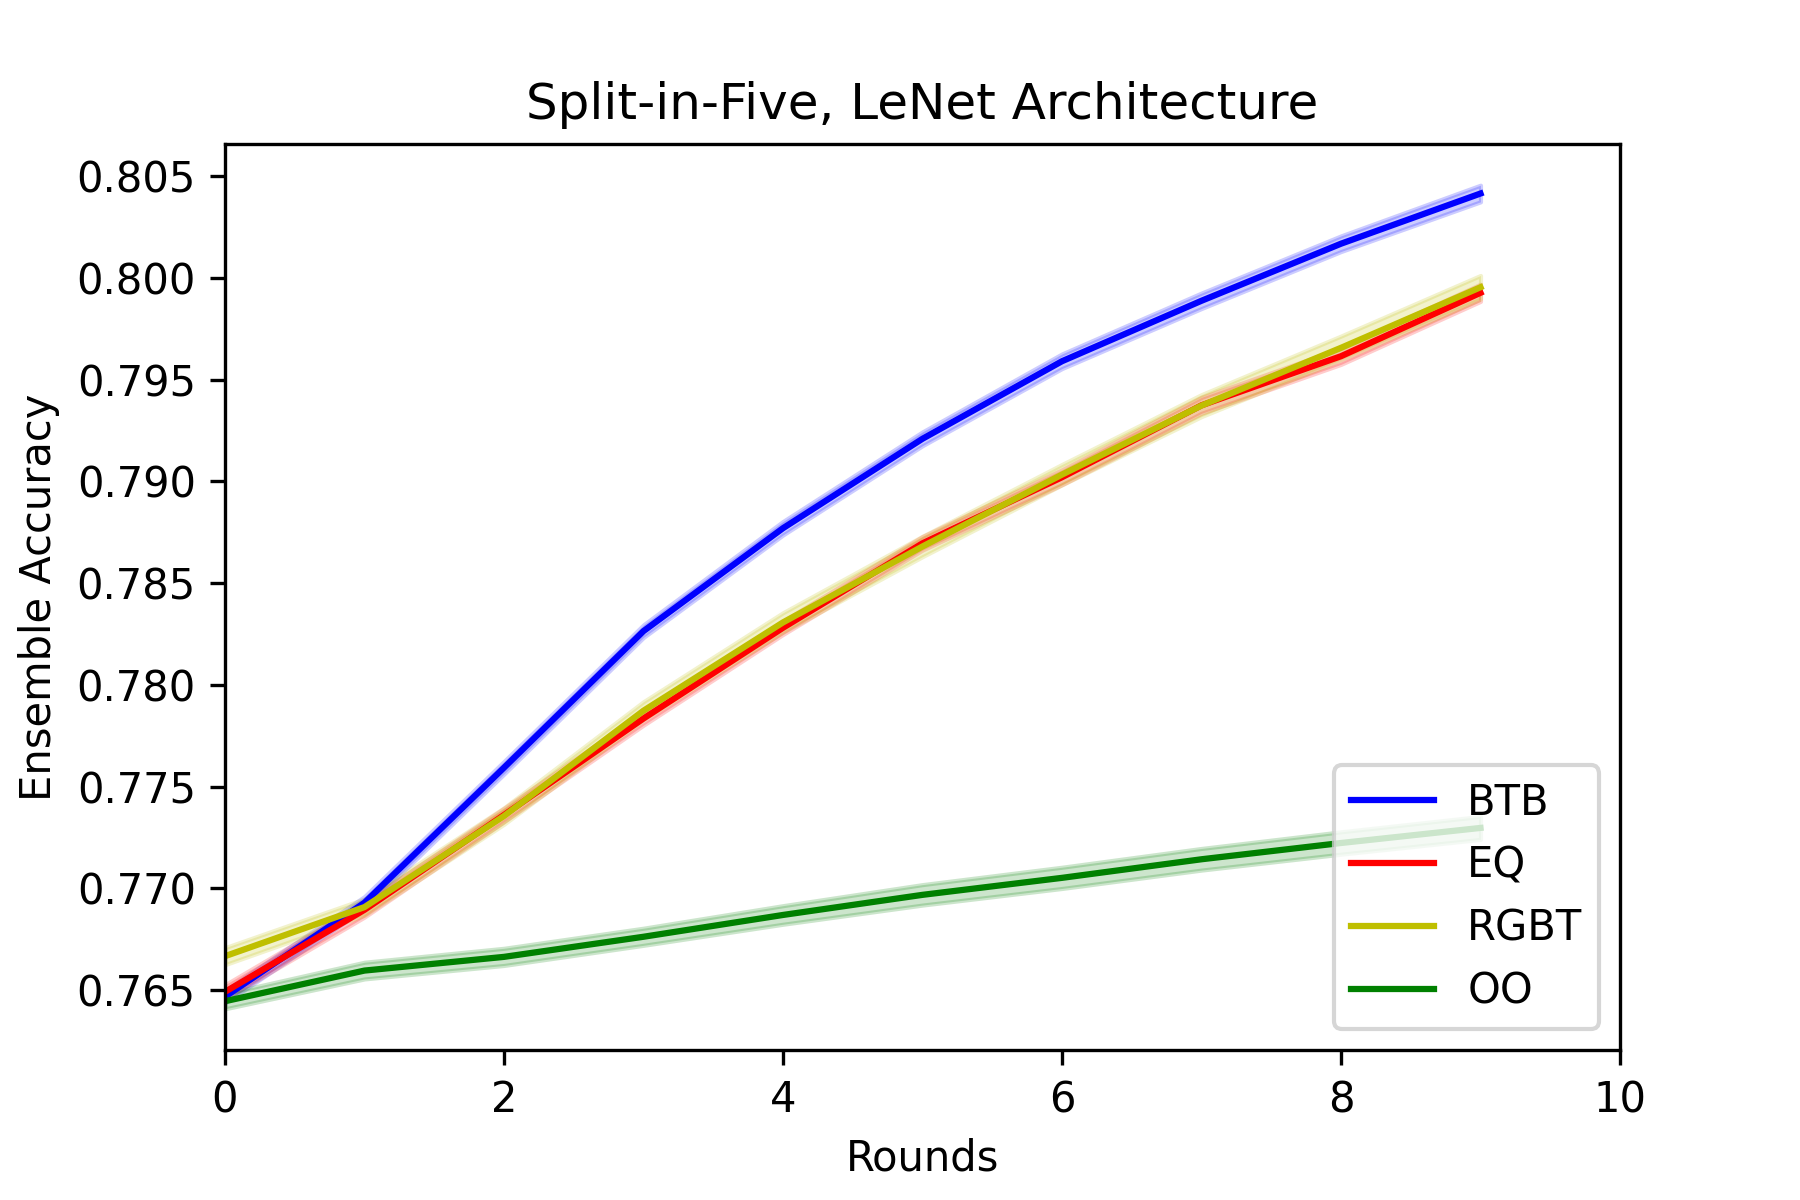}} 
    {\includegraphics[width=0.32\textwidth]{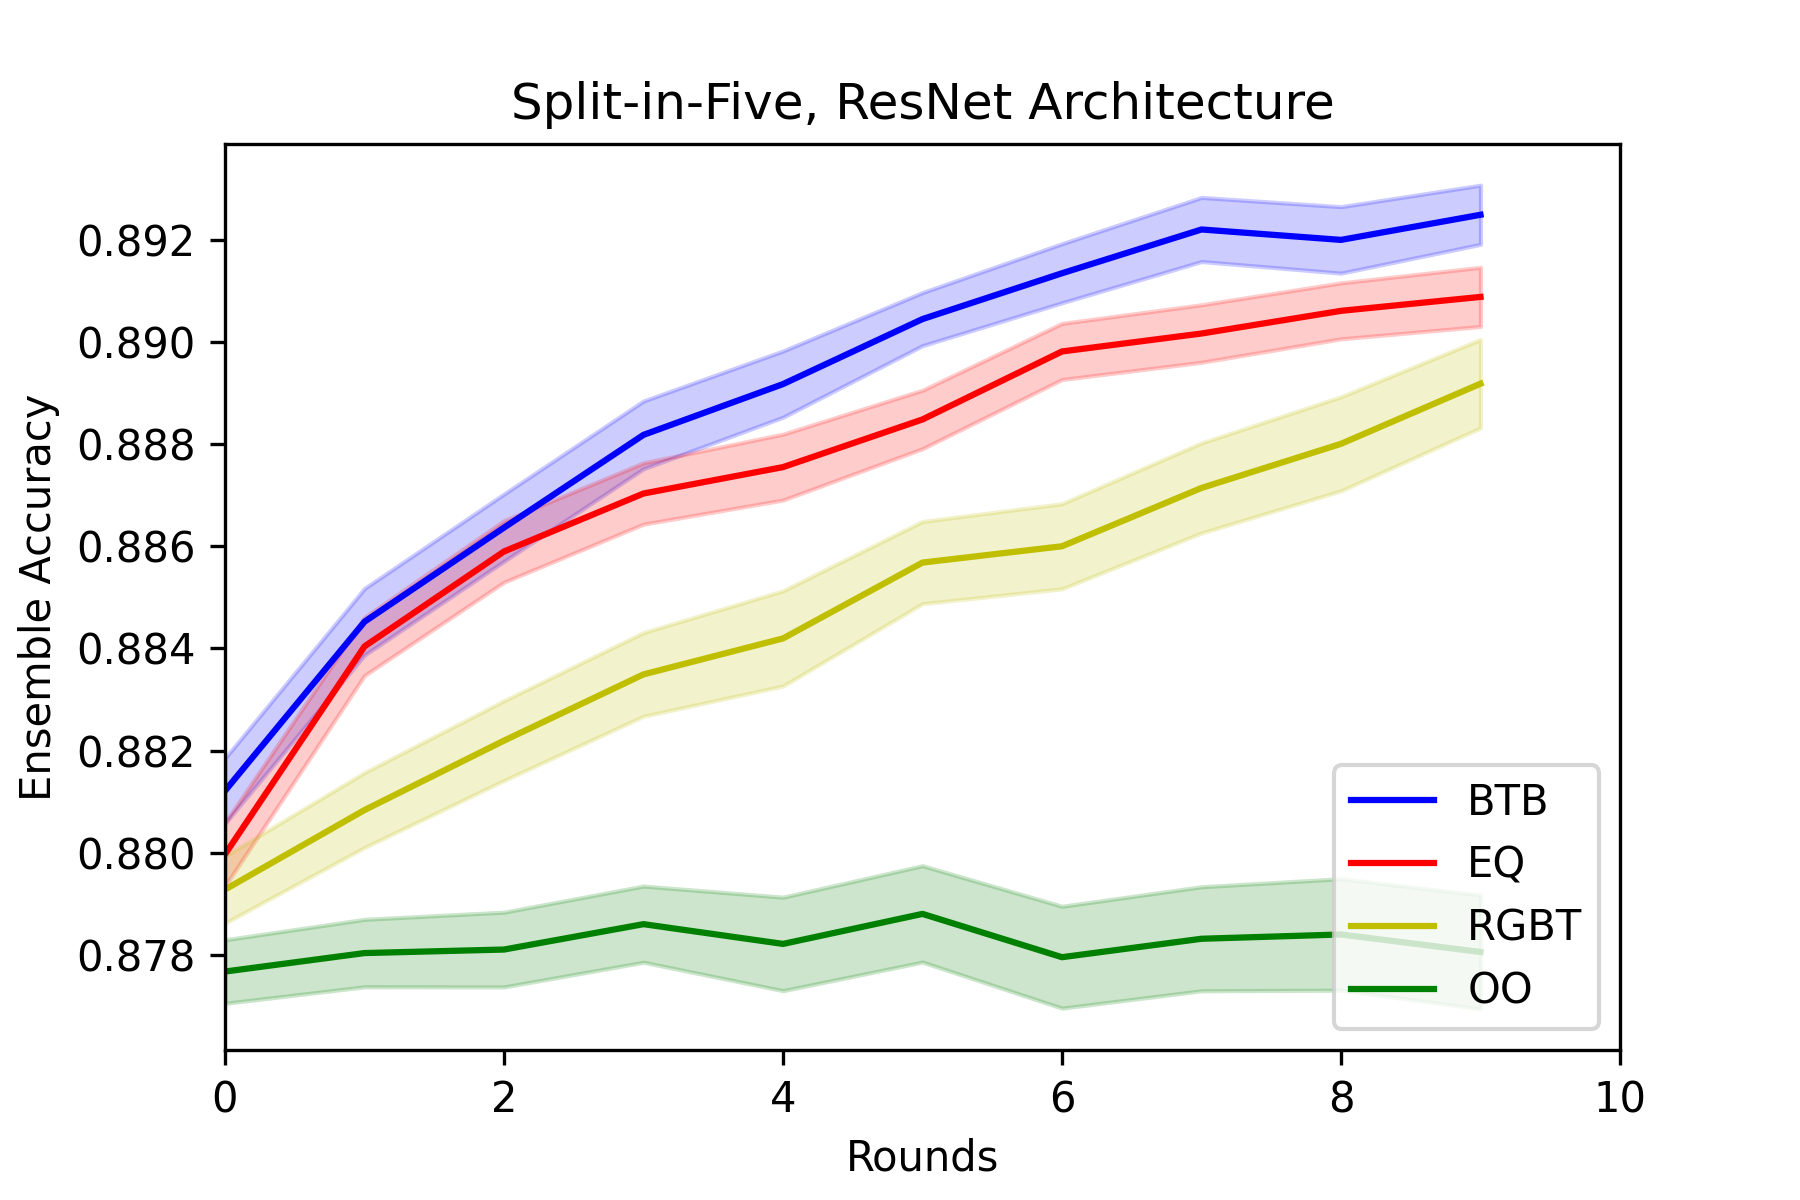}} 
    {\includegraphics[width=0.32\textwidth]{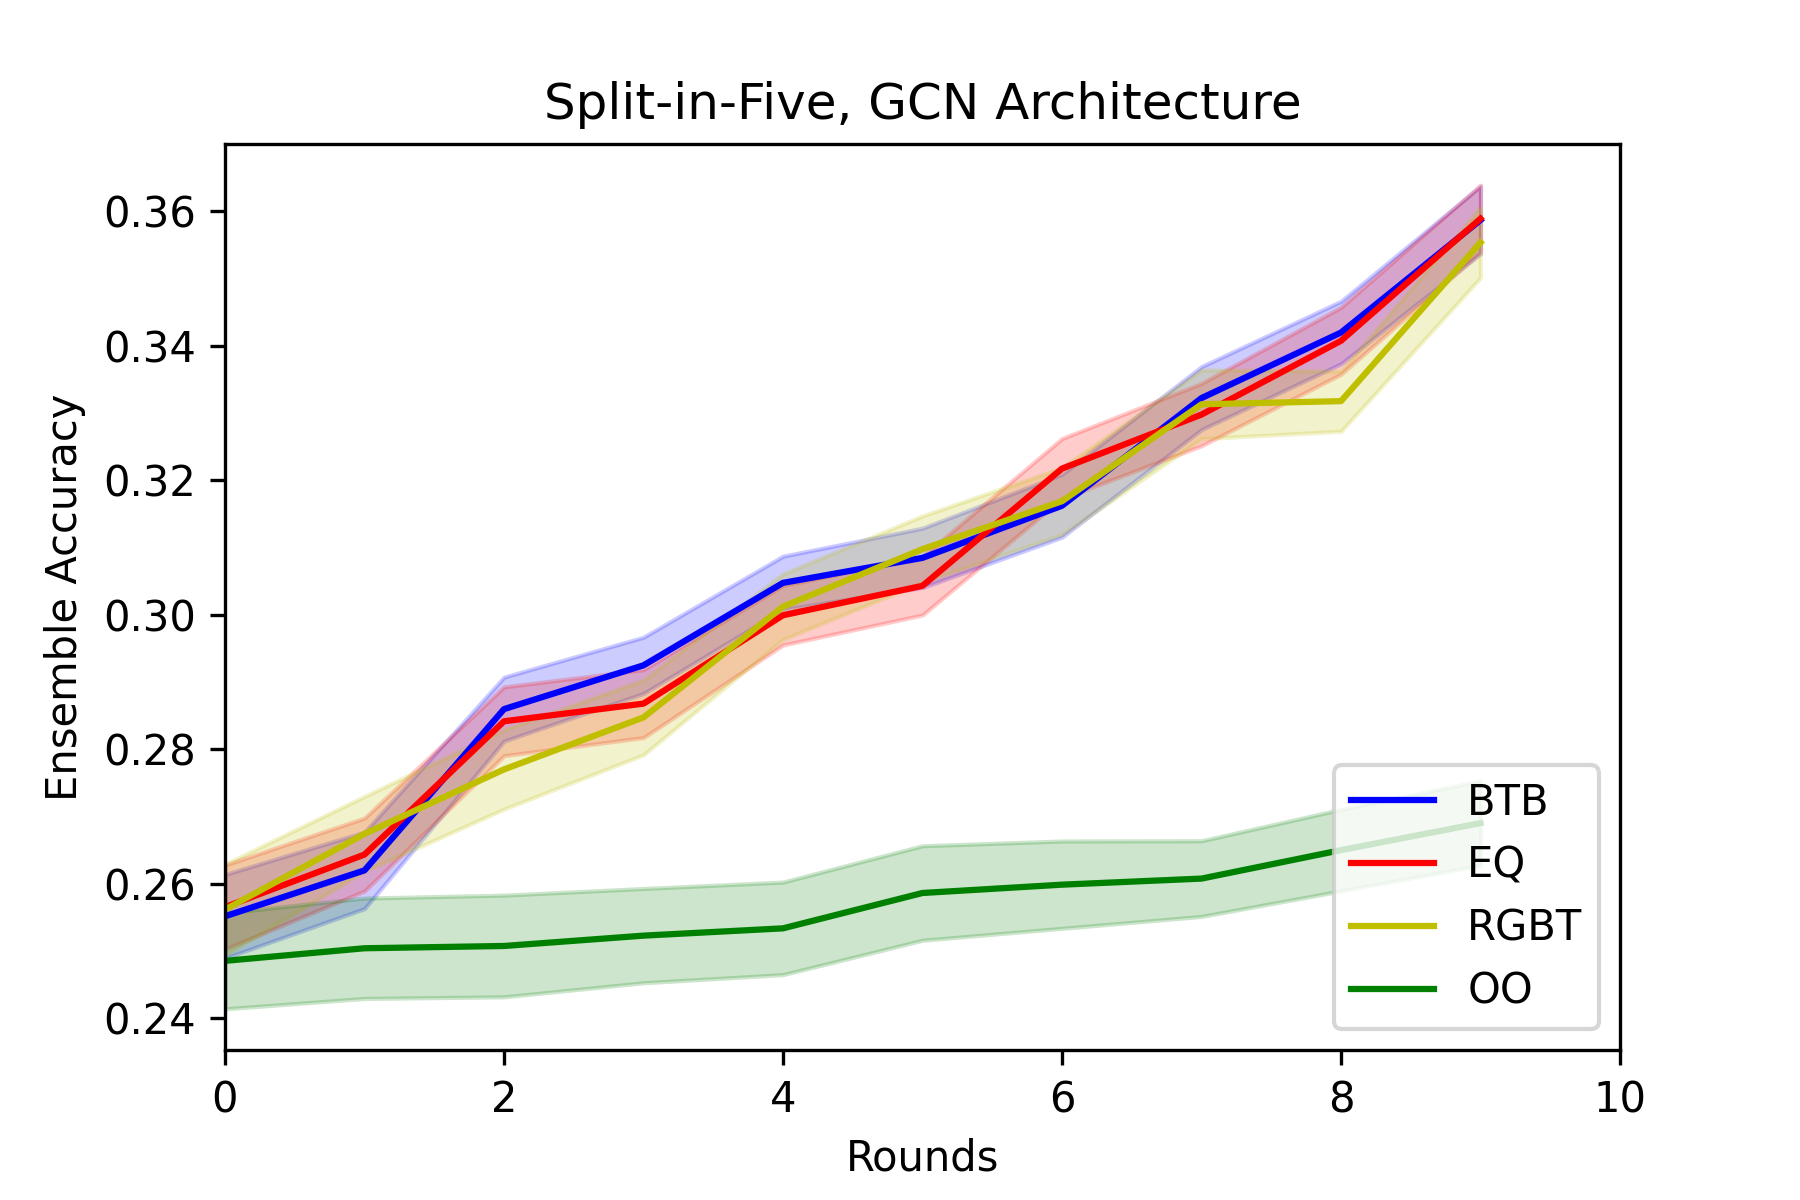}} 
    {\includegraphics[width=0.32\textwidth]{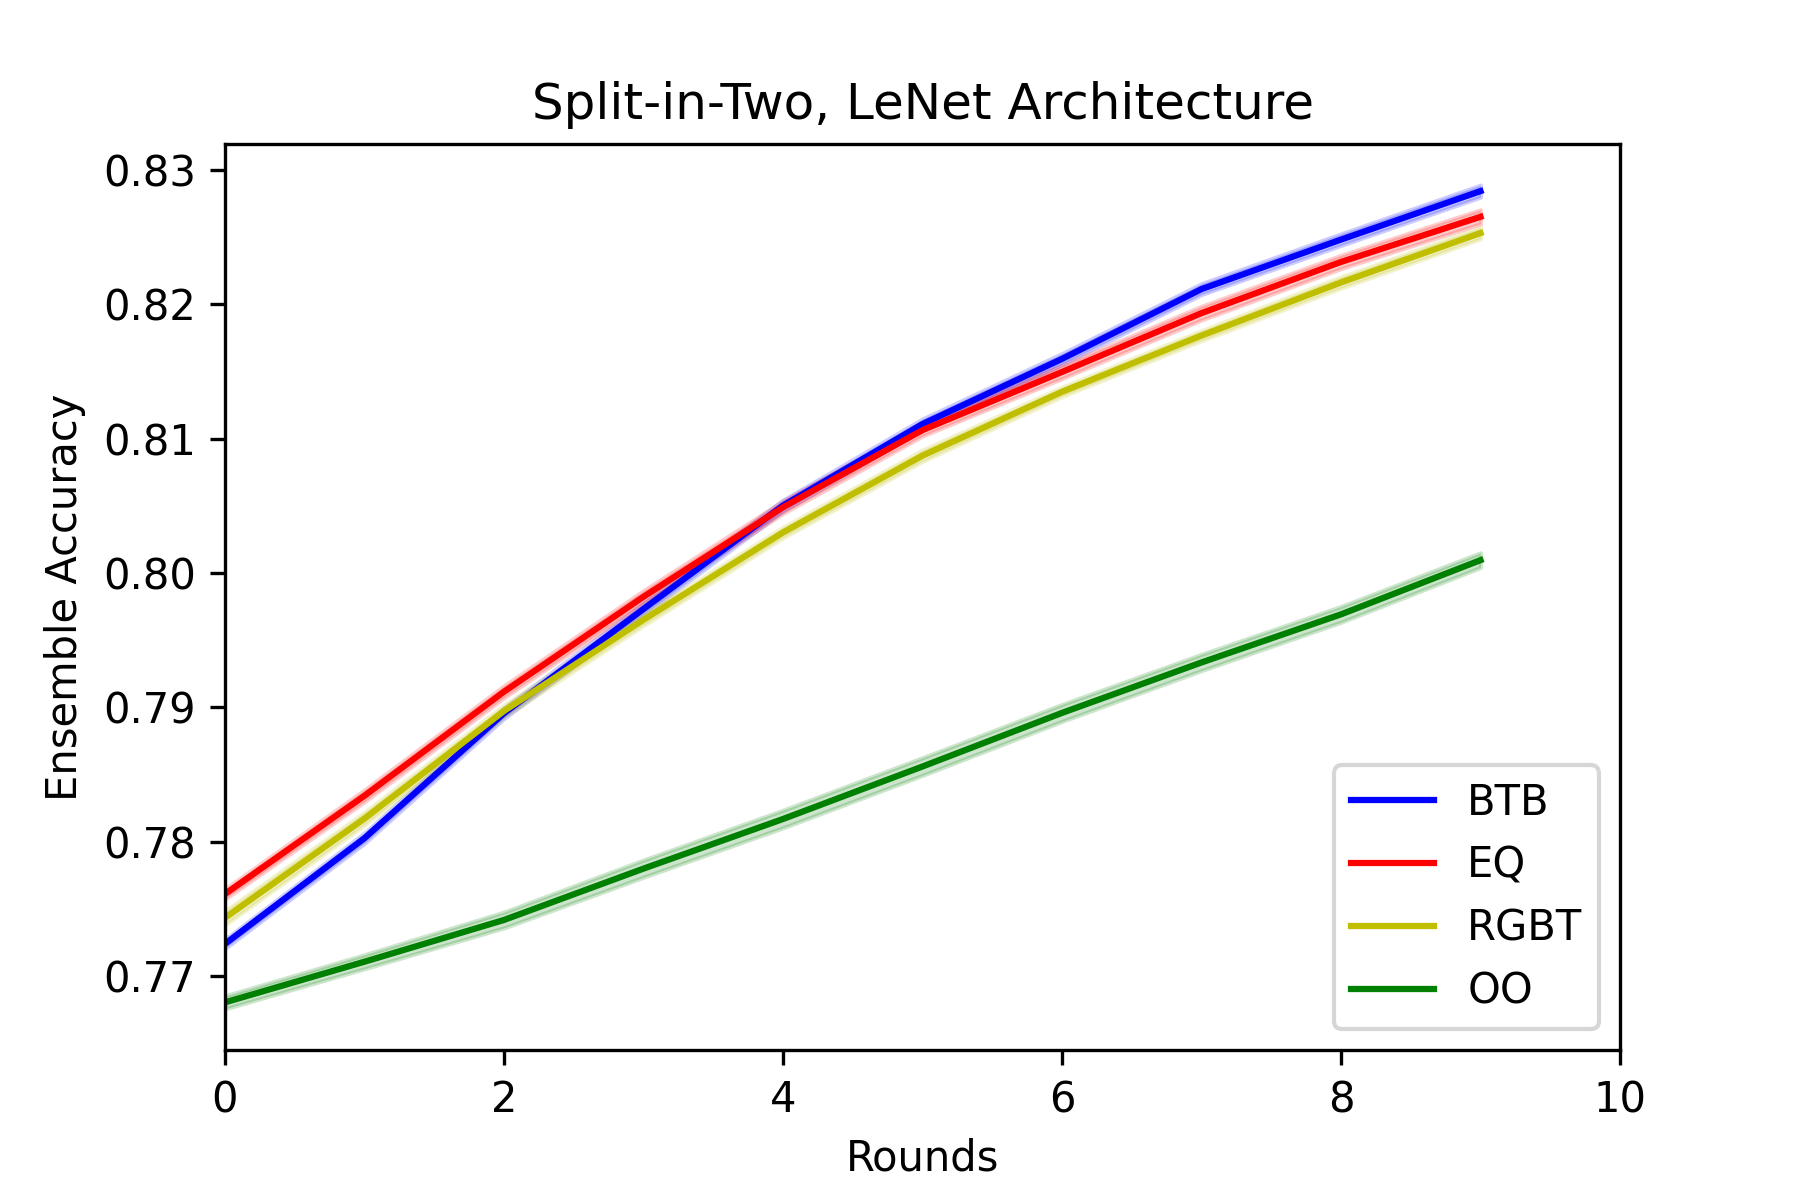}} 
    {\includegraphics[width=0.32\textwidth]{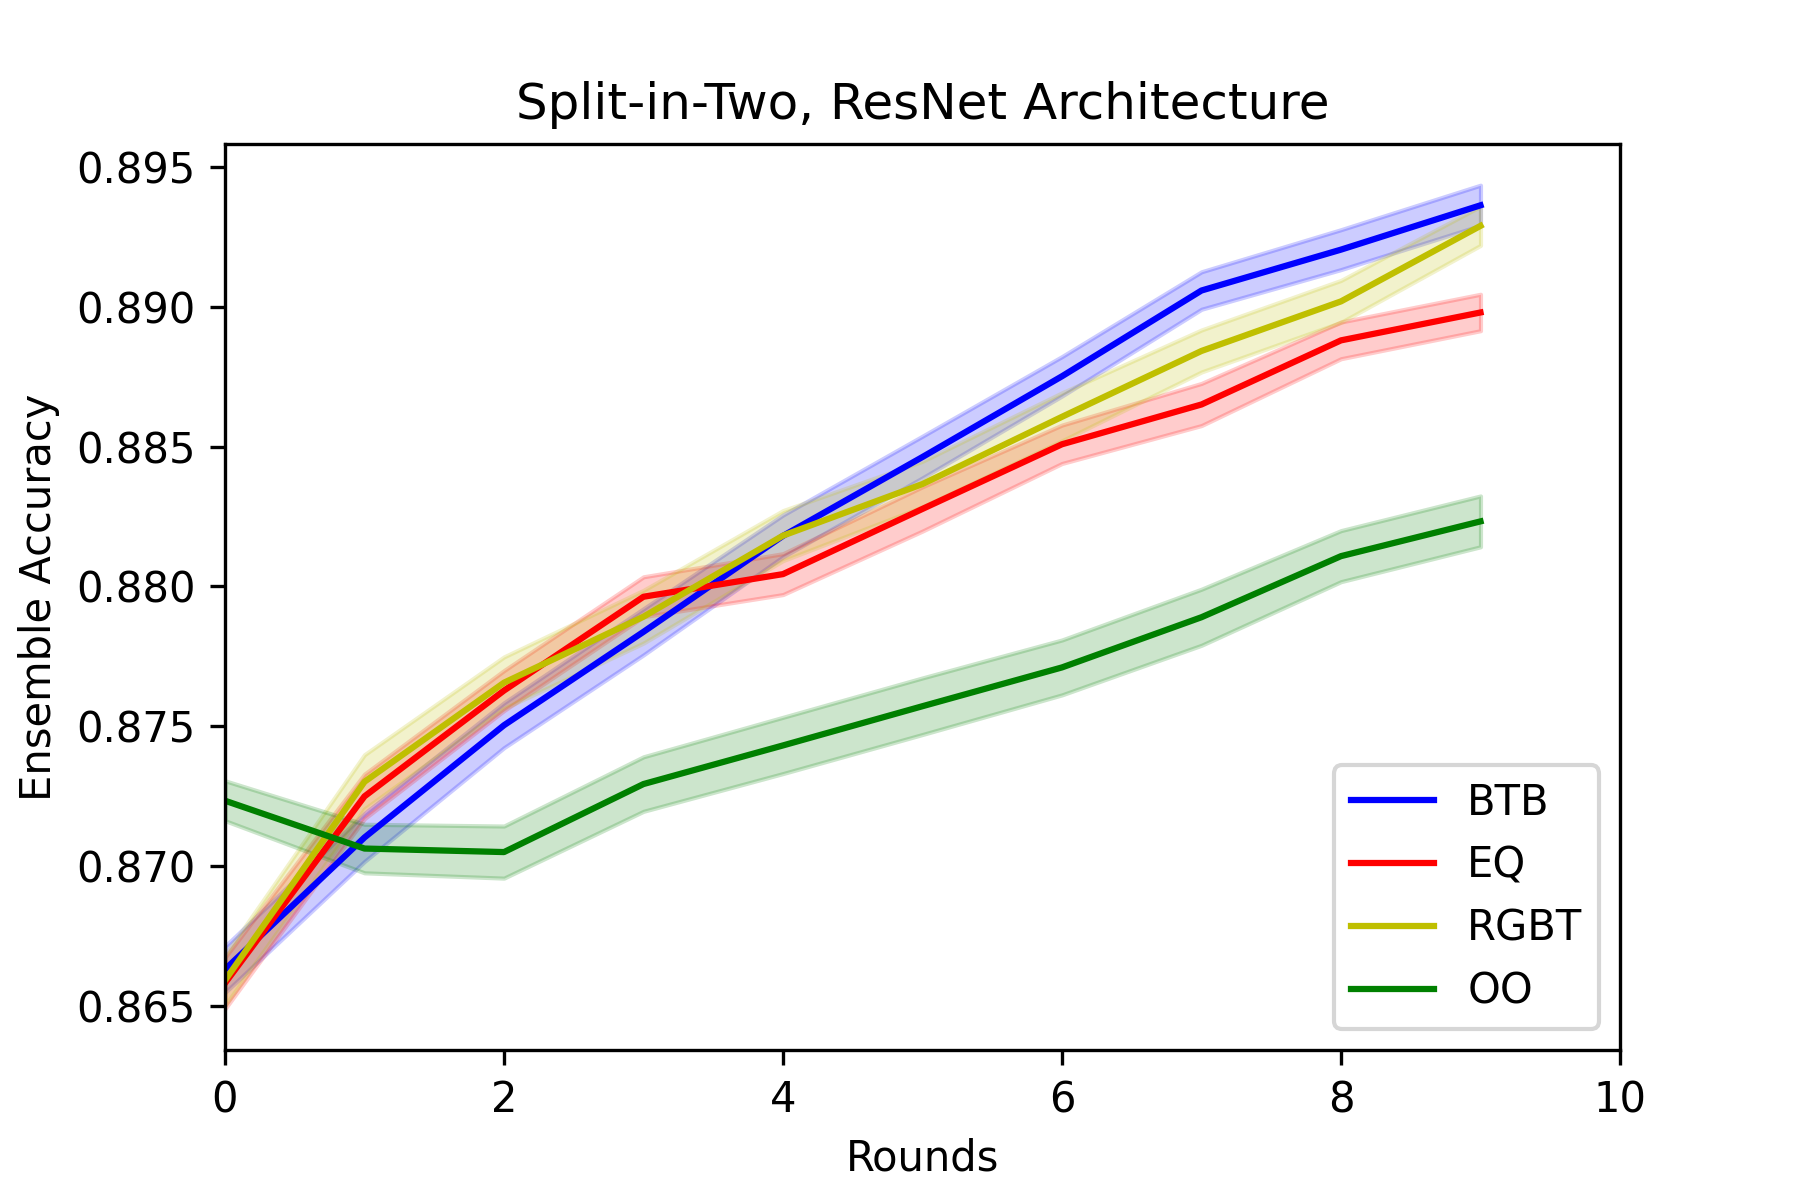}} 
    {\includegraphics[width=0.32\textwidth]{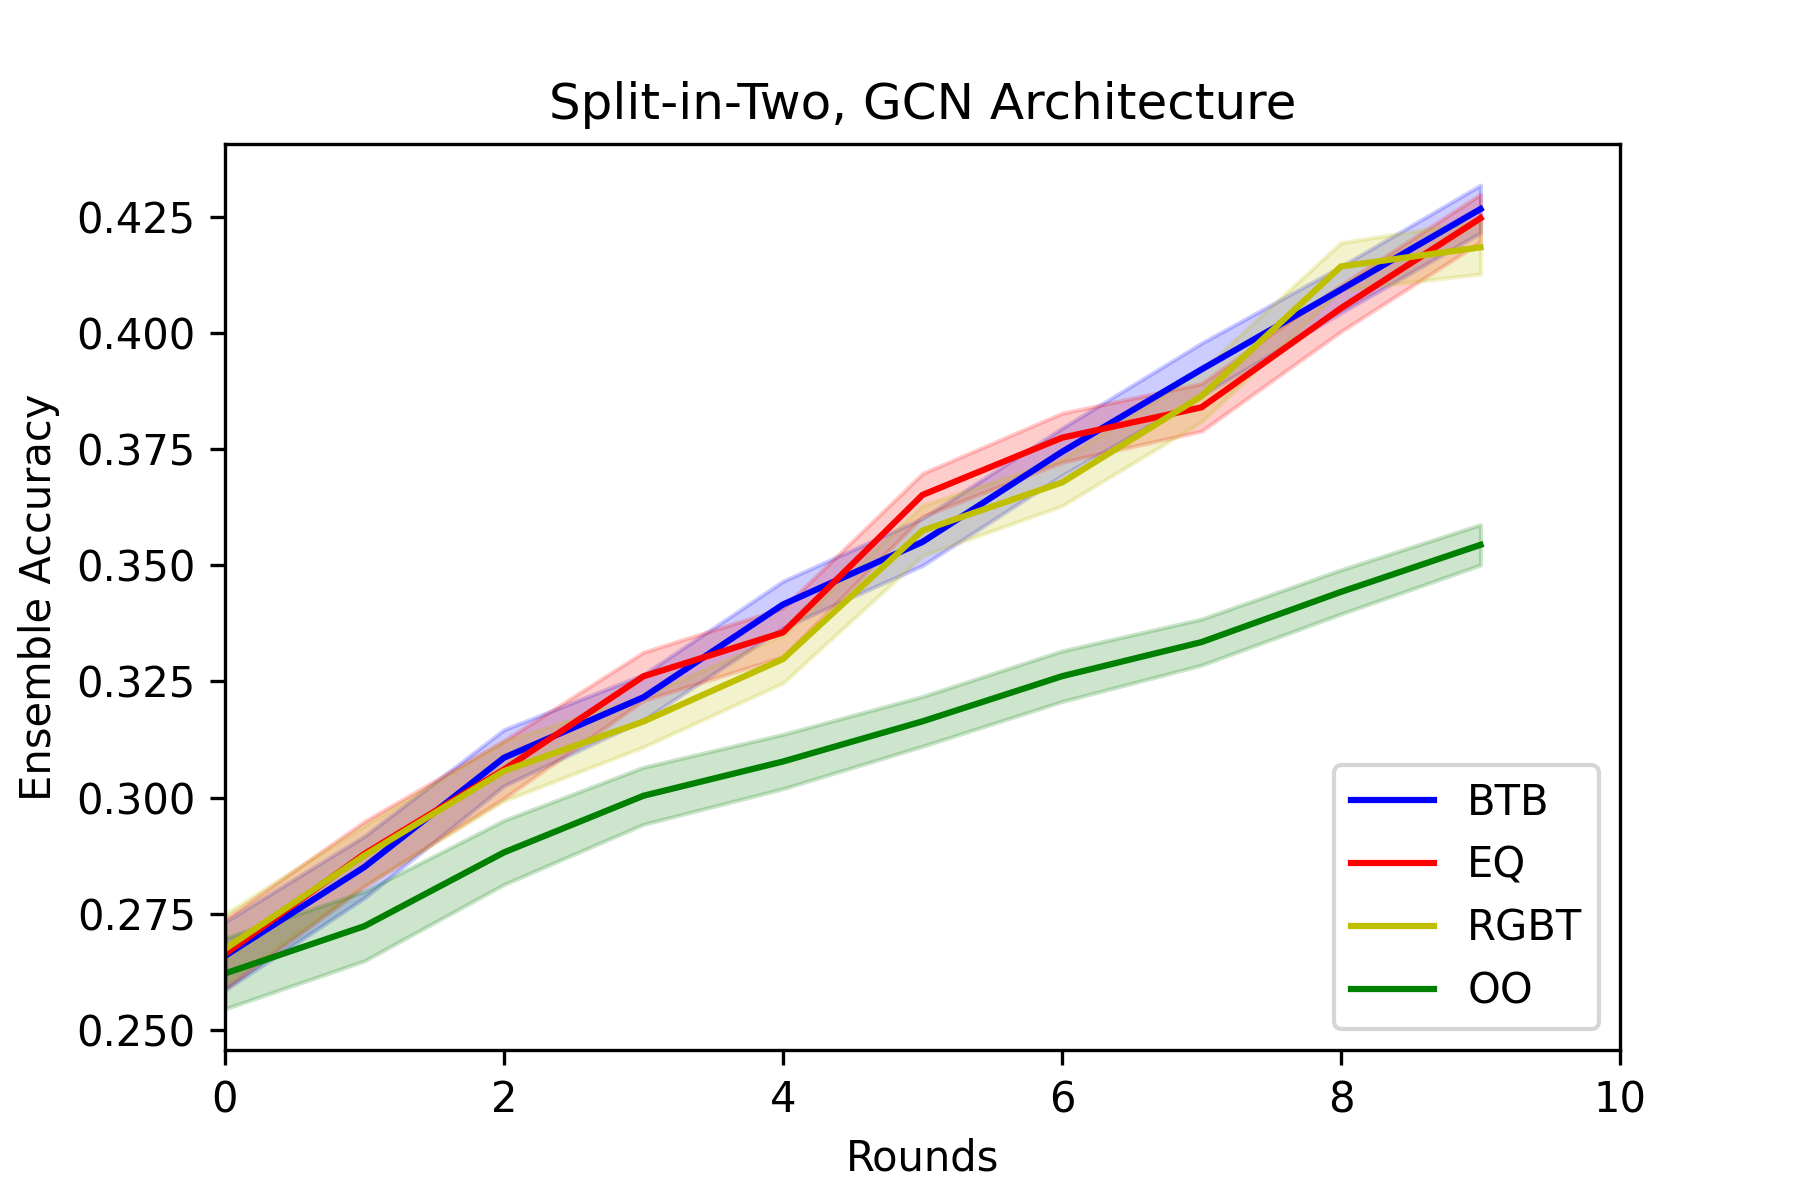}} 
    \caption{Ensemble Accuracy $acc_{\cal E}$ on test set for 10 rounds/epochs \textbf{with pre-training}, for C=2 (above) and C=5 (below).  \\ \textbf{ Comment:} $acc_{\cal E}$ is higher for higher $C$.  Note that the reported metrics are averages over multiple random experiments, as discussed in Section~\ref{sec:setting}. Policy {\em BTB} appears to outperform.}
    \label{fig:ensemble_pretrain_}
\end{figure*}

\begin{figure*}[h]
    \centering
    {\includegraphics[width=0.32\textwidth]{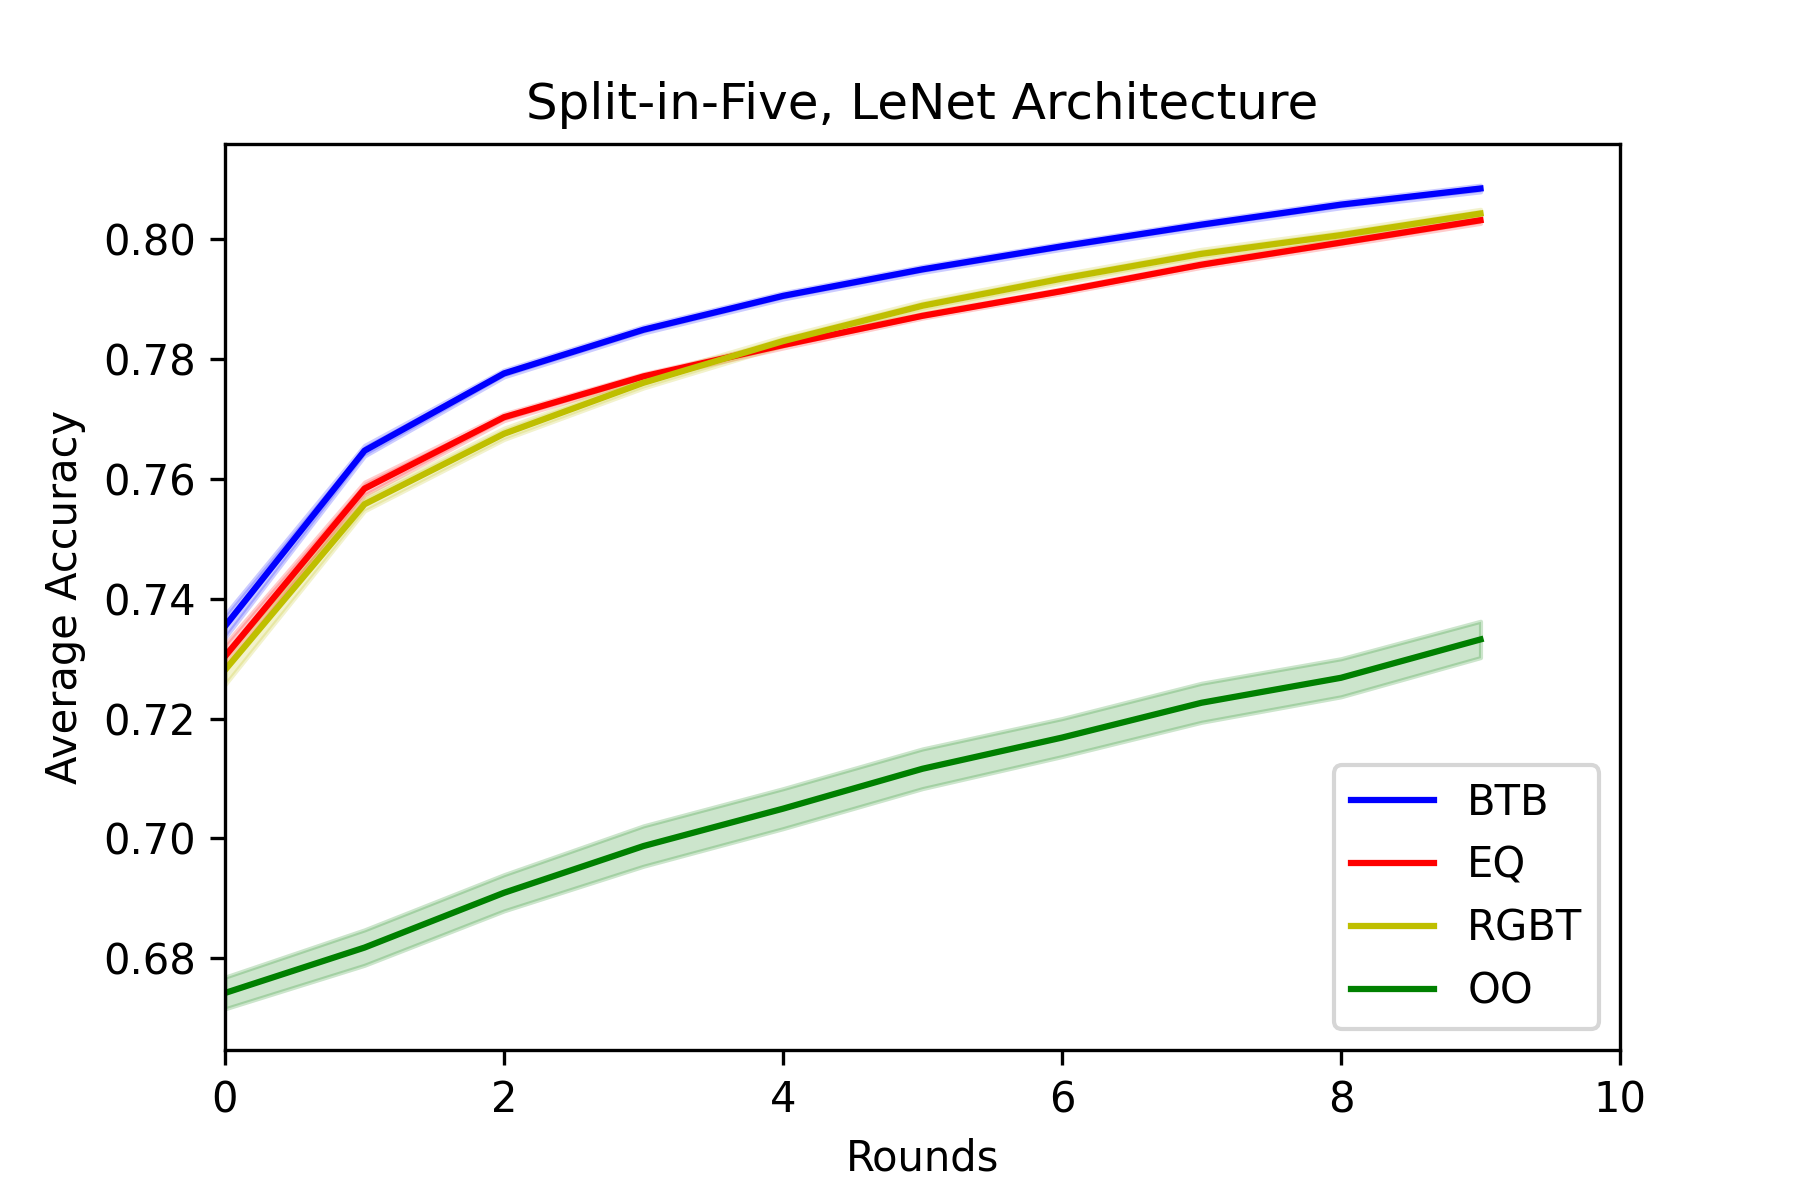}} 
    {\includegraphics[width=0.32\textwidth]{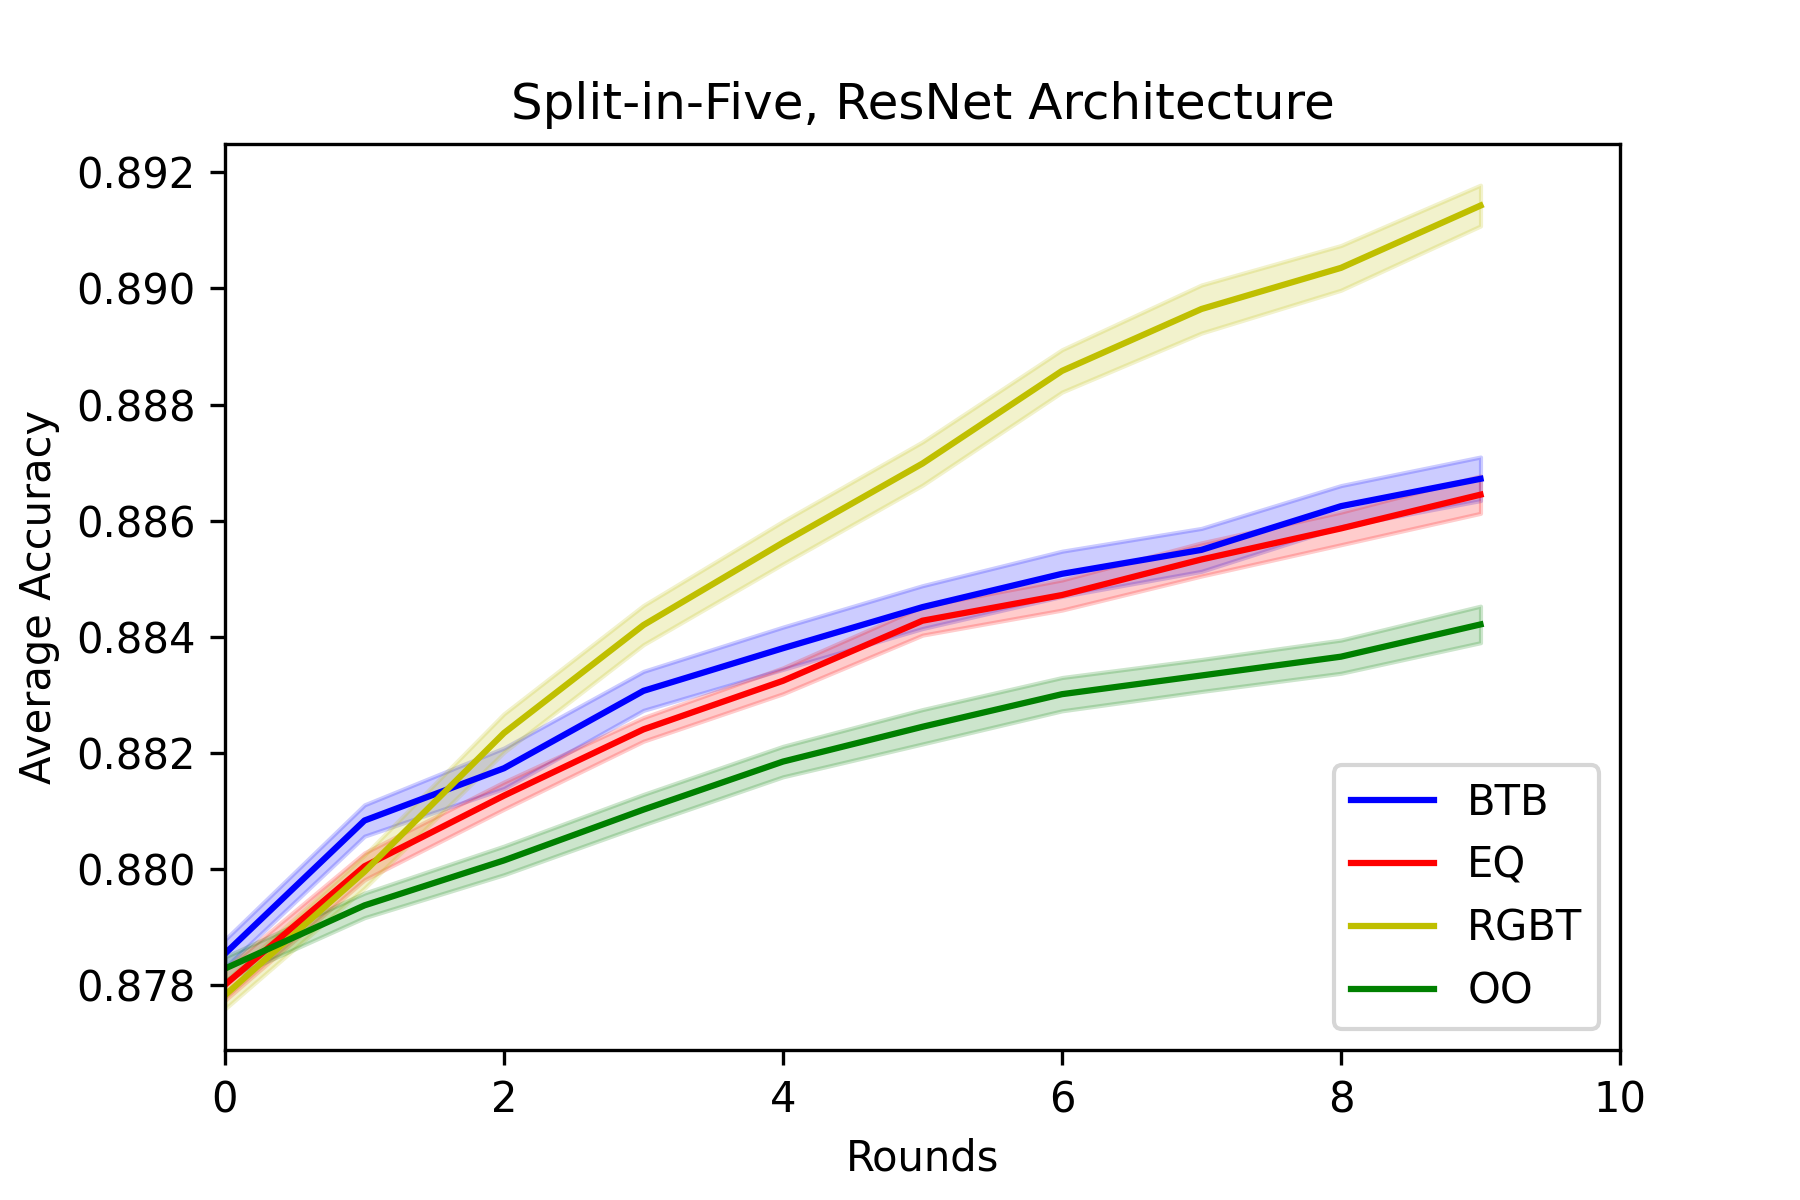}} 
    {\includegraphics[width=0.32\textwidth]{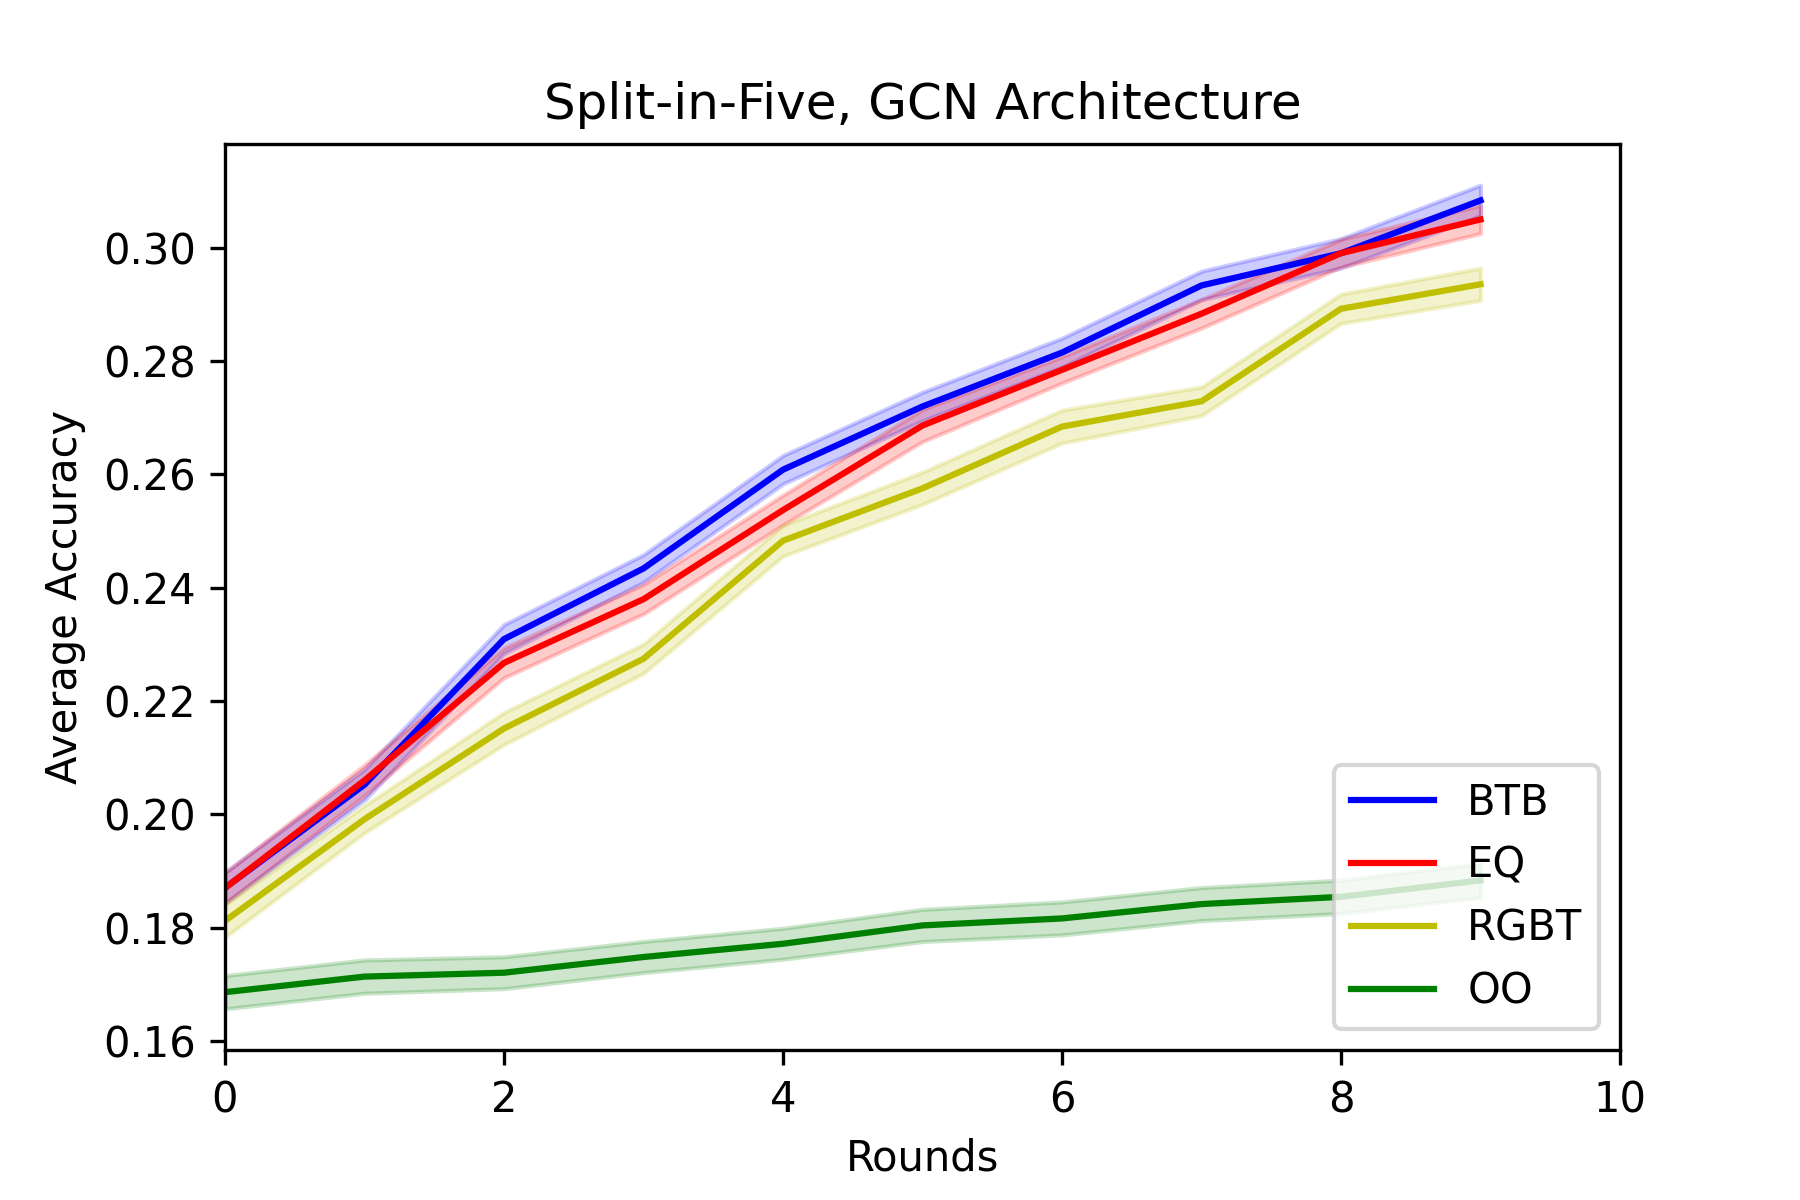}} 
    {\includegraphics[width=0.32\textwidth]{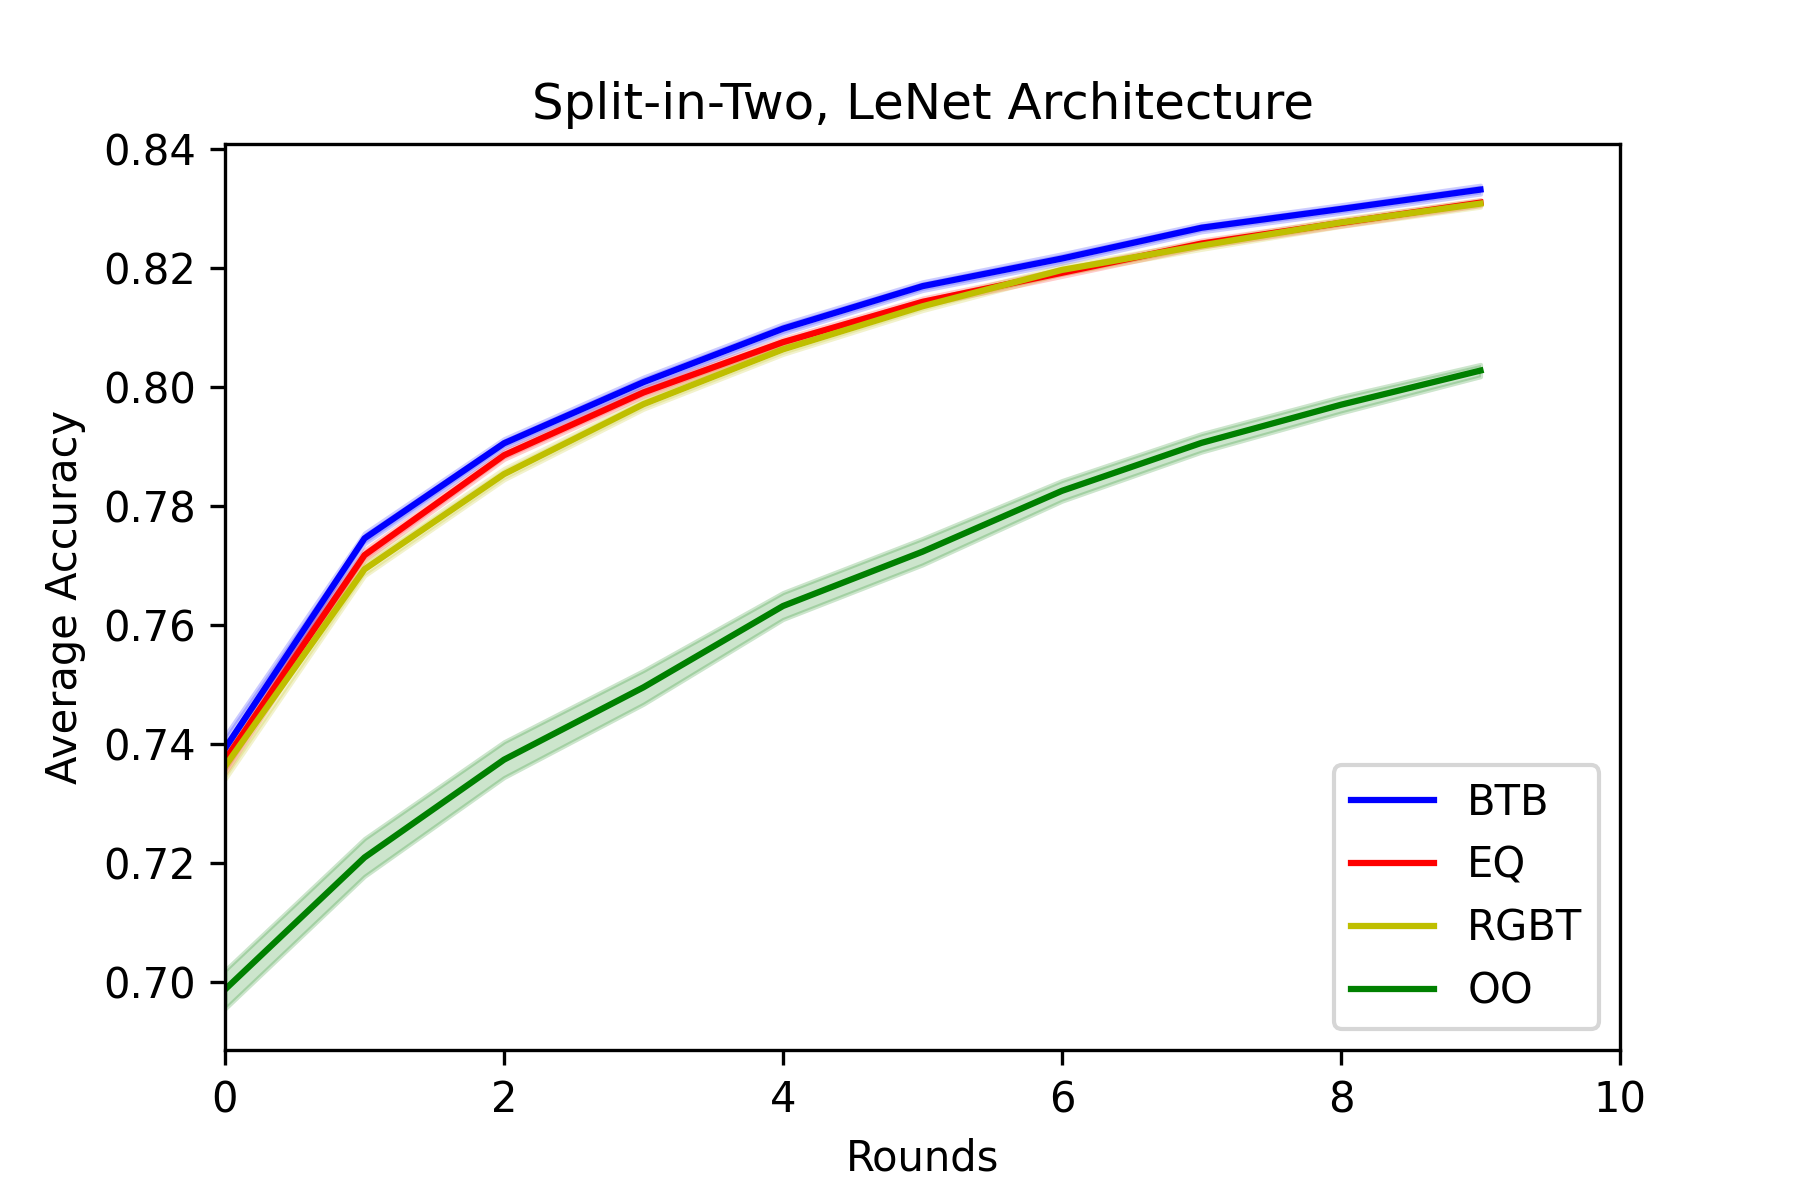}} 
    {\includegraphics[width=0.32\textwidth]{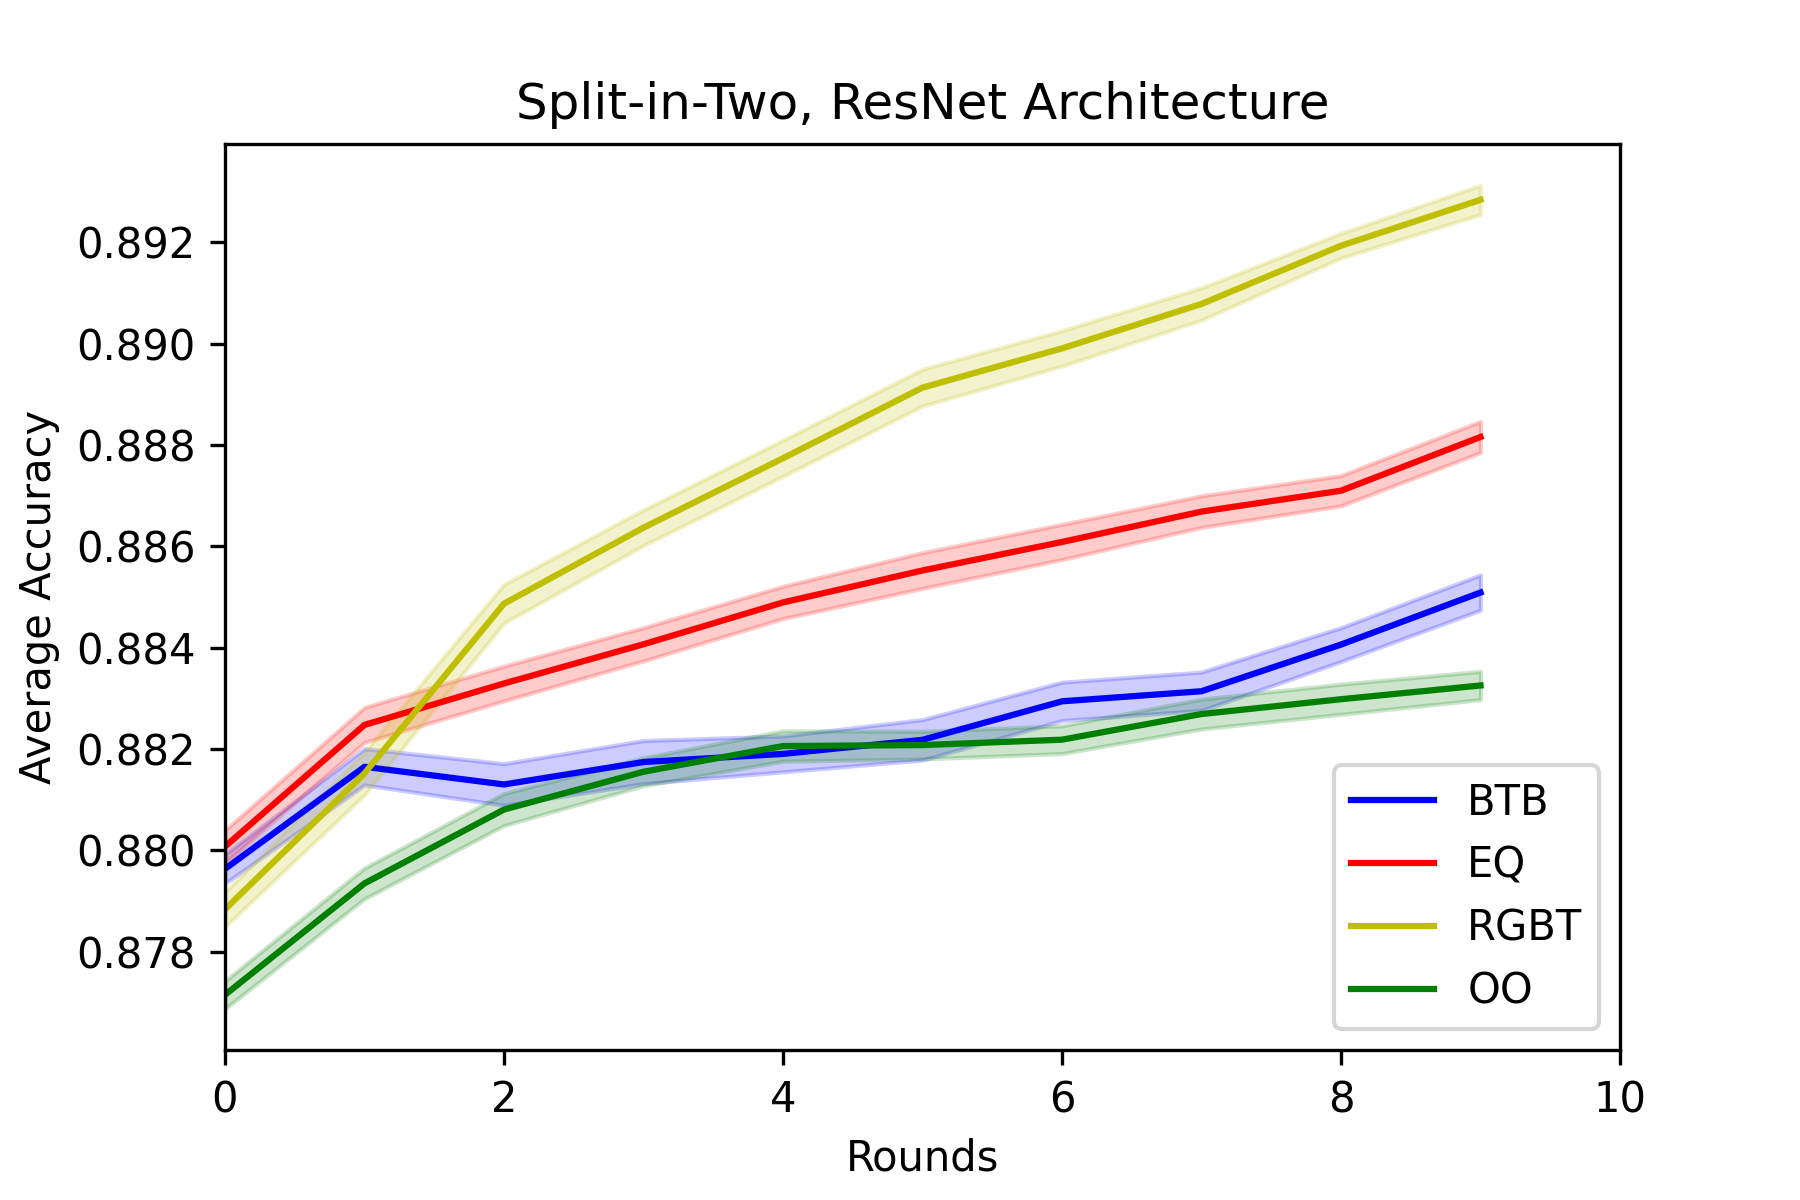}} 
    {\includegraphics[width=0.32\textwidth]{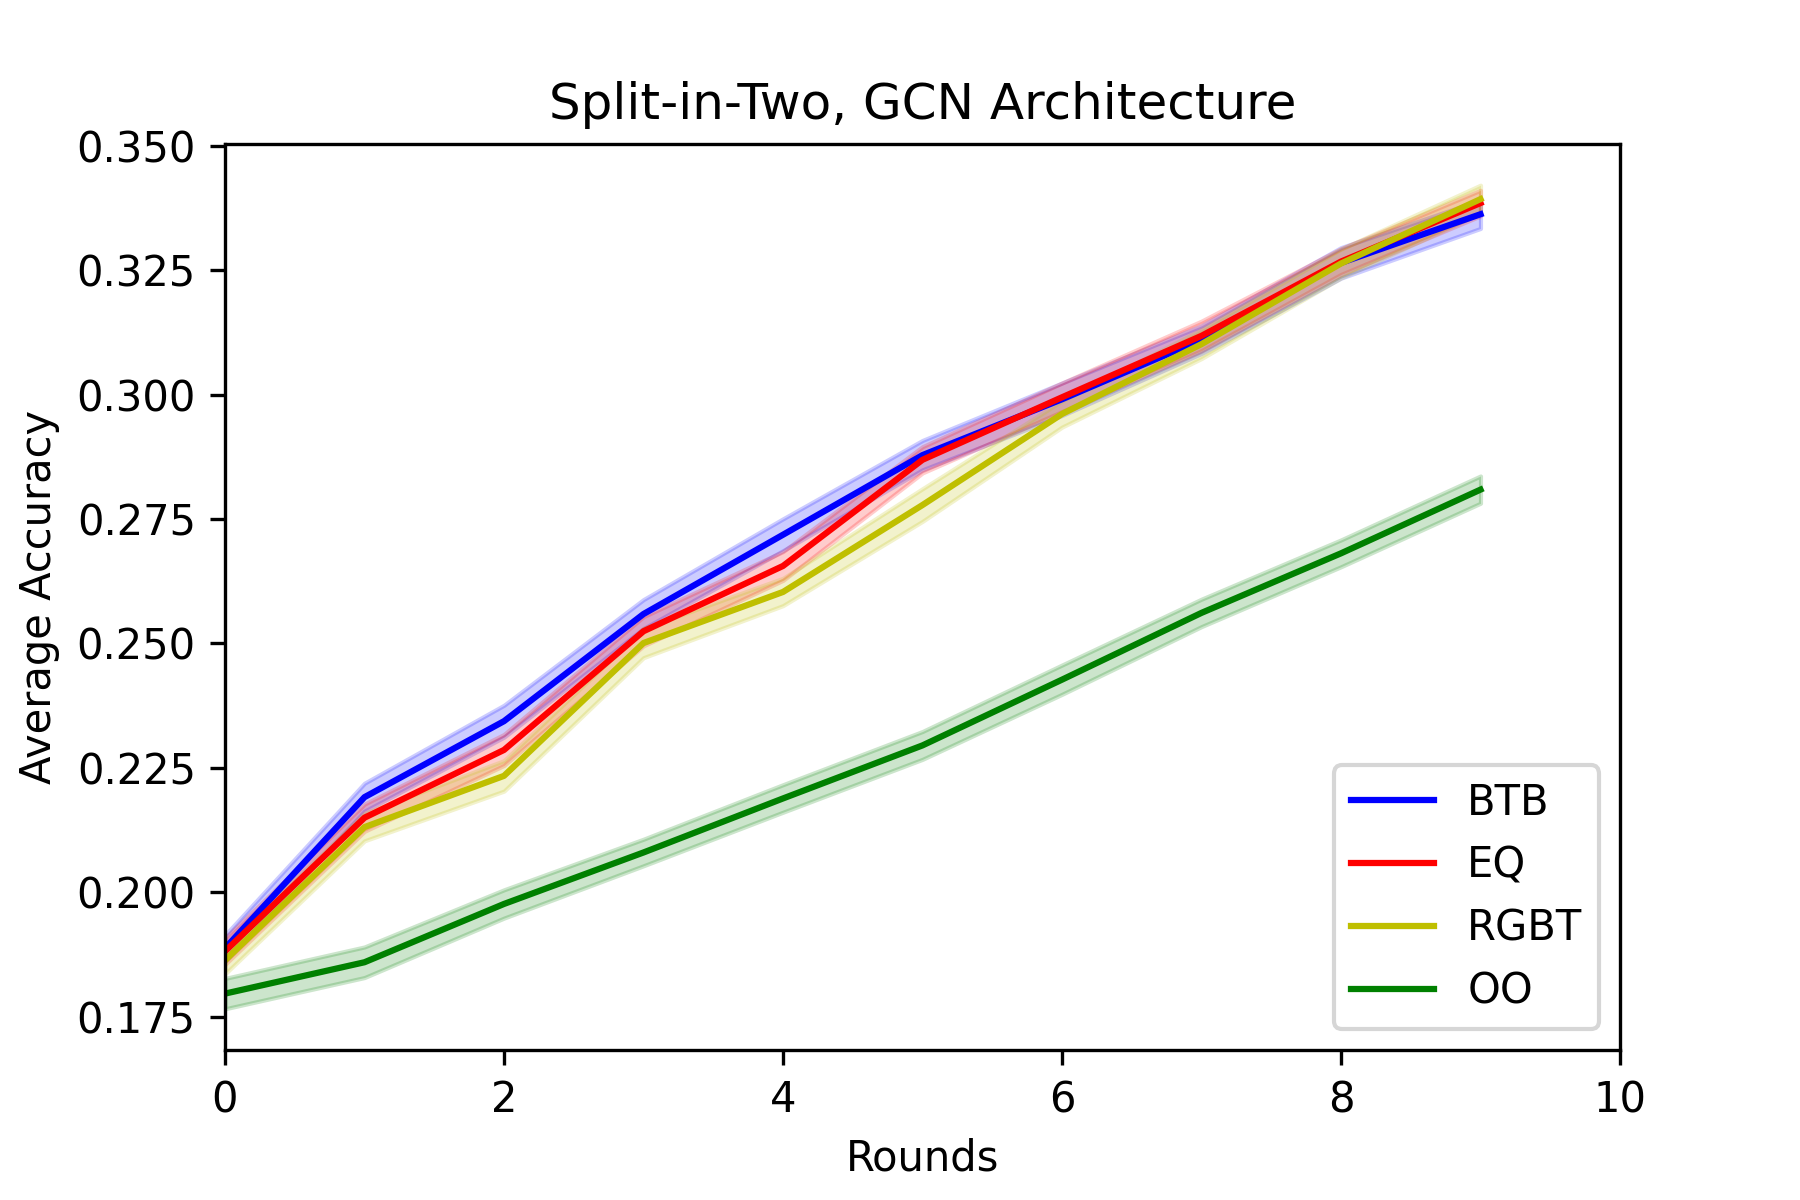}} 
    \caption{Average Learner Accuracy $alacc_{\cal E}$ on test set for 10 rounds/epochs \textbf{with pre-training}, for C=2 (above) and C=5 (below).  \\ \textbf{Comment:} $alacc_{\cal E}$ is higher for higher $acc_{\cal E}$. Note that the reported metrics are averages over multiple random experiments, as discussed in Section~\ref{sec:setting}. Policy {\em BTB} appears to outperform on LeNet and GCN. However the moderately coordinate {\em RGBT} outperforms on ResNet. Note that ResNet is a much bigger and deeper model that already reaches very high accuracy after round 1. This may suggest that Random Grouping policies may be better for later stages of learning. It is also worth studying ResNet in a setting with more granular rounds, as discussed in Section~\ref{sec:open}.
    }
   \label{fig:average_pretrain}
\end{figure*}

%%%%%%%%%%%%%%%%%%%%%%%%%%%%%%%%%%%%%%%%%%%%%%%%%%%%%%%%%%%%%%%%%%%%%%%%%%%%%%%
%%%%%%%%%%%%%%%%%%%%%%%%%%%%%%%%%%%%%%%%%%%%%%%%%%%%%%%%%%%%%%%%%%%%%%%%%%%%%%%

\newpage
% No pretrain: Supplementary
\begin{figure*}[h]
\centering
\includegraphics[width=0.30\textwidth]{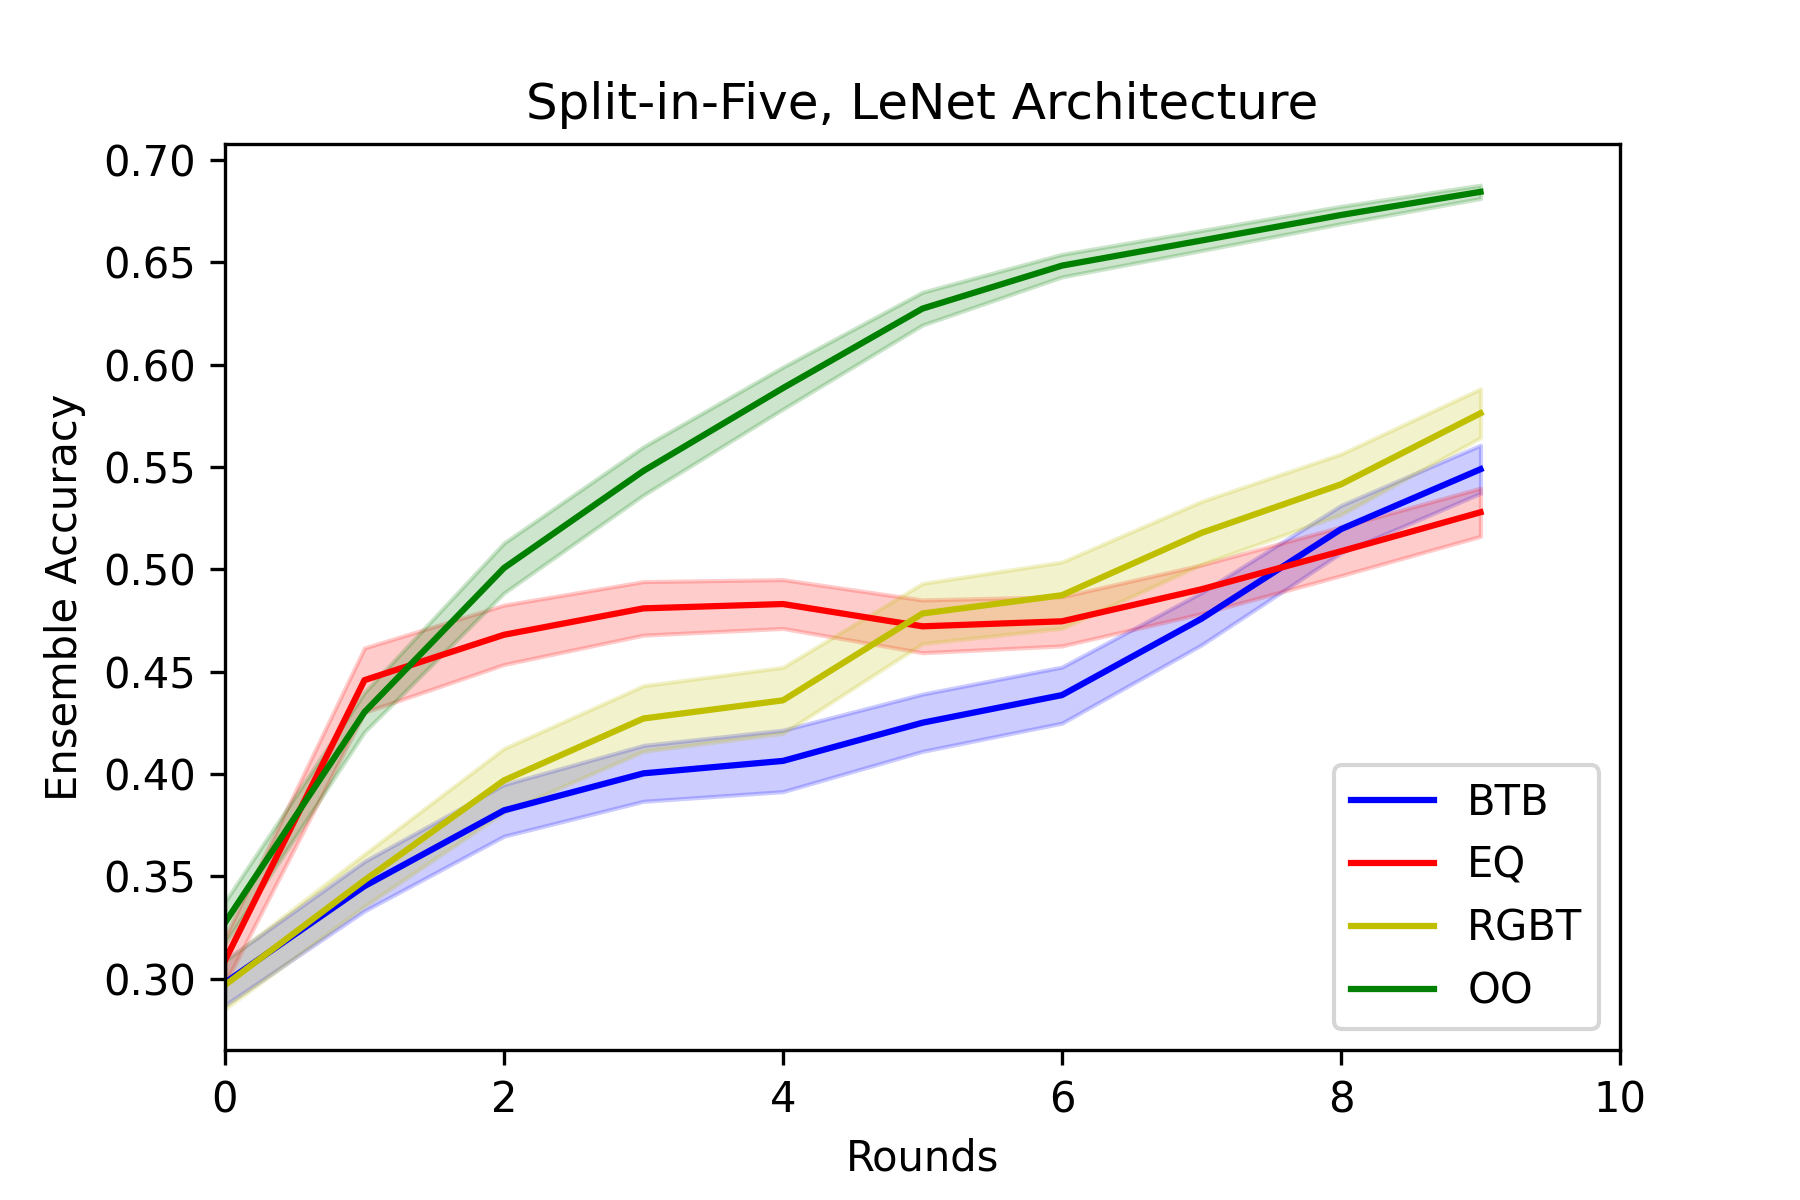}
\includegraphics[width=0.30\textwidth]{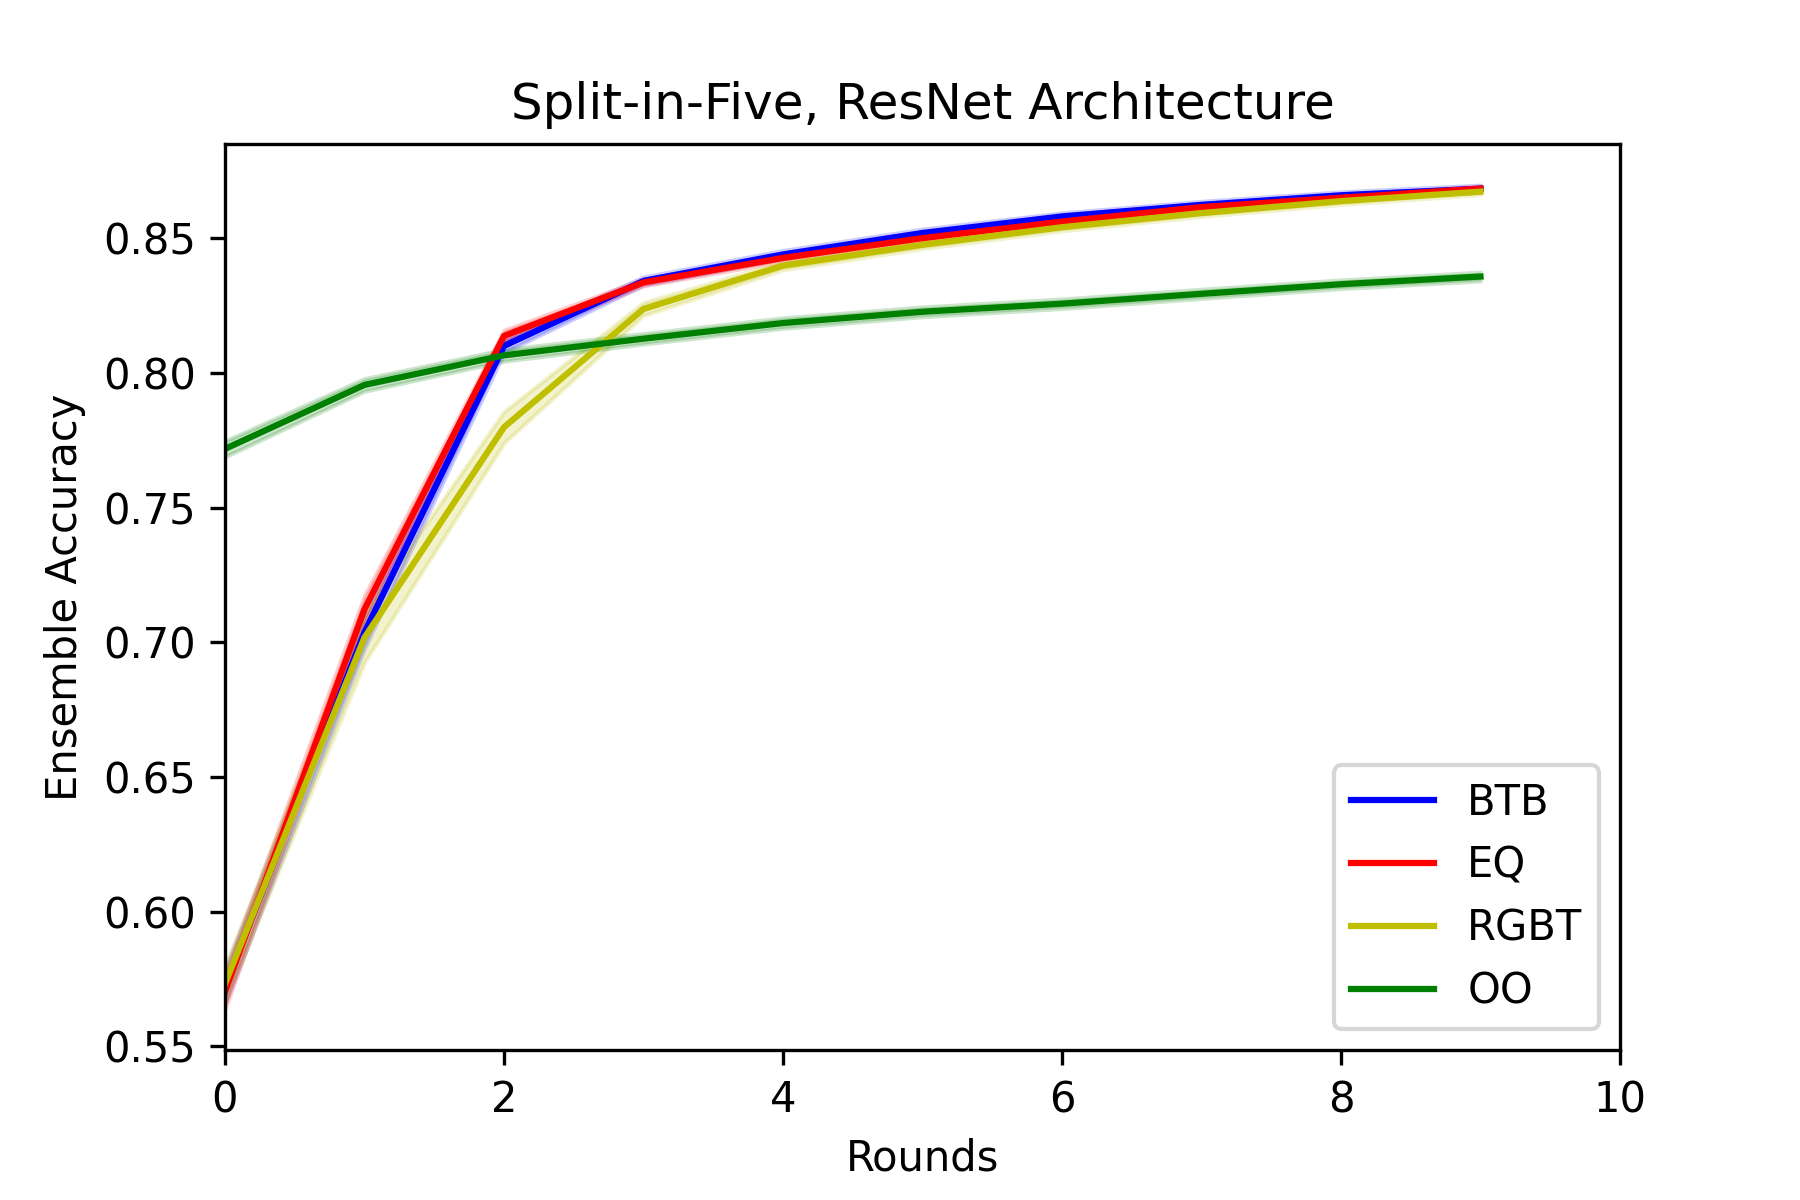}
\includegraphics[width=0.30\textwidth]{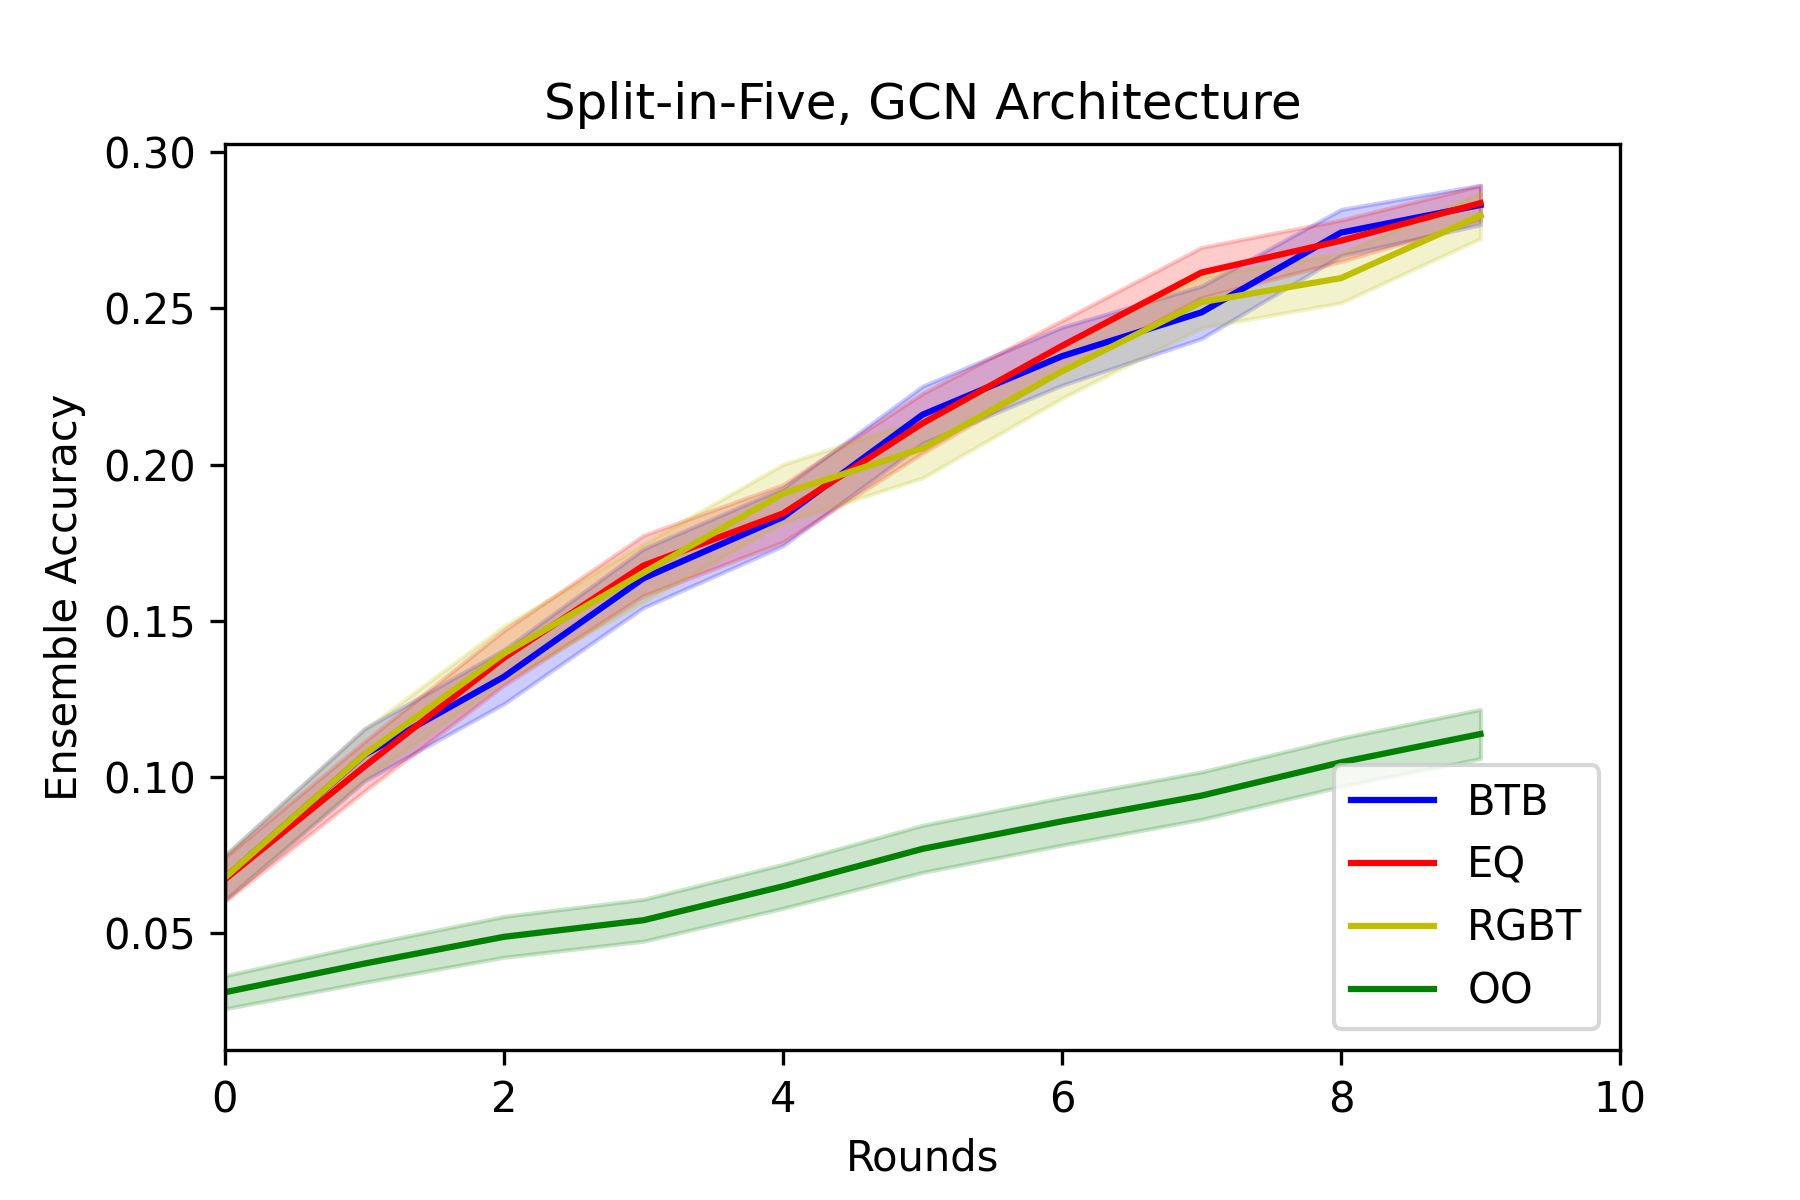}
\includegraphics[width=0.30\textwidth]{Figures/Ensemble_no_pretrain/GCN_Paired_shaded.png}
\includegraphics[width=0.30\textwidth]{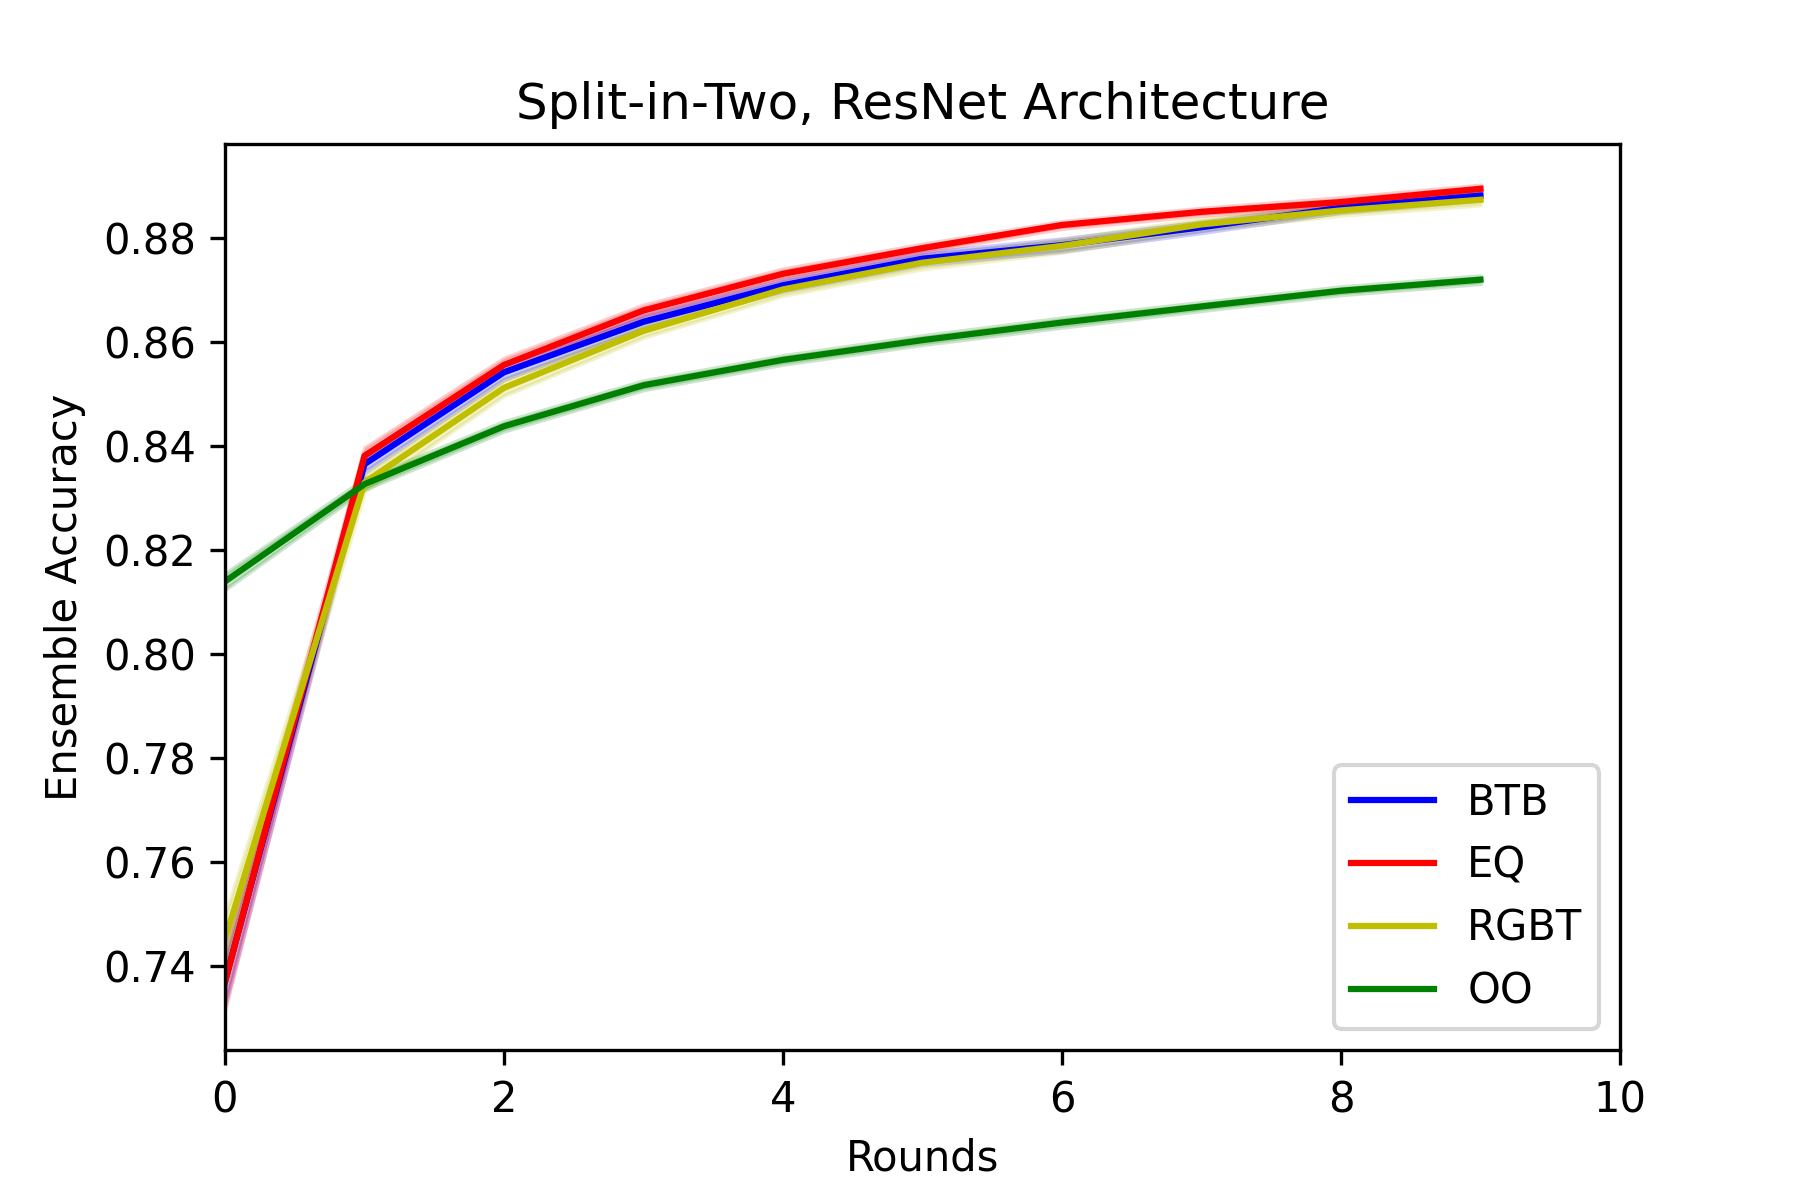}
\includegraphics[width=0.30\textwidth]{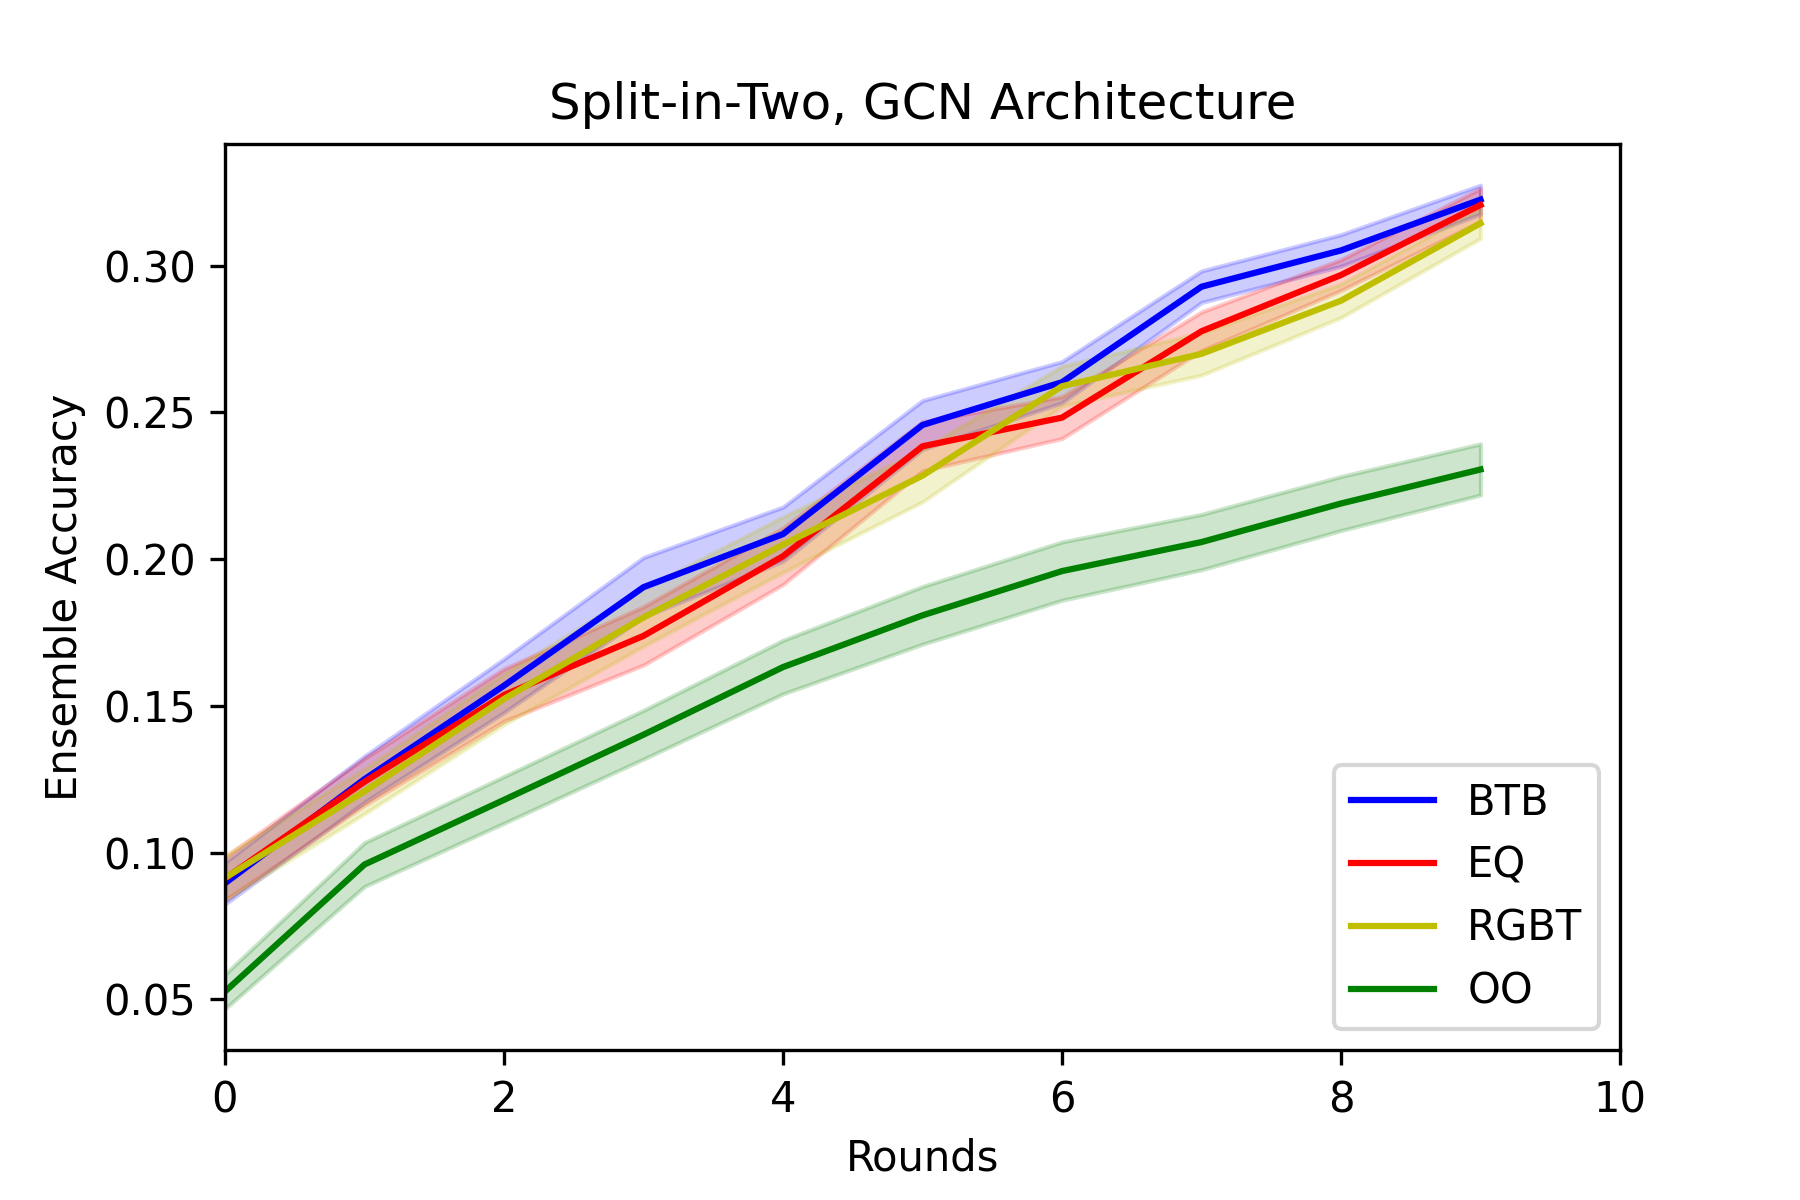}
\caption{Ensemble Accuracy $acc_{\cal E}$ on test set for 10 rounds/epochs \textbf{without pre-training}. \\ Above:  Split-in-Five $(C=2)$ grouping. Below: Split-in-Two $(C=5)$. \\ Comment: $acc_{\cal E}$ is higher for higher $C$.  Note that the reported metrics are averages over multiple random experiments, as discussed in Section~\ref{sec:results}. {\em OO} outperforms only on ResNet. Highly-coordinate policies {\em BTG, EQ} are slighly better than the moderately coordinated {\em RGBT}.}
\label{fig:ensemble_no_pretrain}
\end{figure*}

\begin{figure*}[]
\centering
\includegraphics[width=0.3\textwidth]{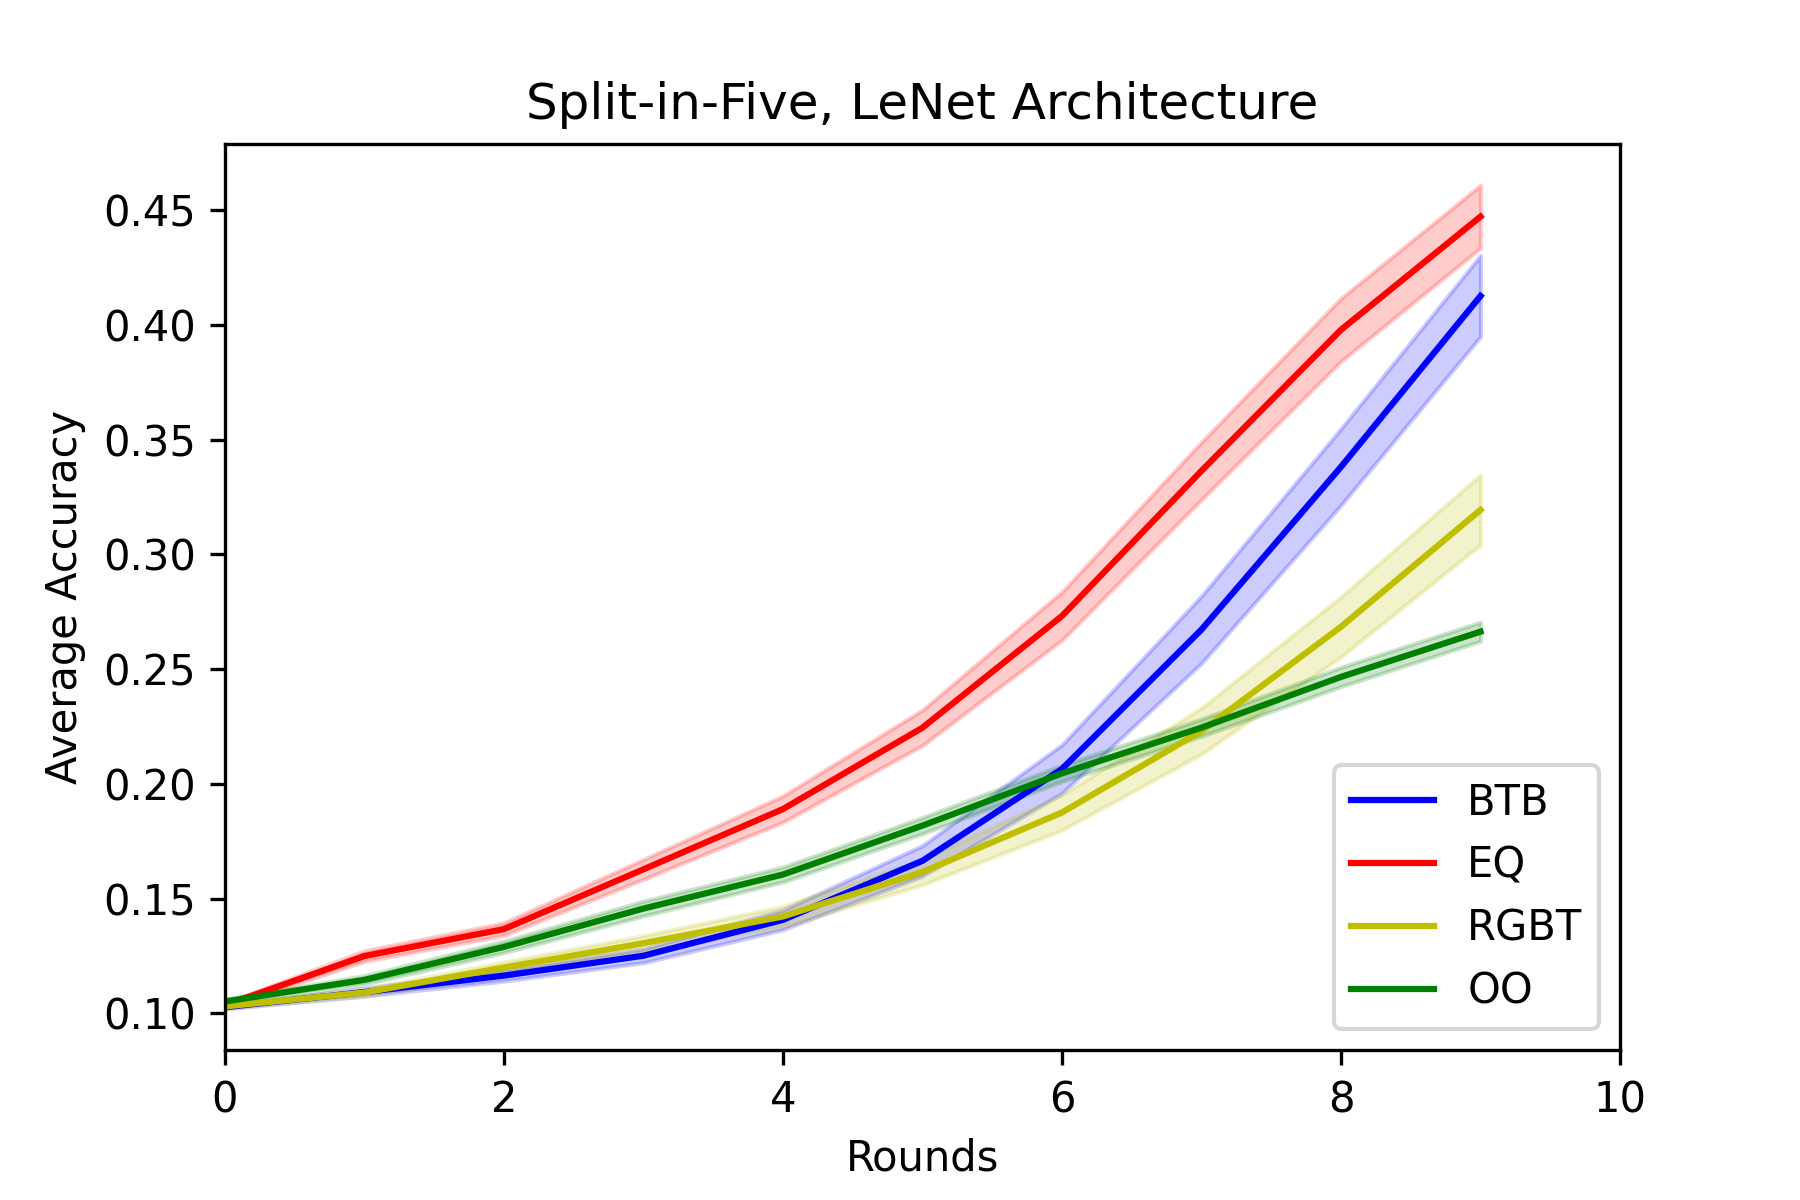}
\includegraphics[width=0.3\textwidth]{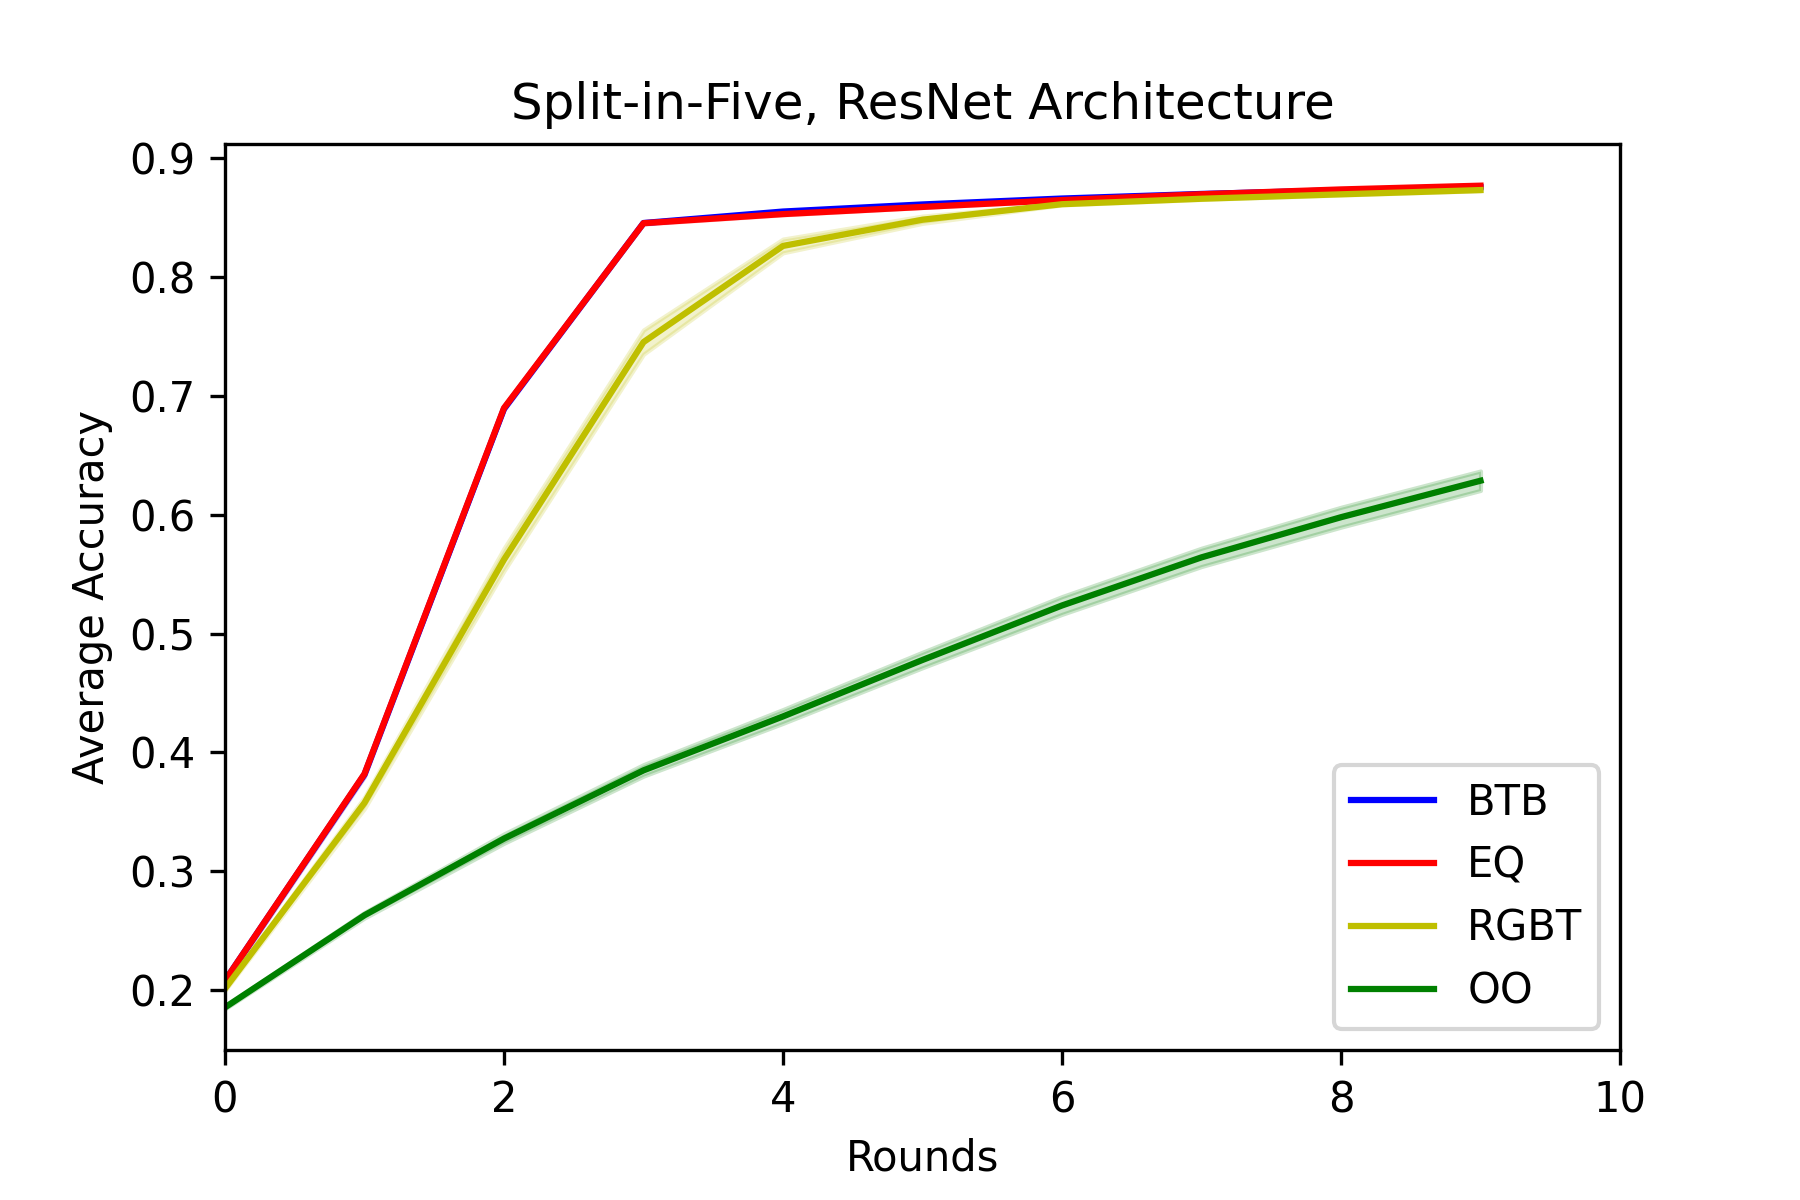}
\includegraphics[width=0.3\textwidth]{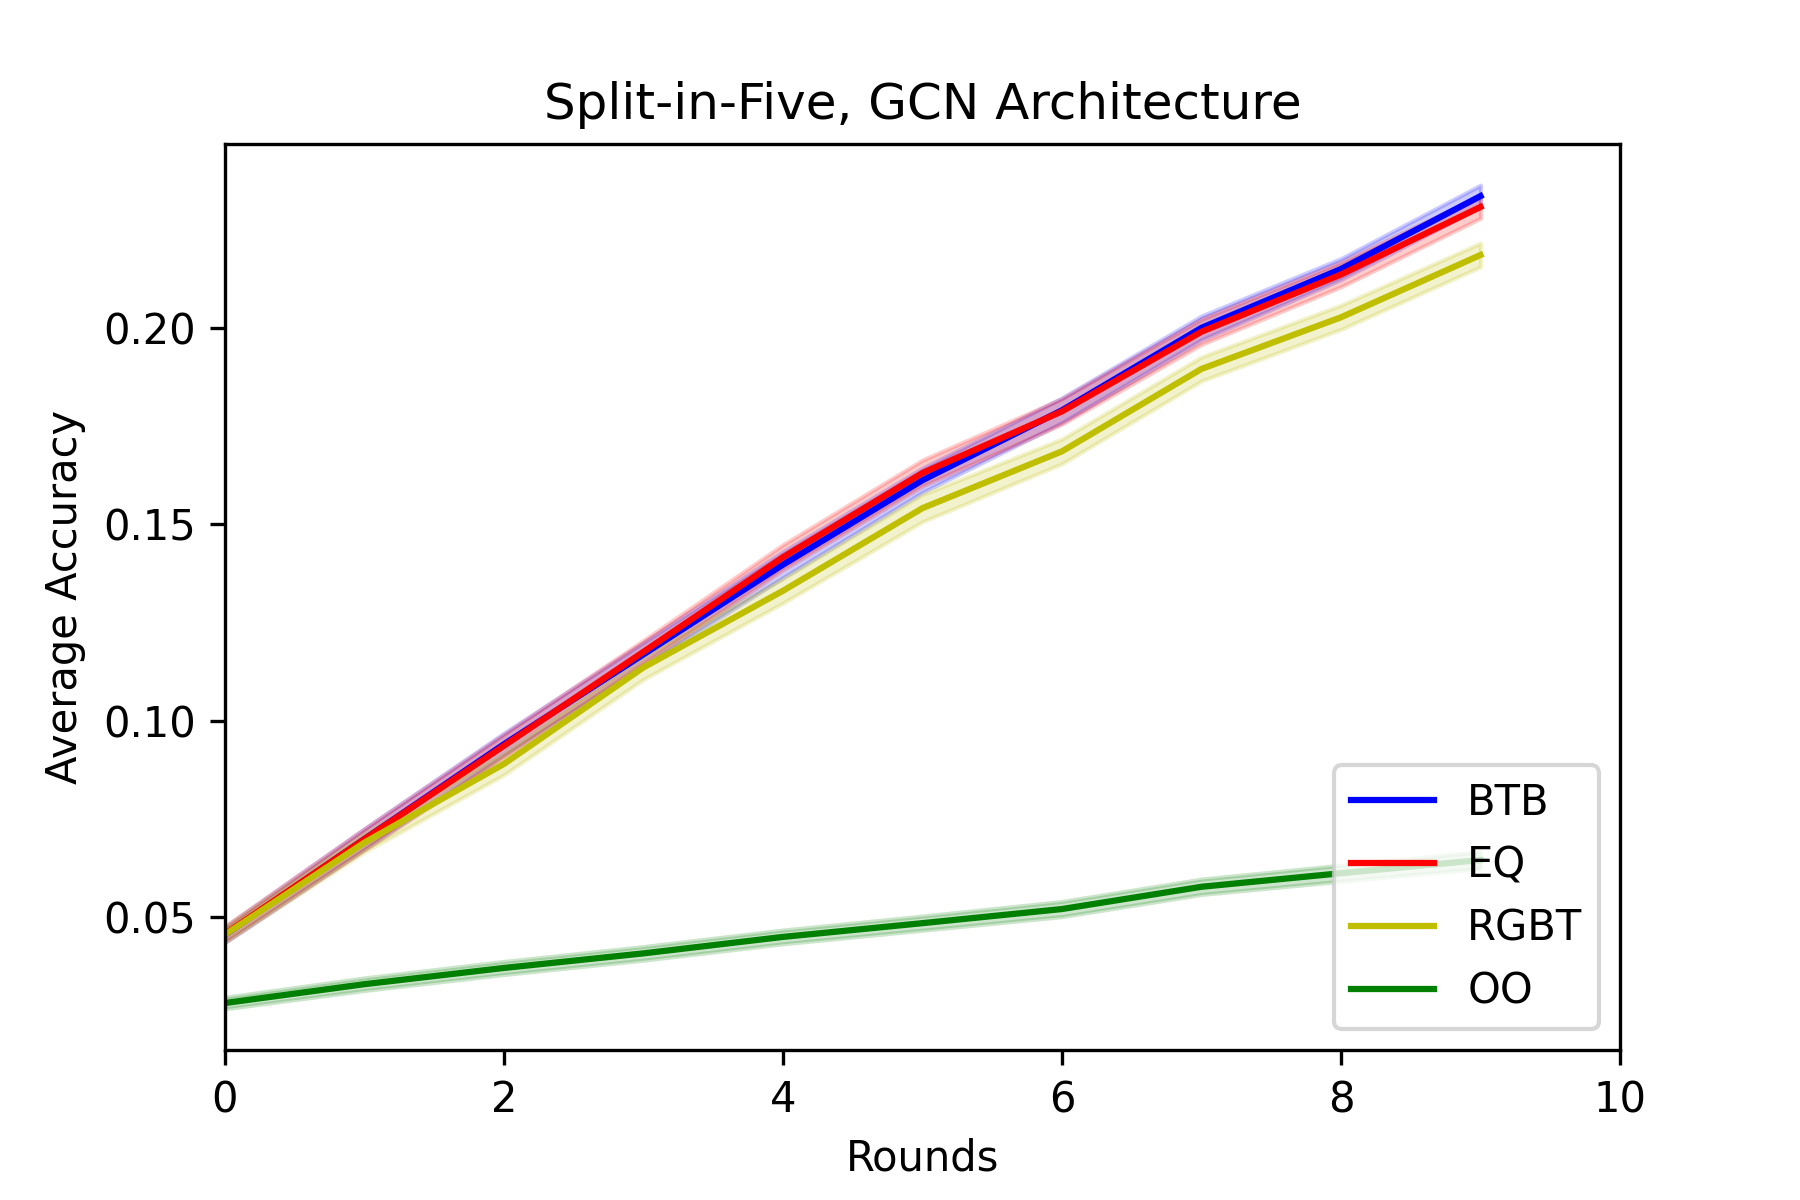}
\includegraphics[width=0.3\textwidth]{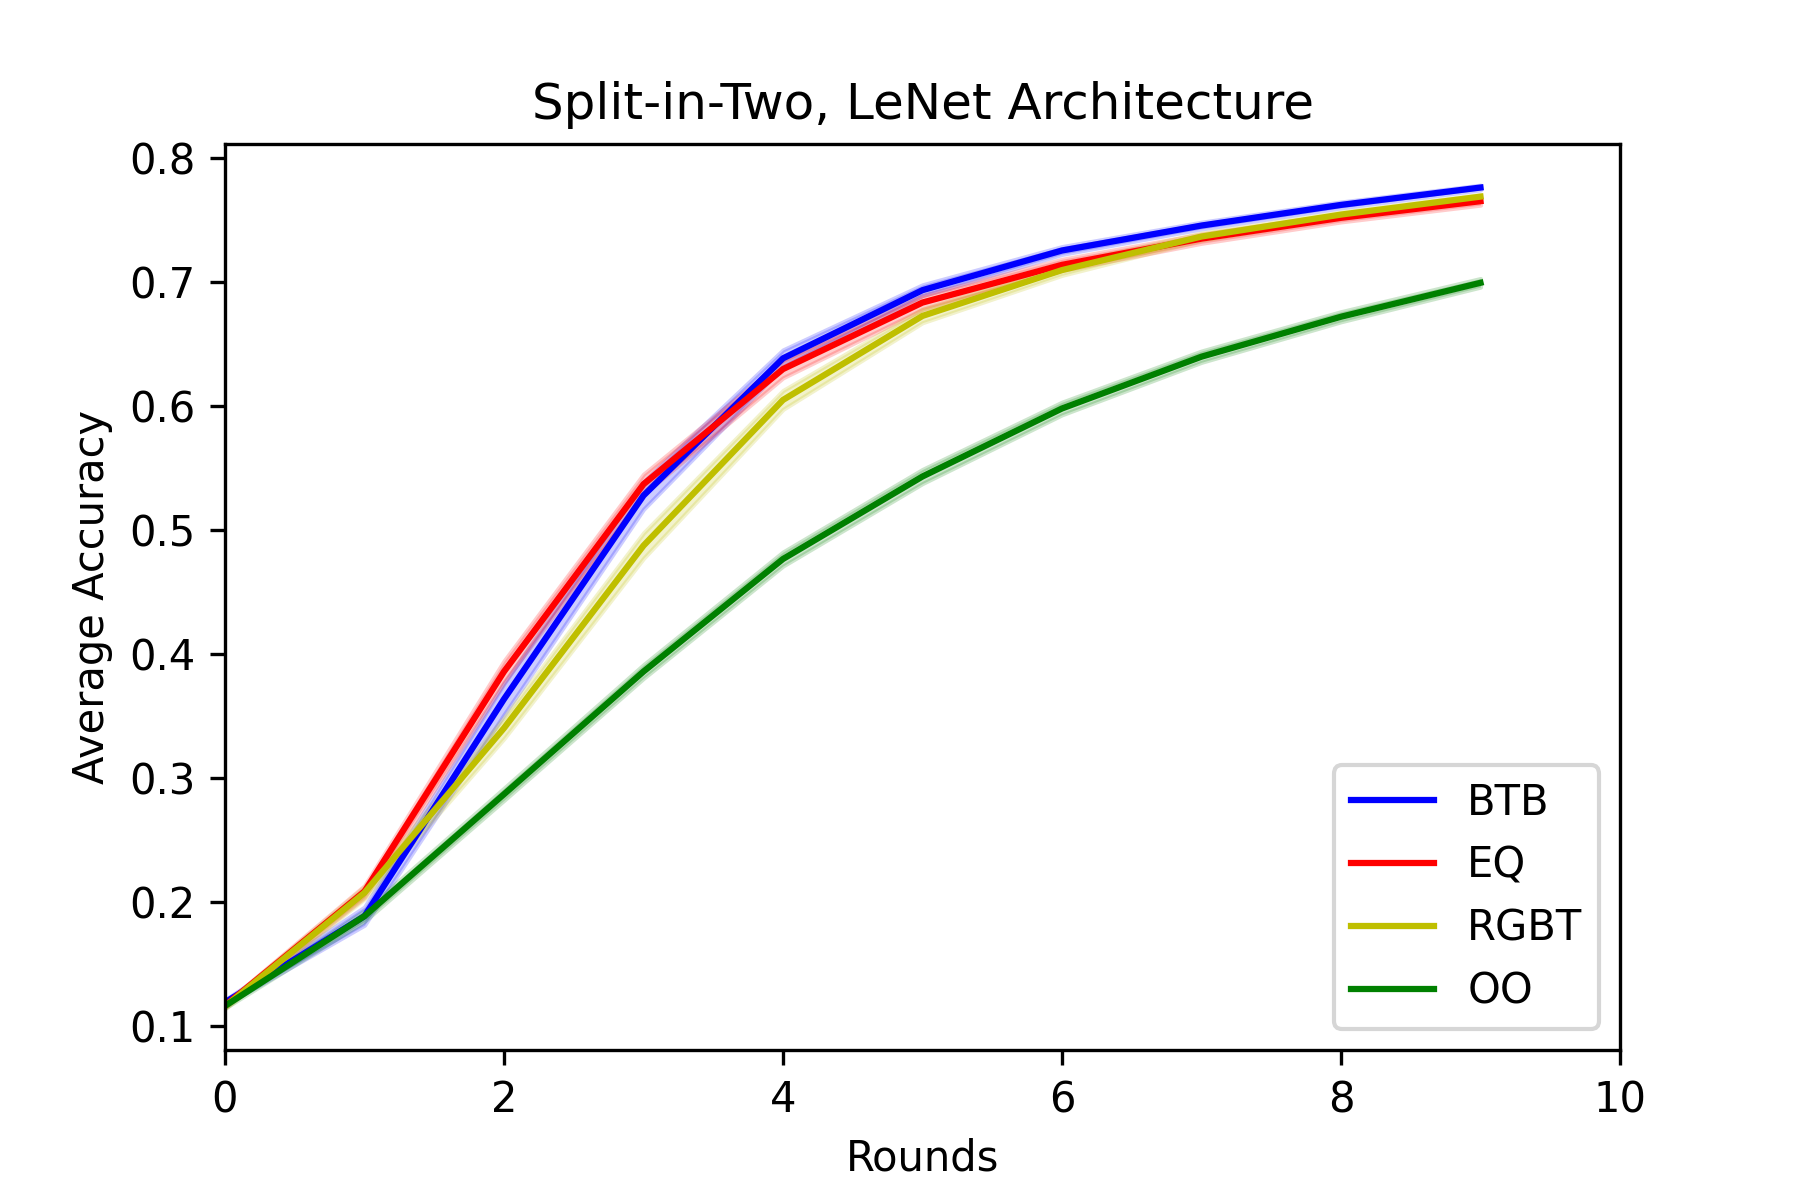}
\includegraphics[width=0.3\textwidth]{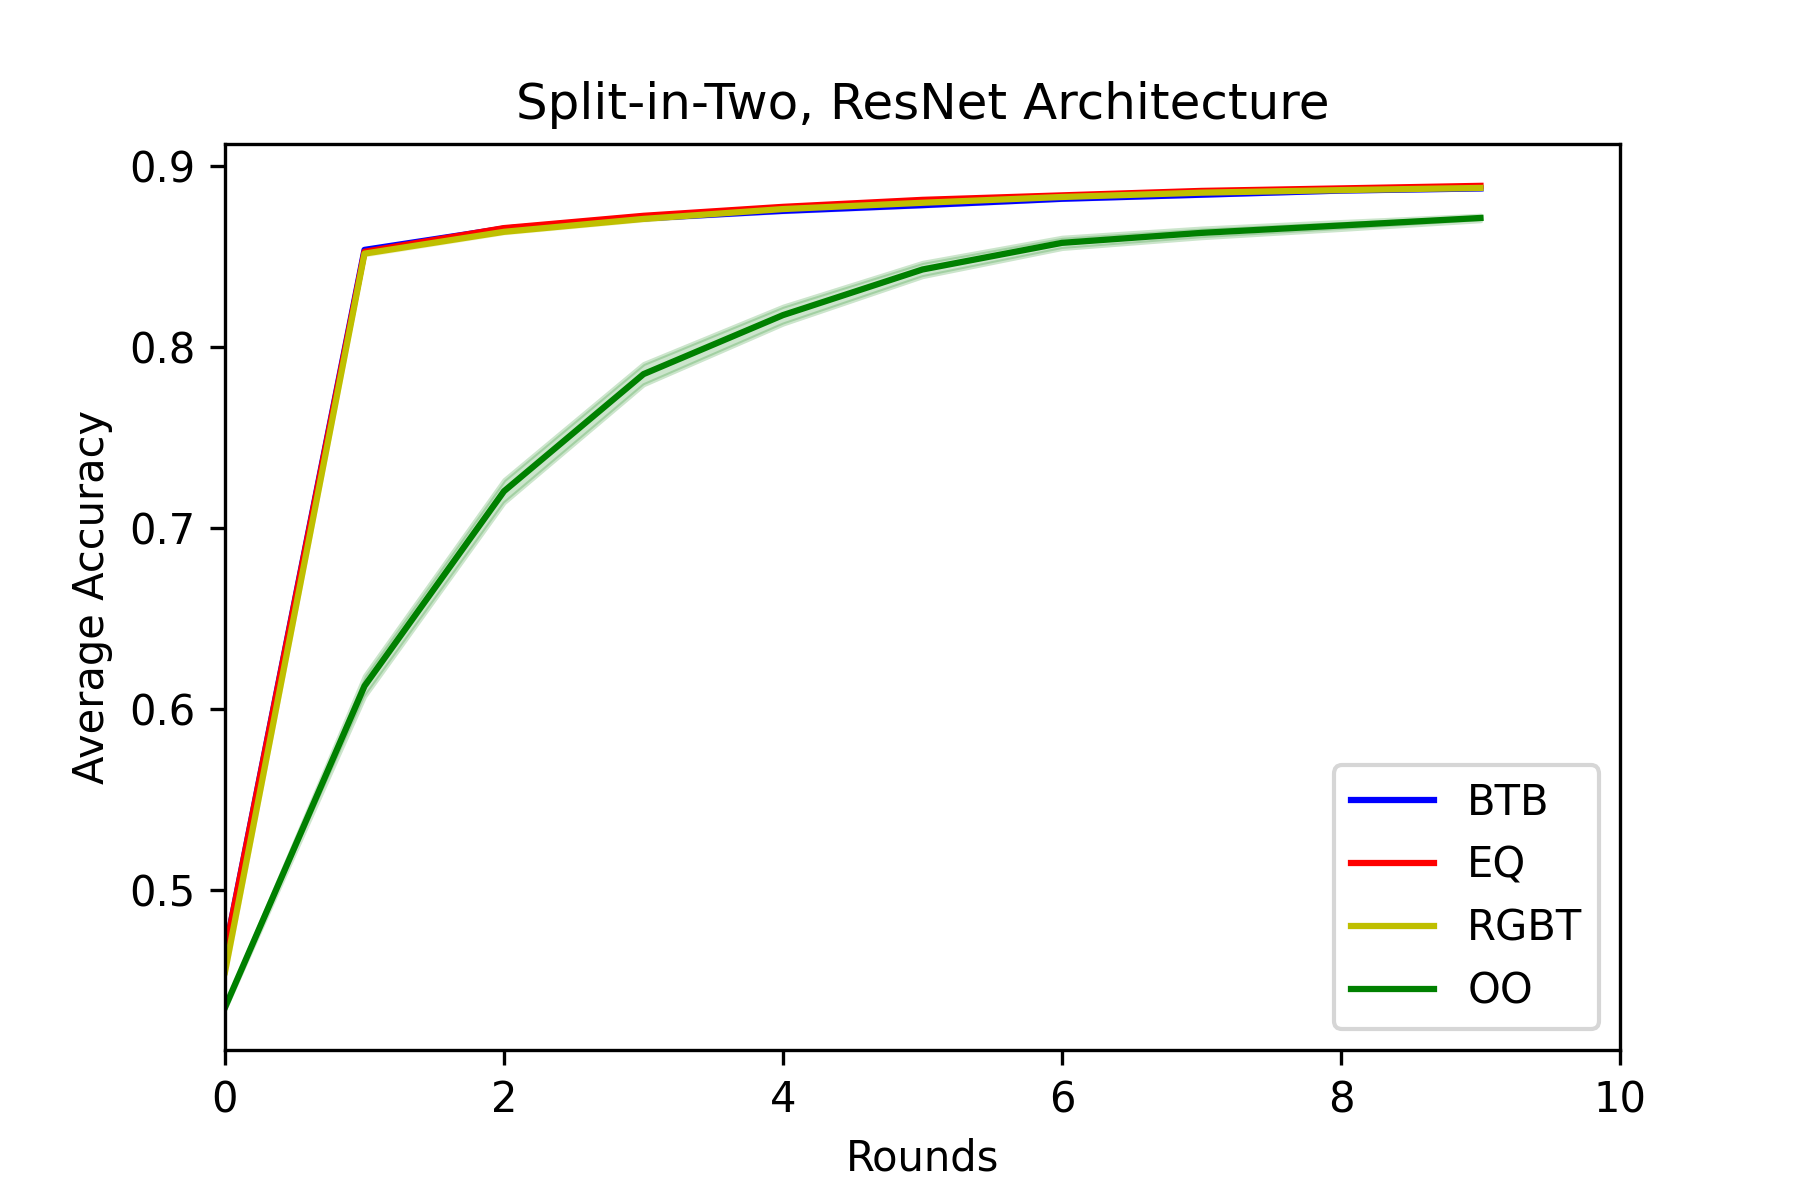}
 \includegraphics[width=0.3\textwidth]{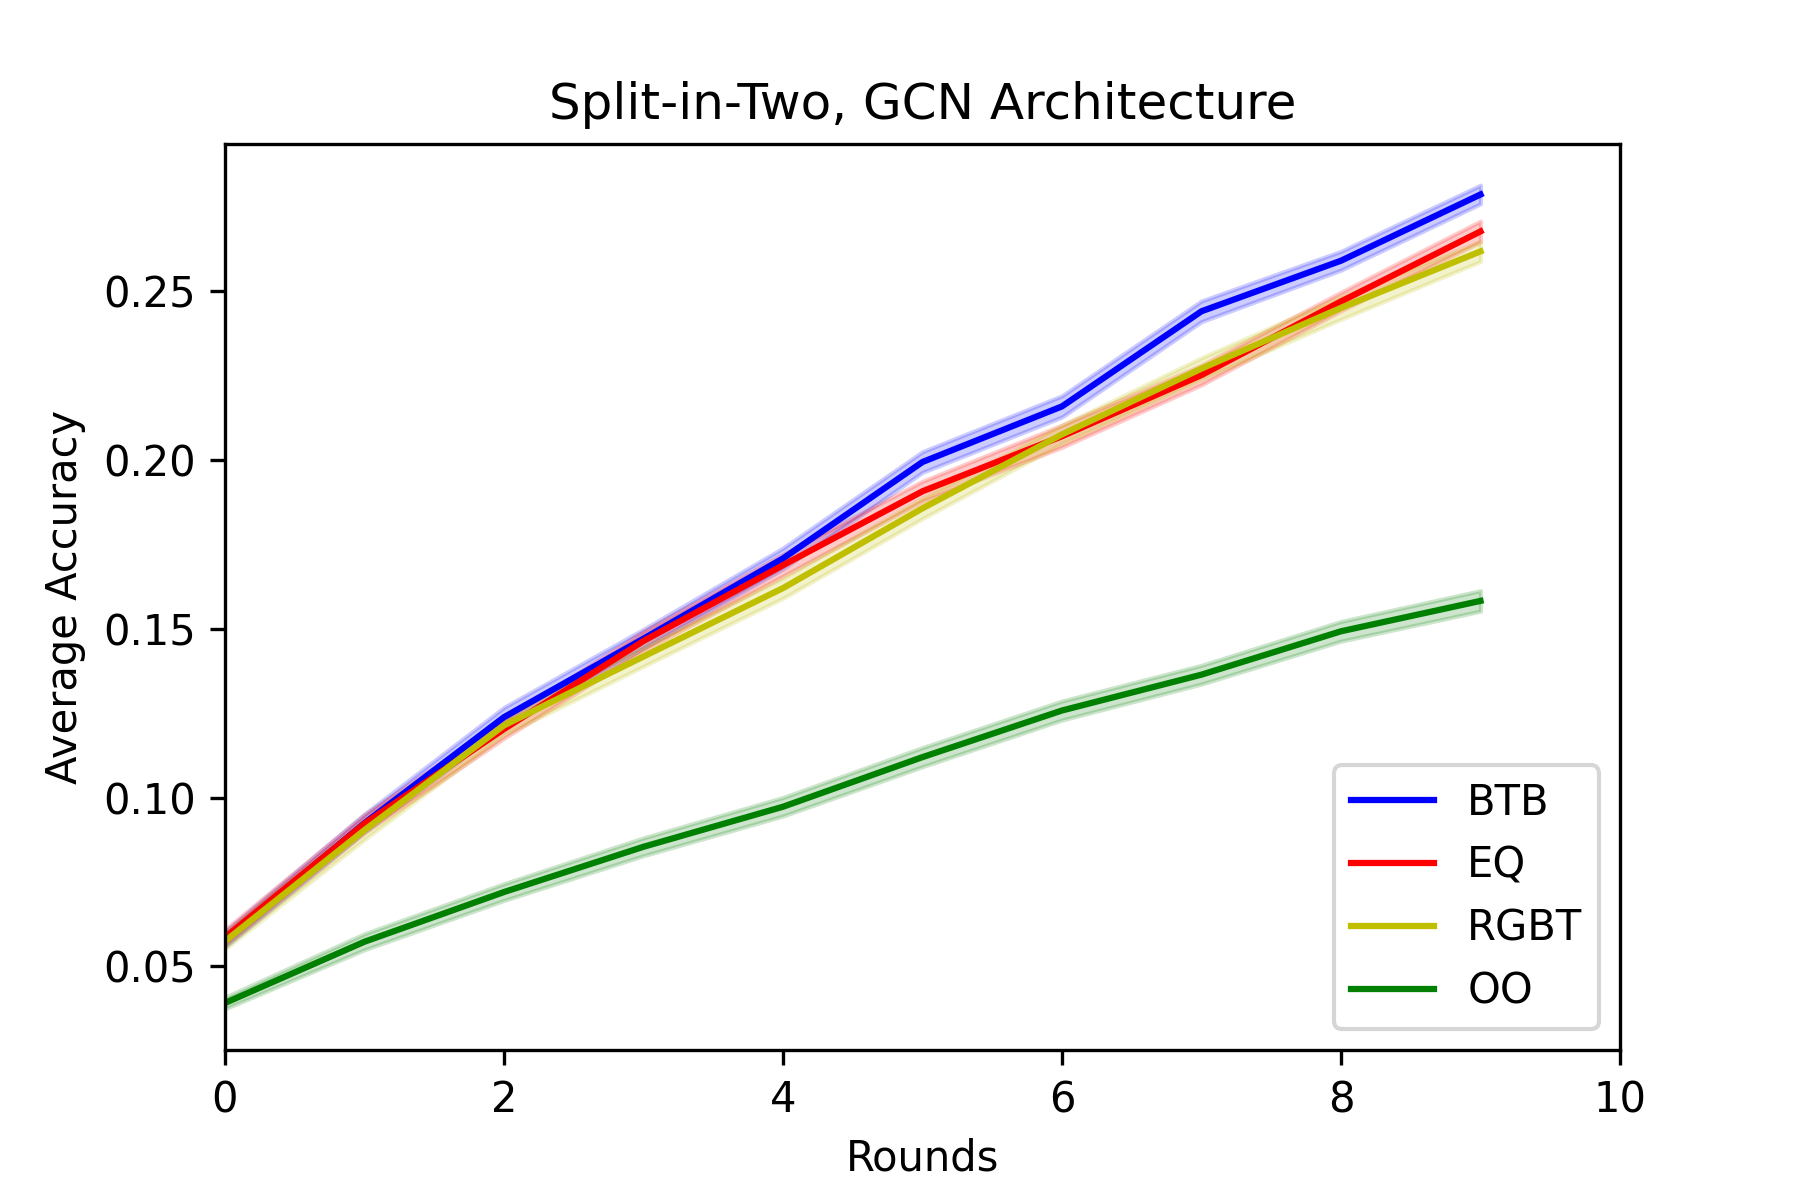}
\caption{Average Learner Accuracy $alacc_{\cal E}$ on test set for 10 rounds/epochs \textbf{without pre-training}. \\ Above:  Split-in-Five $(C=2)$ grouping. Below: Split-in-Two $(C=5)$. \\ Comment: $alacc_{\cal E}$ is higher for higher $acc_{\cal E}$. Note that the reported metrics are averages over multiple random experiments, as discussed in Section~\ref{sec:results}. Coordinated Policies (i.e. {\em BTB} and {\em EQ}) outperform other policies.}
\label{fig:average_no_pretrain} 
\end{figure*}

% % Forward: Supplementary
\begin{figure*}[h]
\centering
\includegraphics[width=0.32\textwidth]{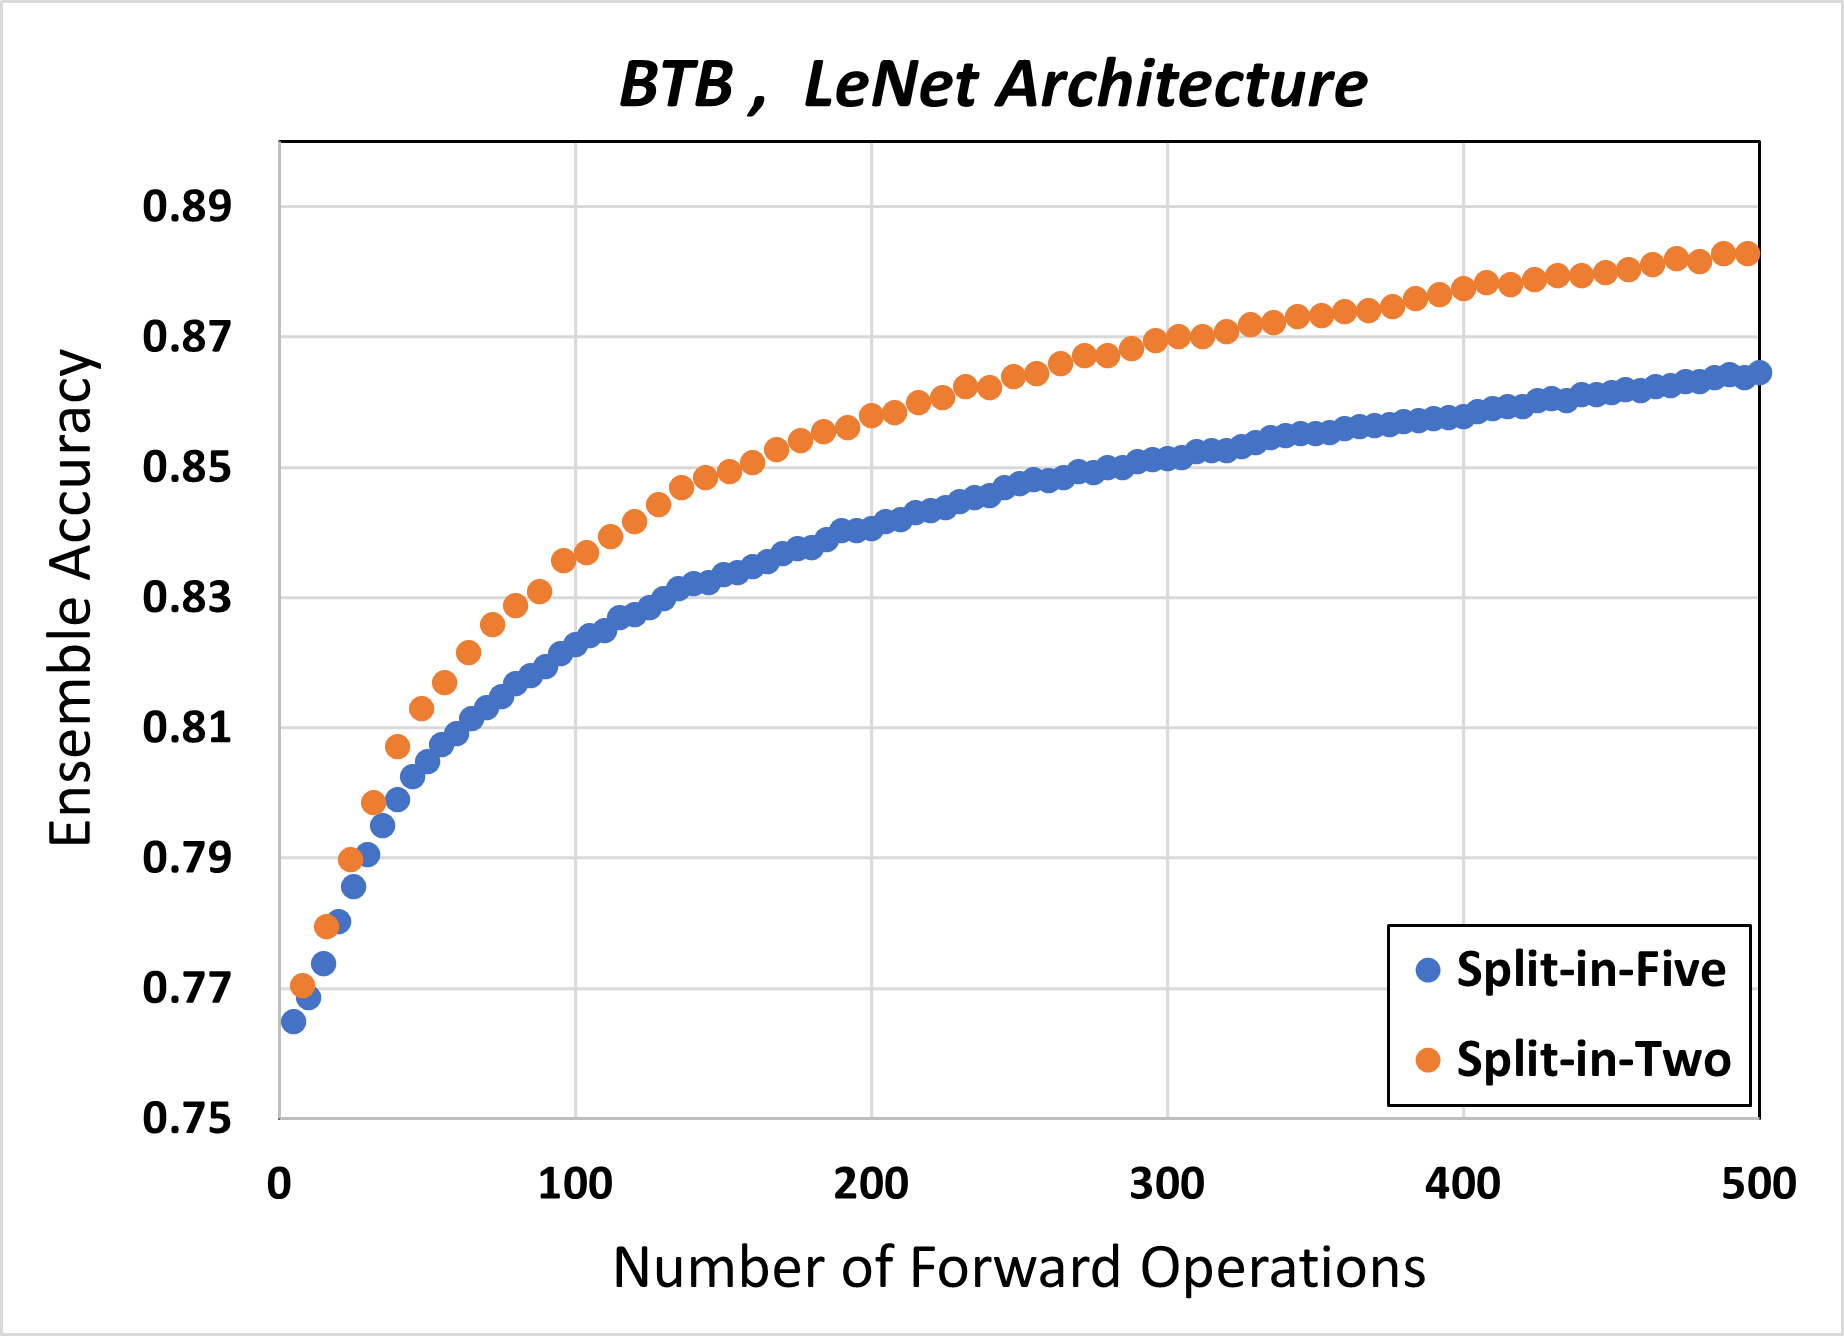}
\includegraphics[width=0.32\textwidth]{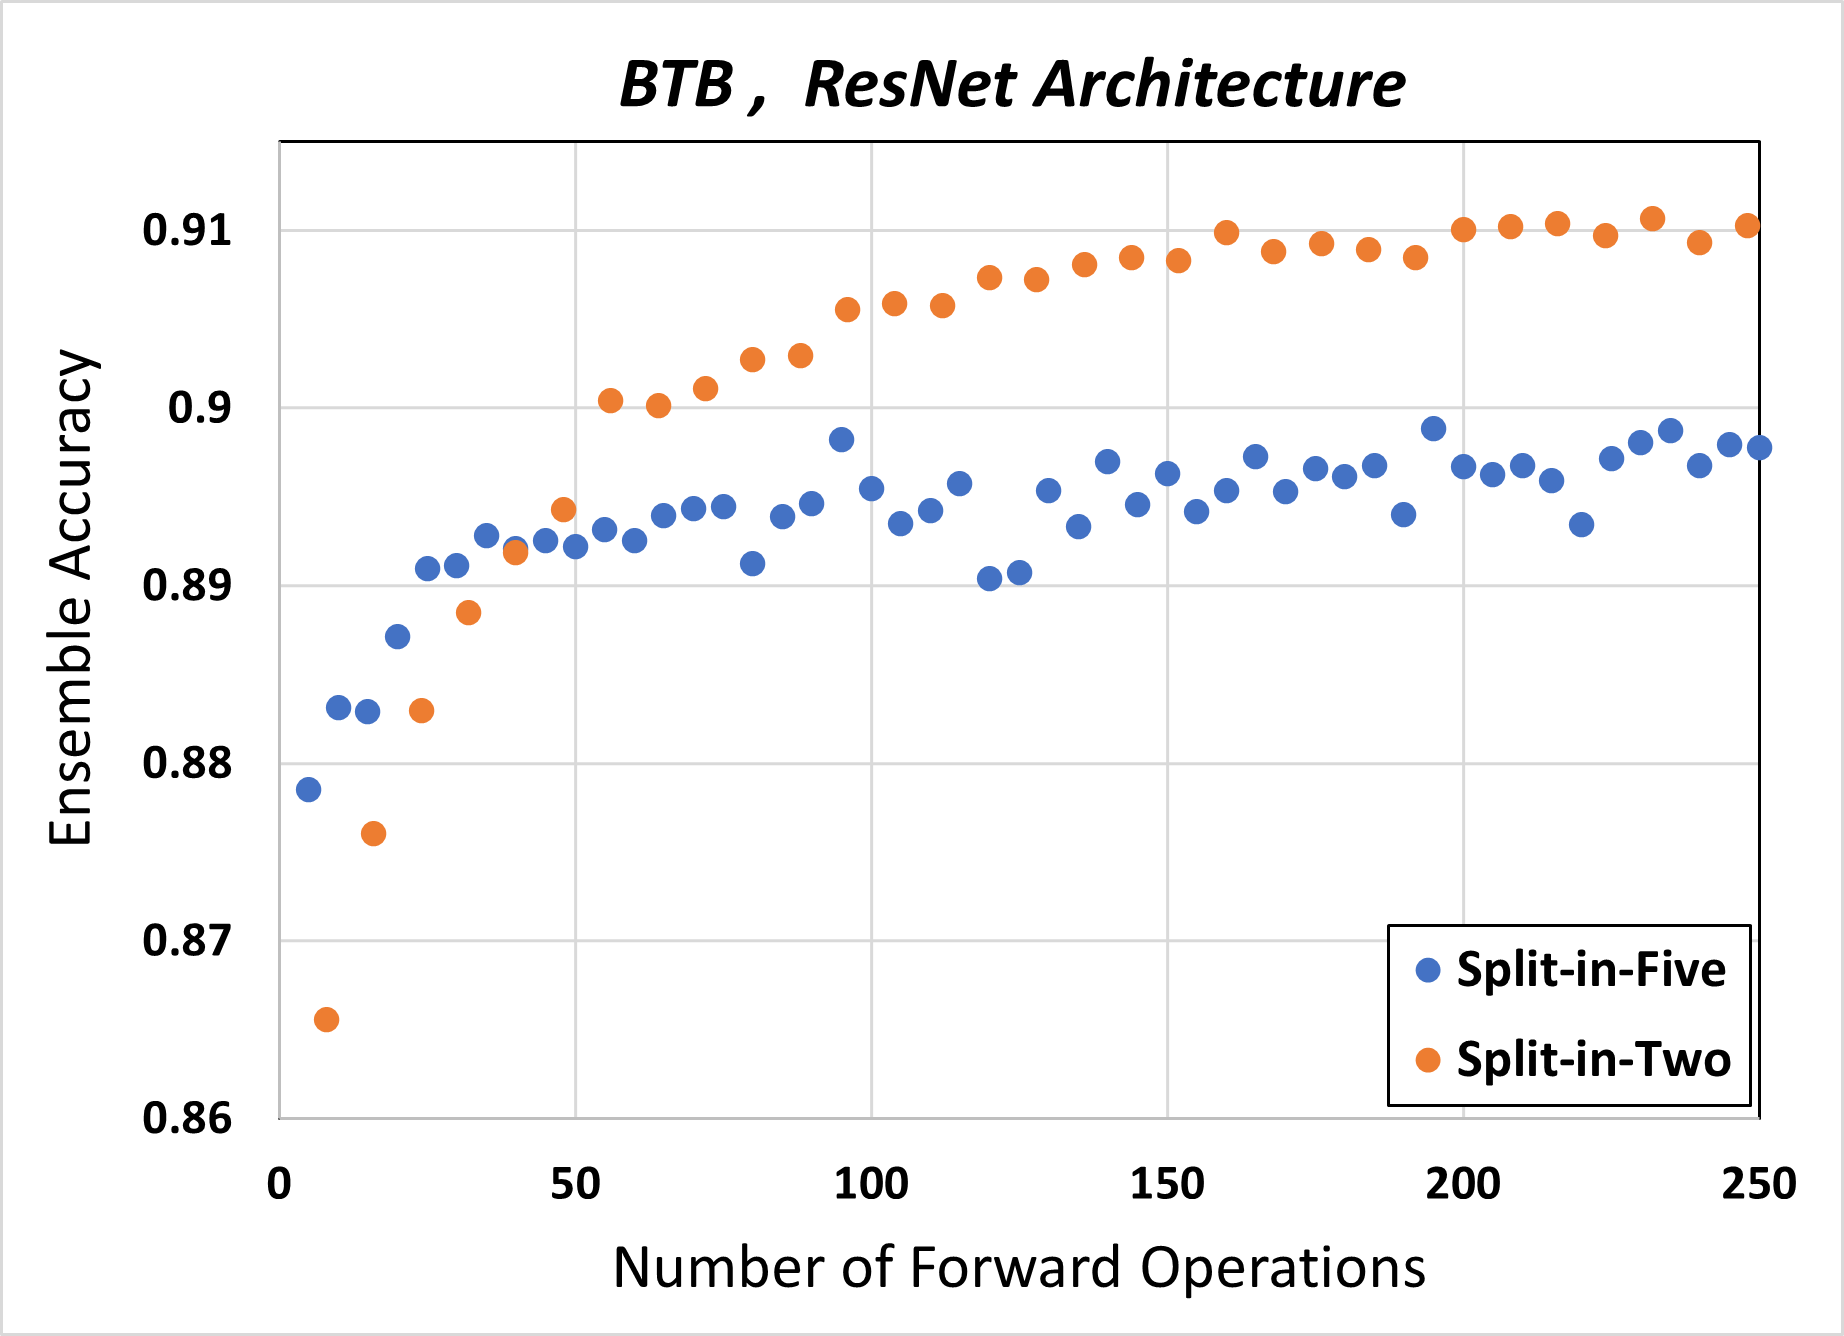}
\includegraphics[width=0.32\textwidth]{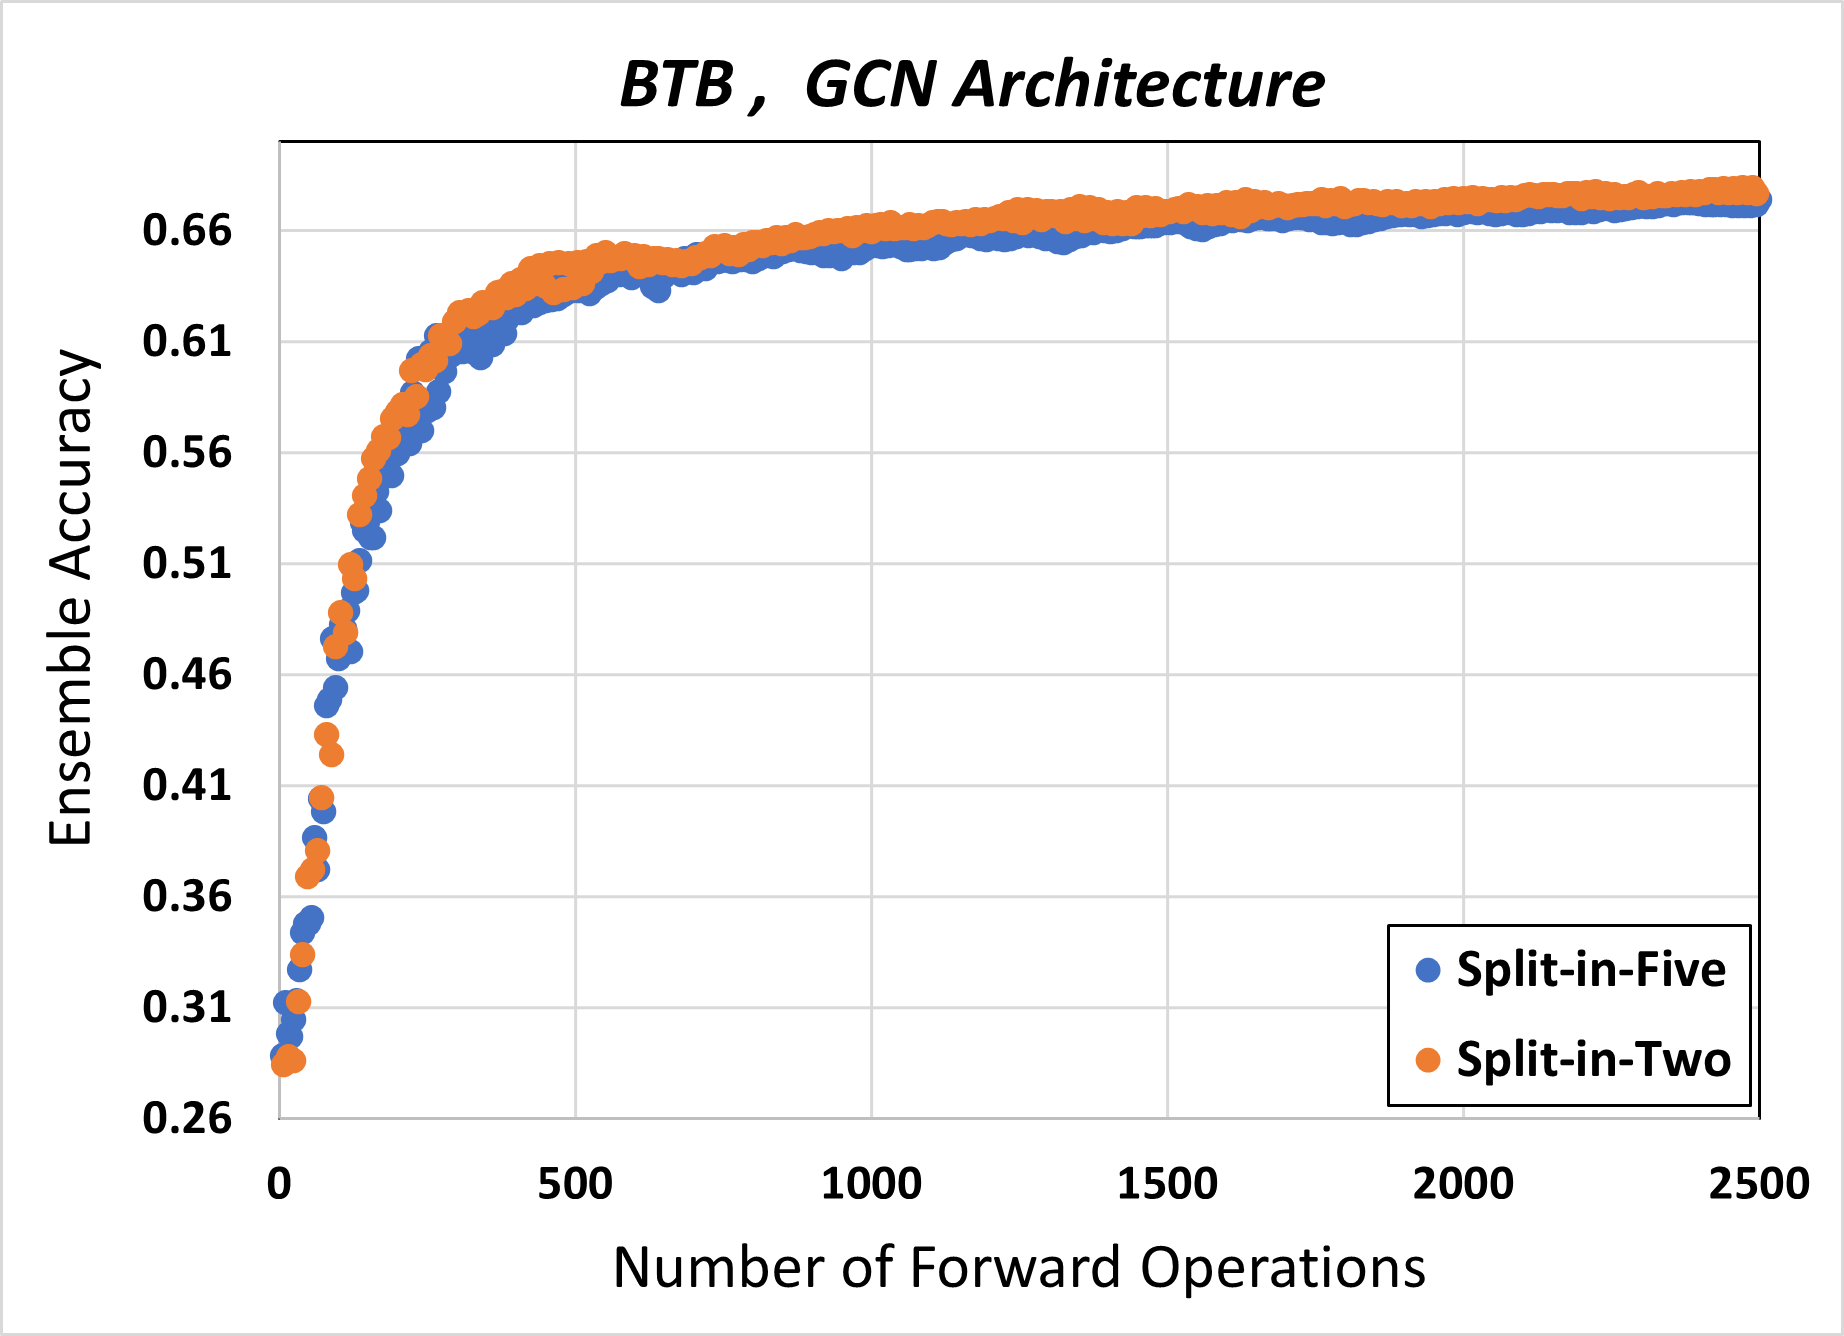}

\includegraphics[width=0.32\textwidth]{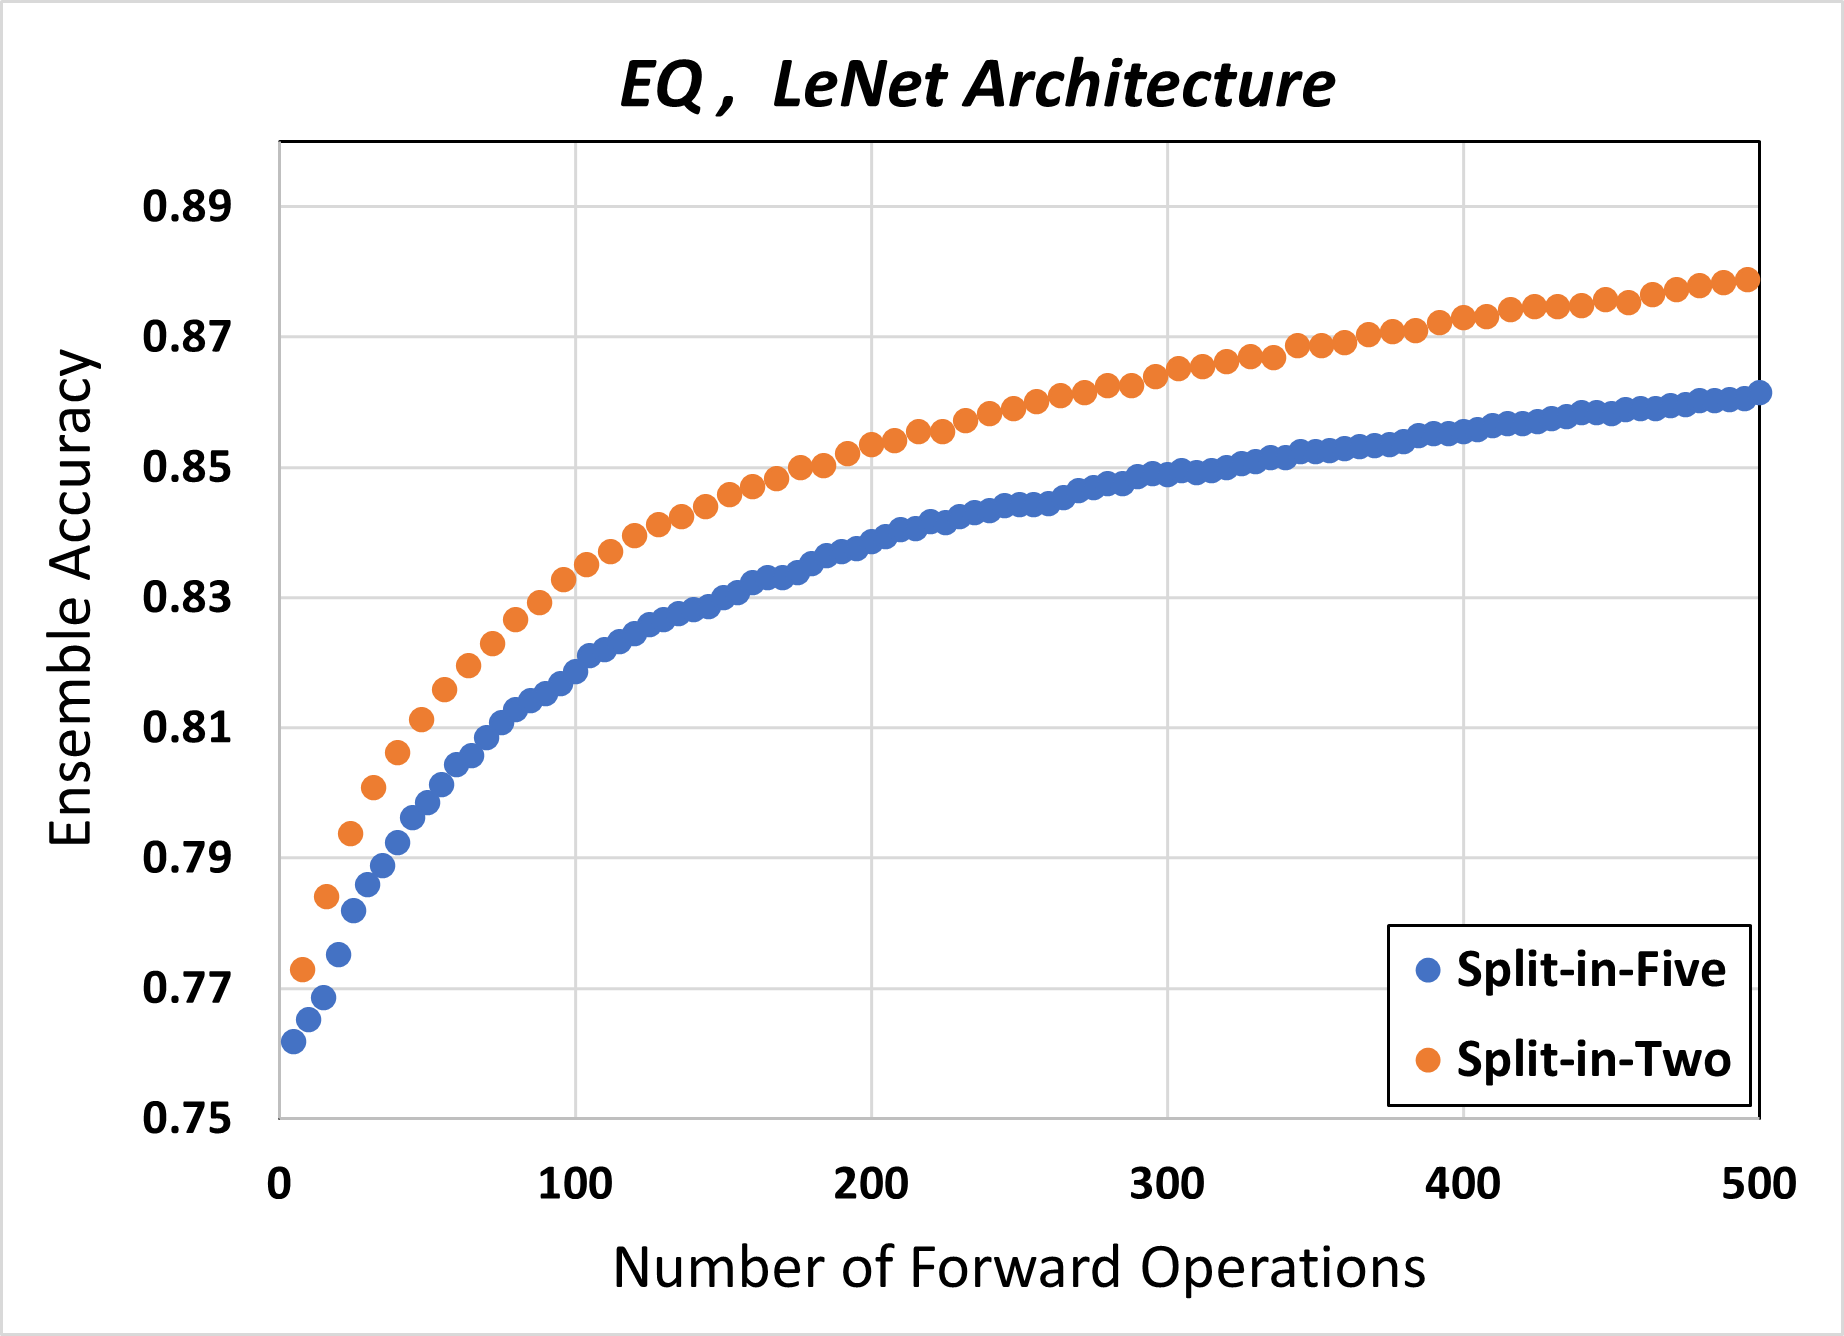}
\includegraphics[width=0.32\textwidth]{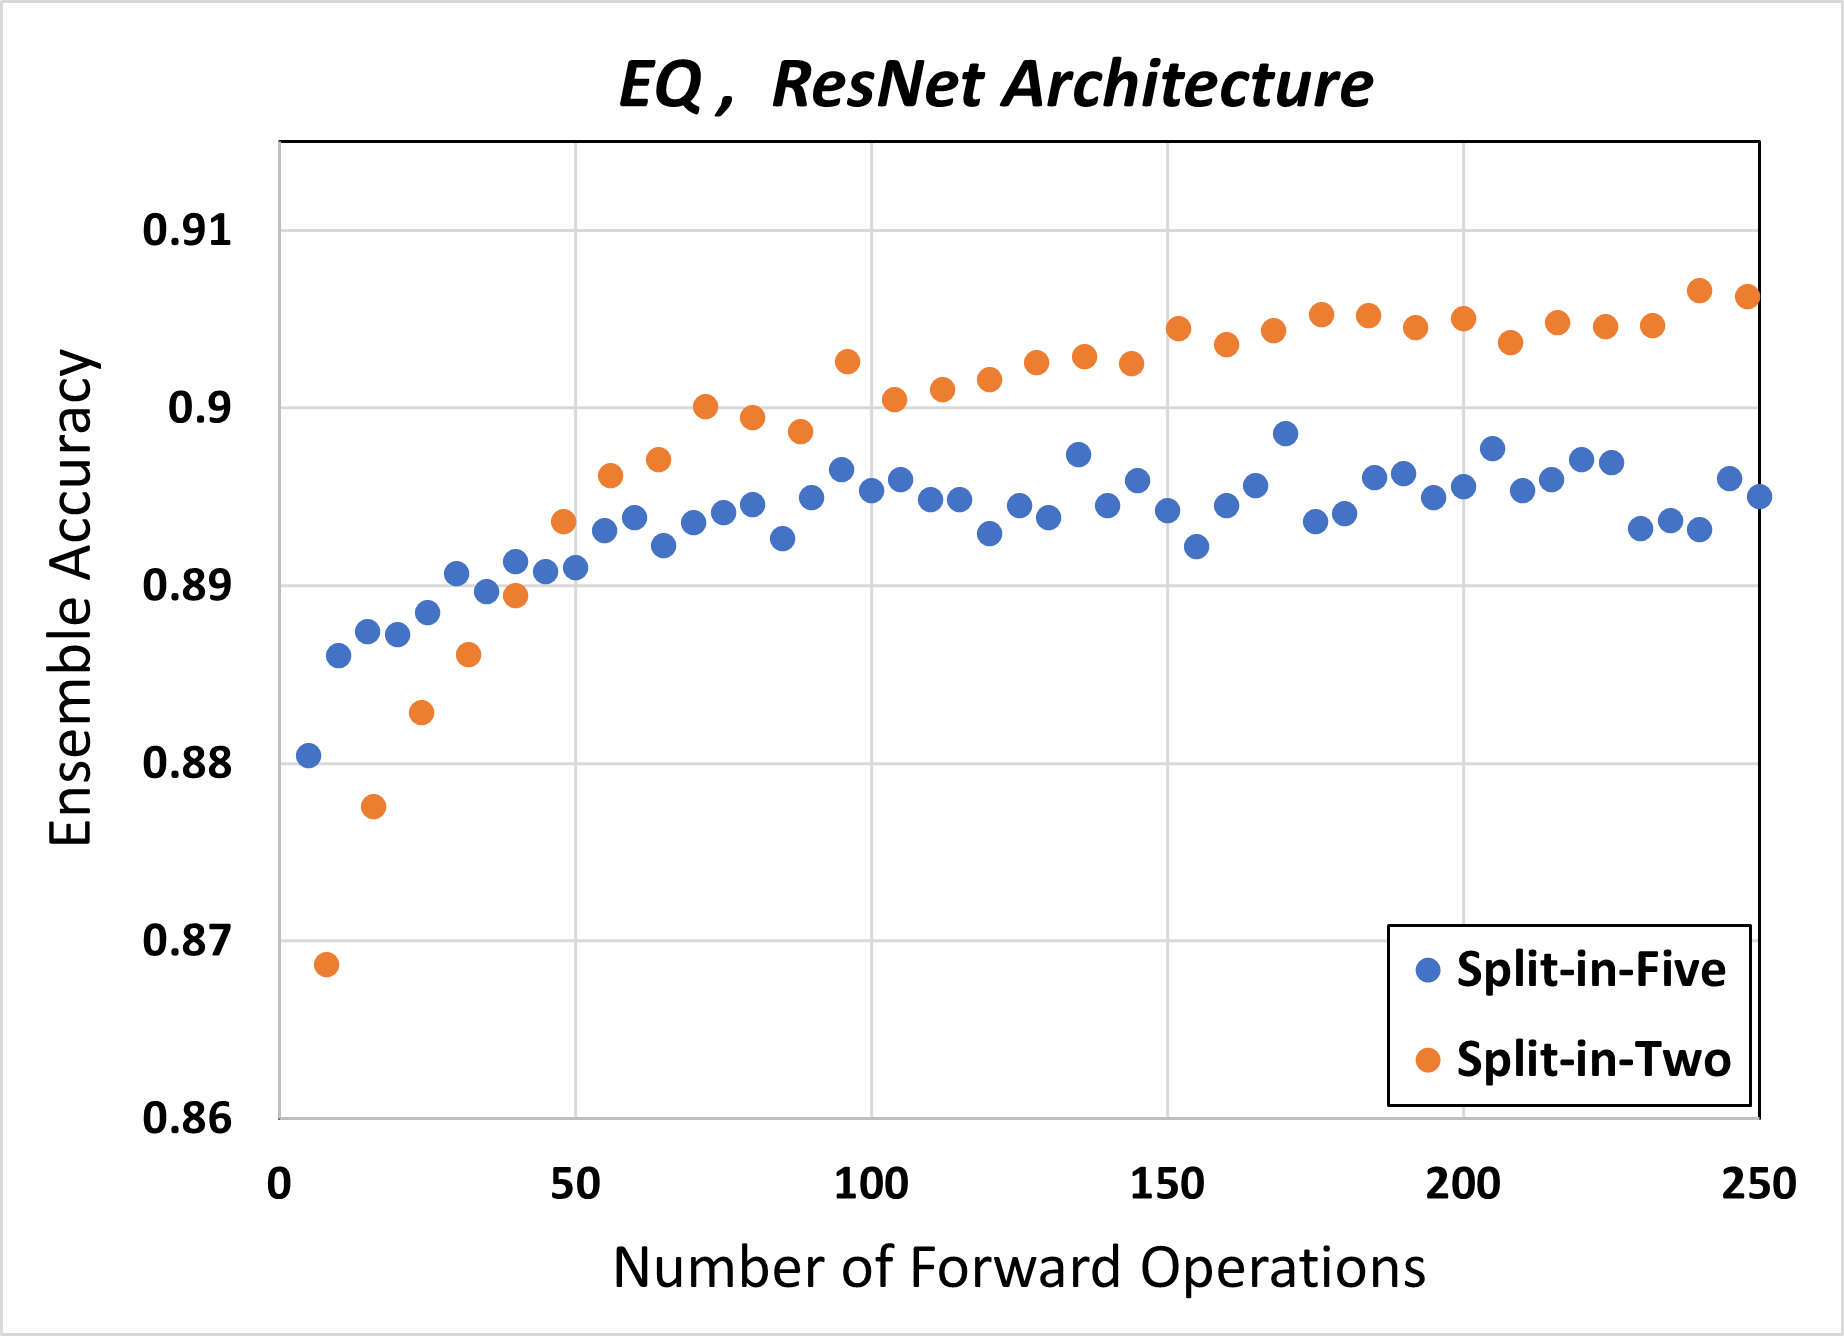}
\includegraphics[width=0.32\textwidth]{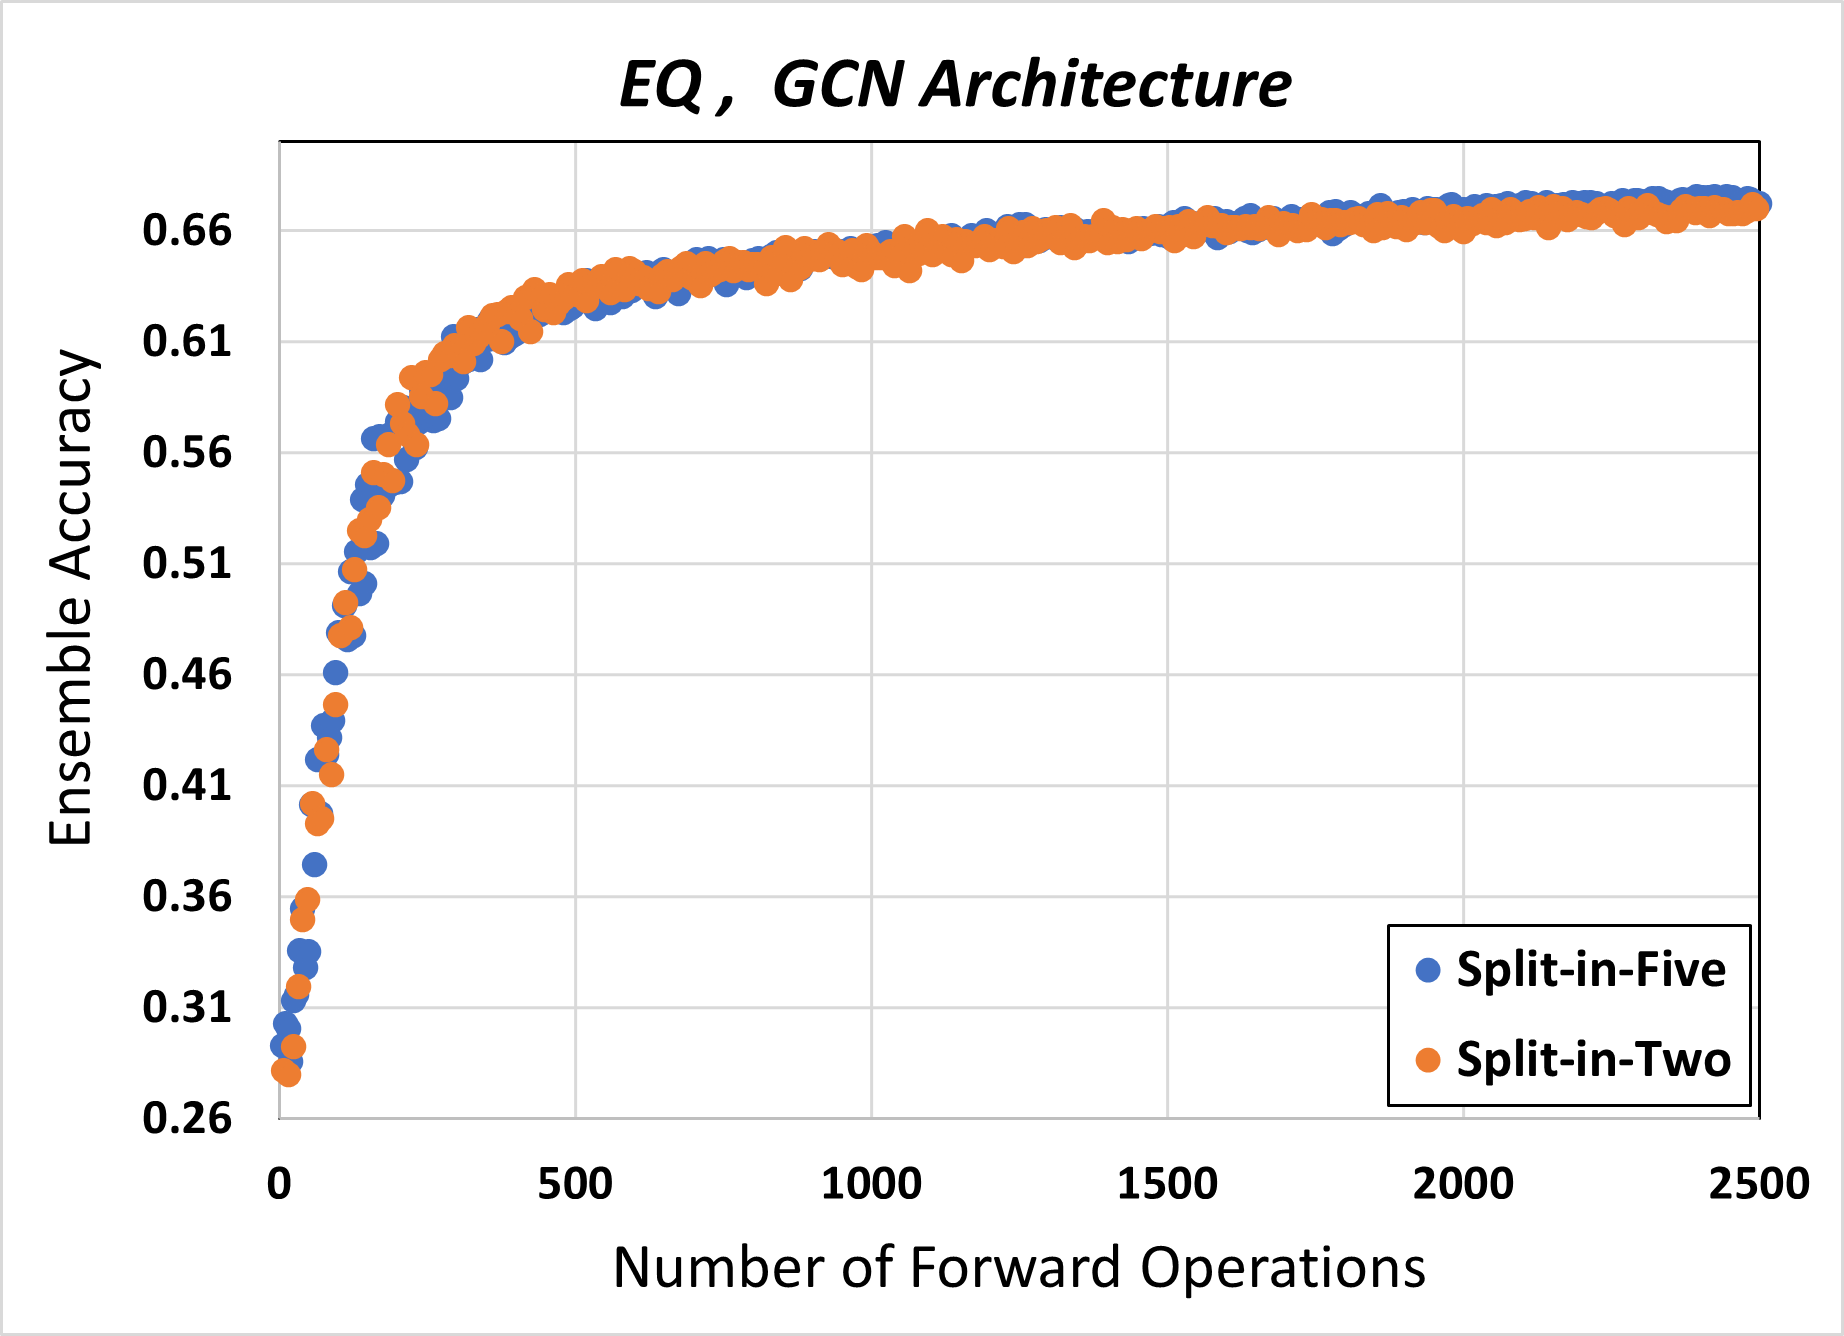}

\includegraphics[width=0.32\textwidth]{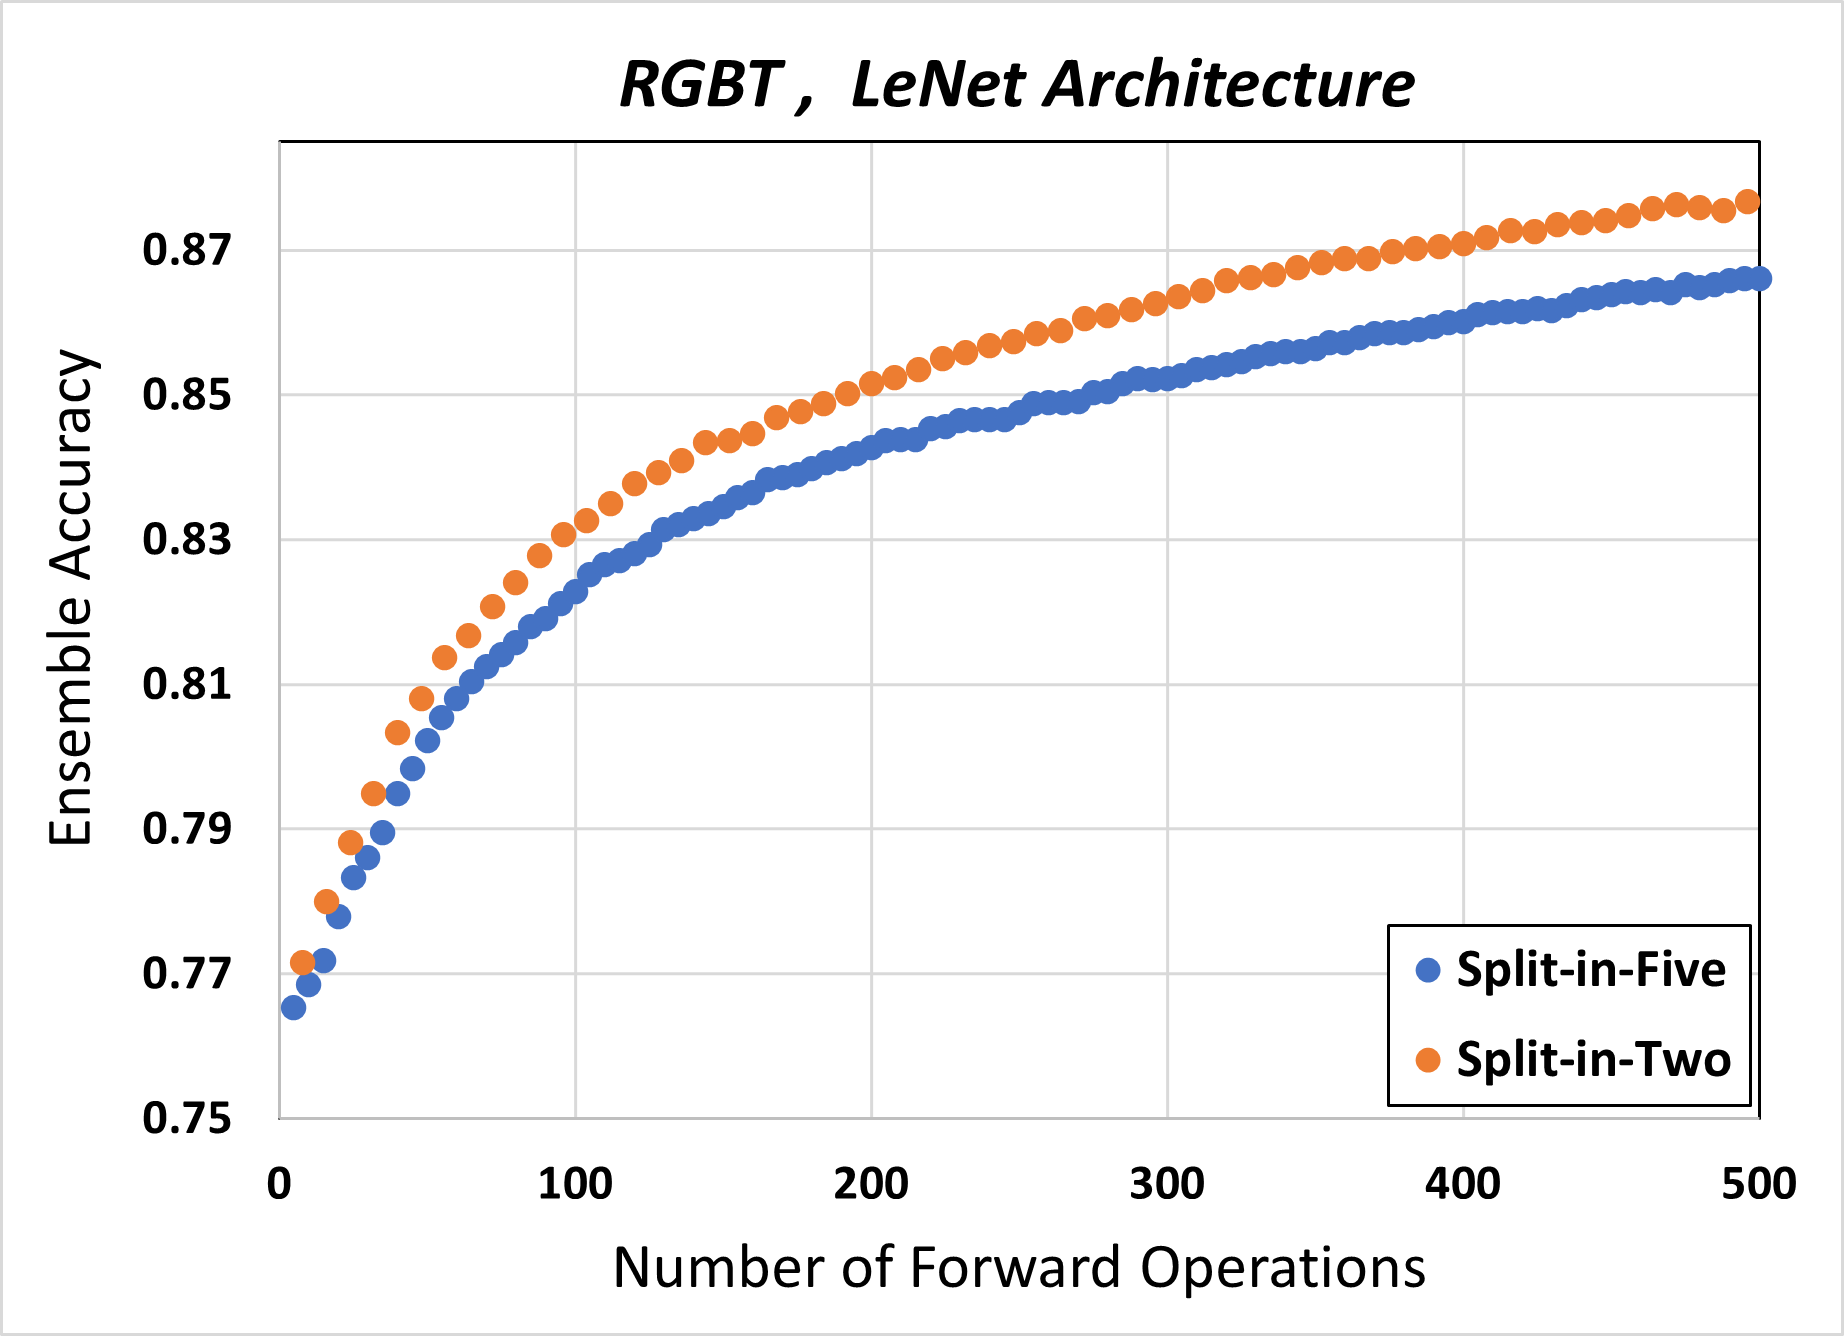}
\includegraphics[width=0.32\textwidth]{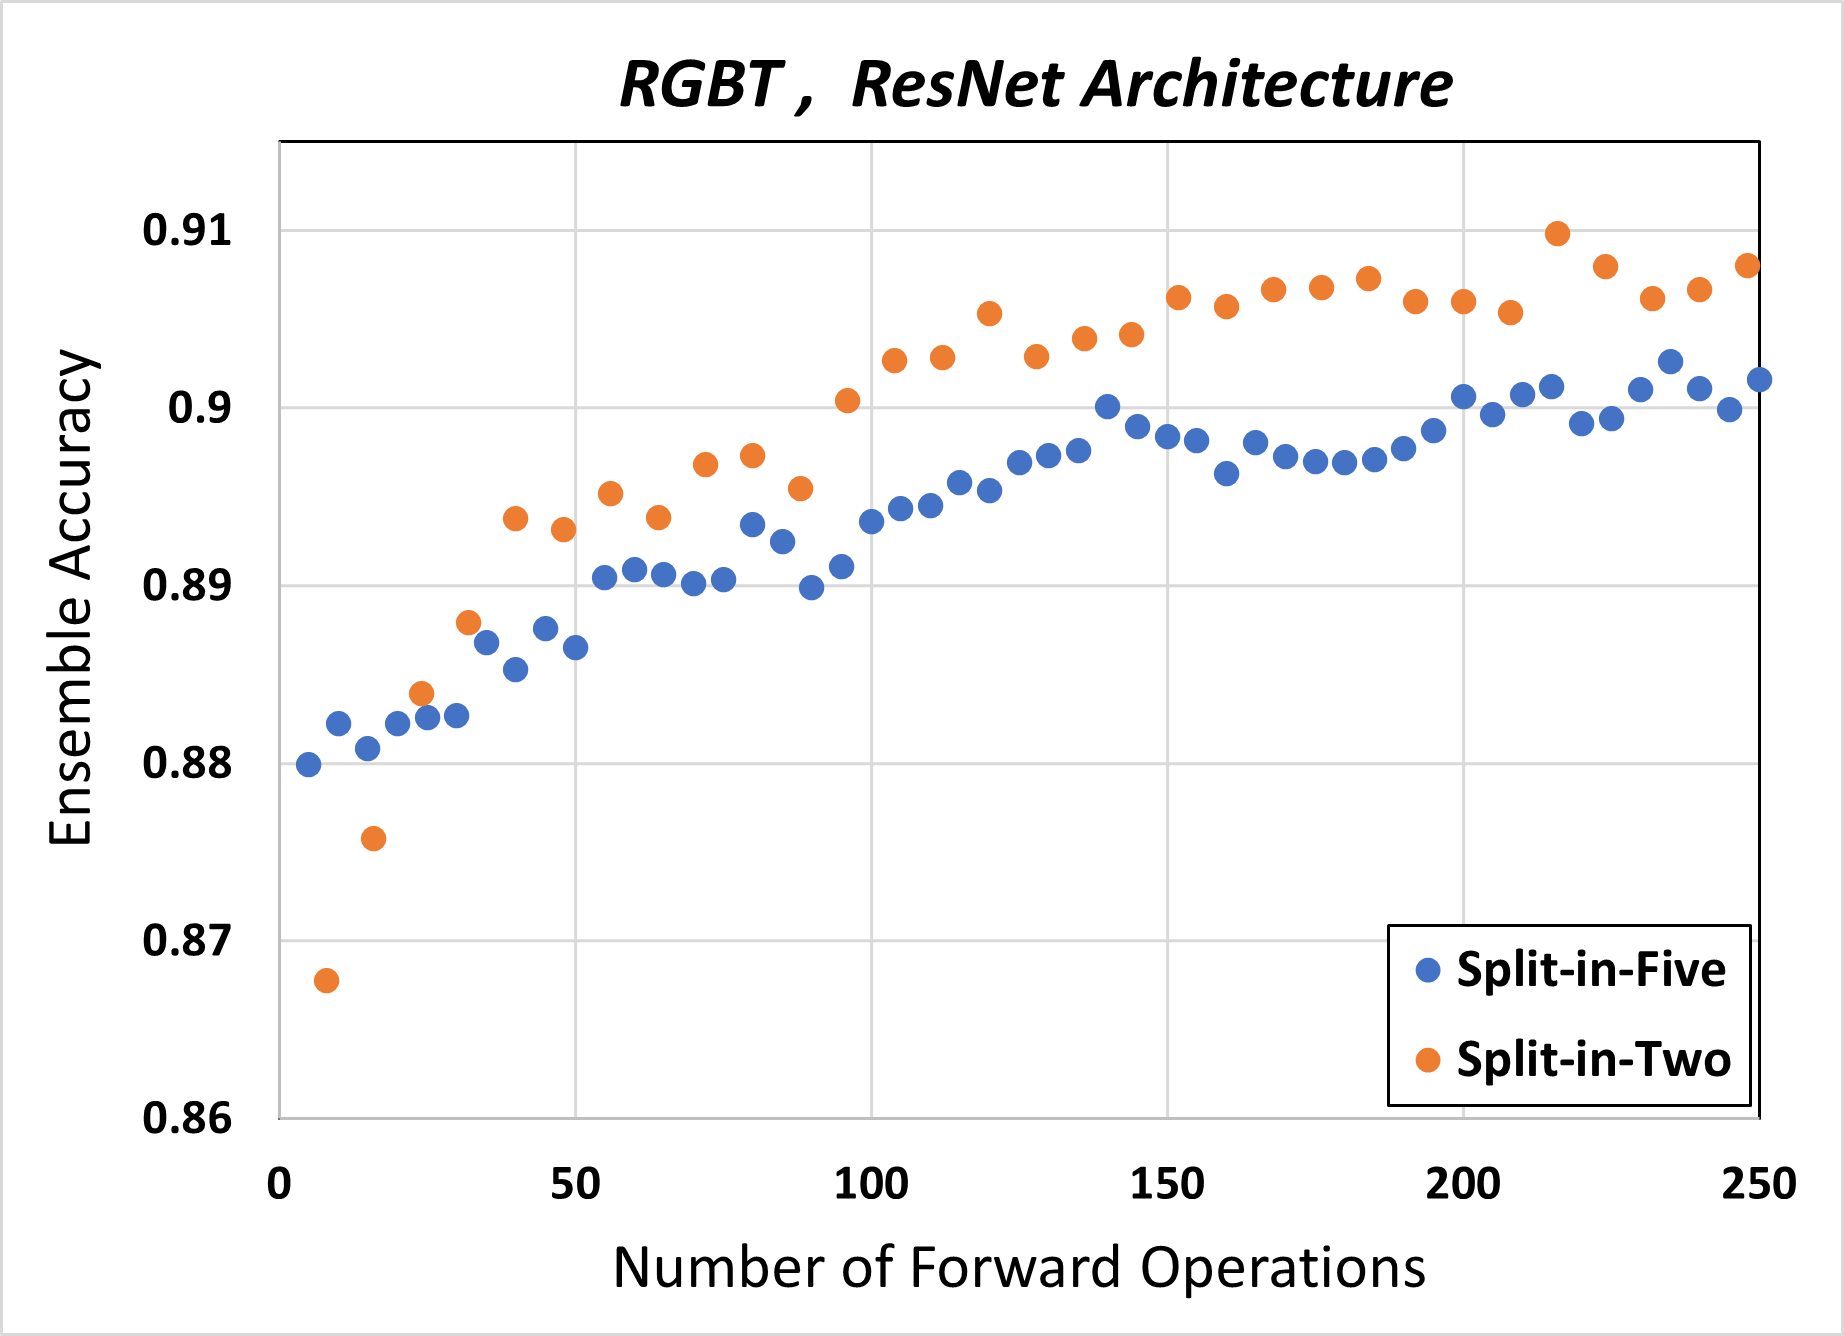}
\includegraphics[width=0.32\textwidth]{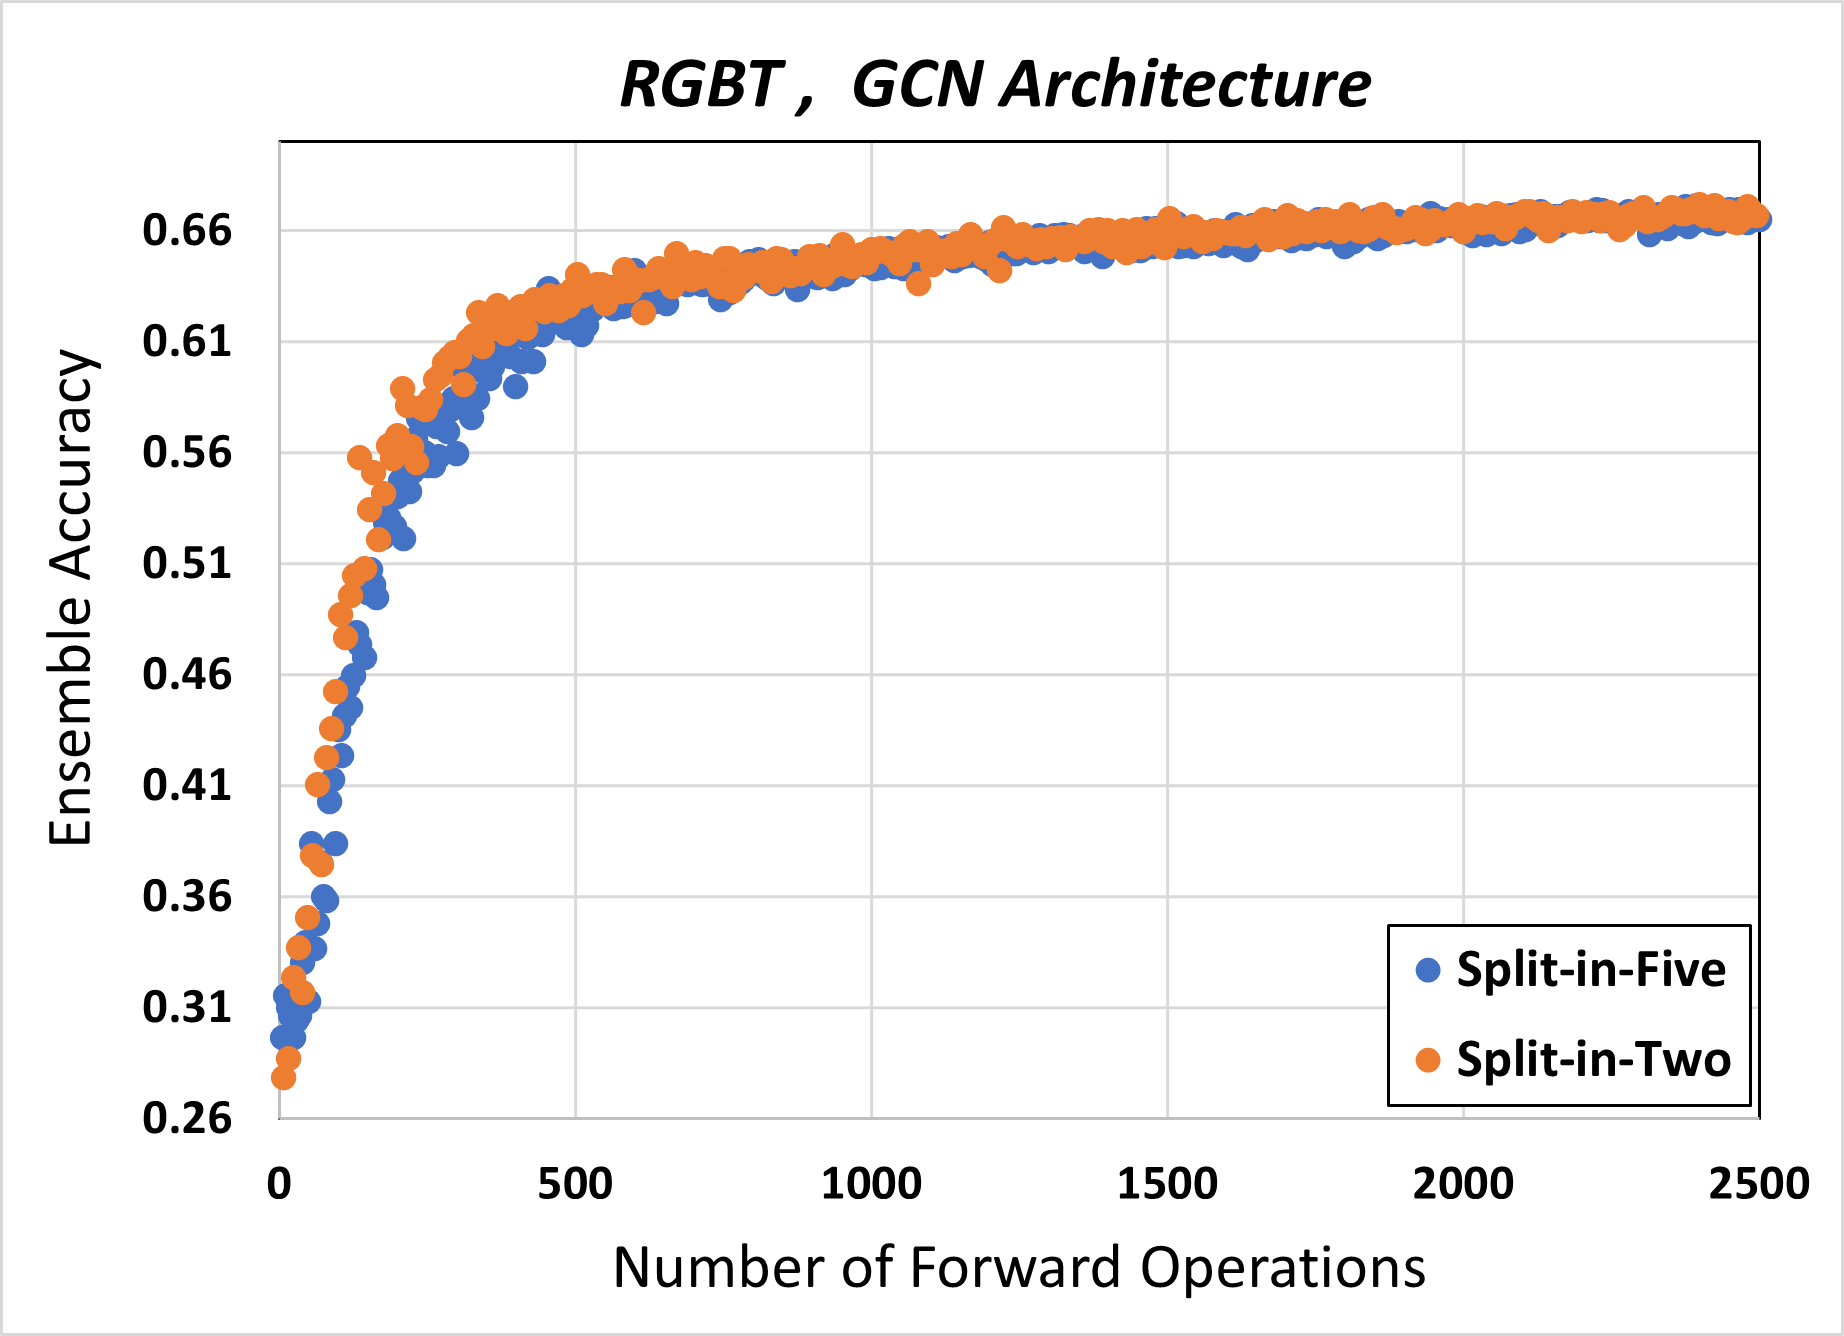}

\includegraphics[width=0.32\textwidth]{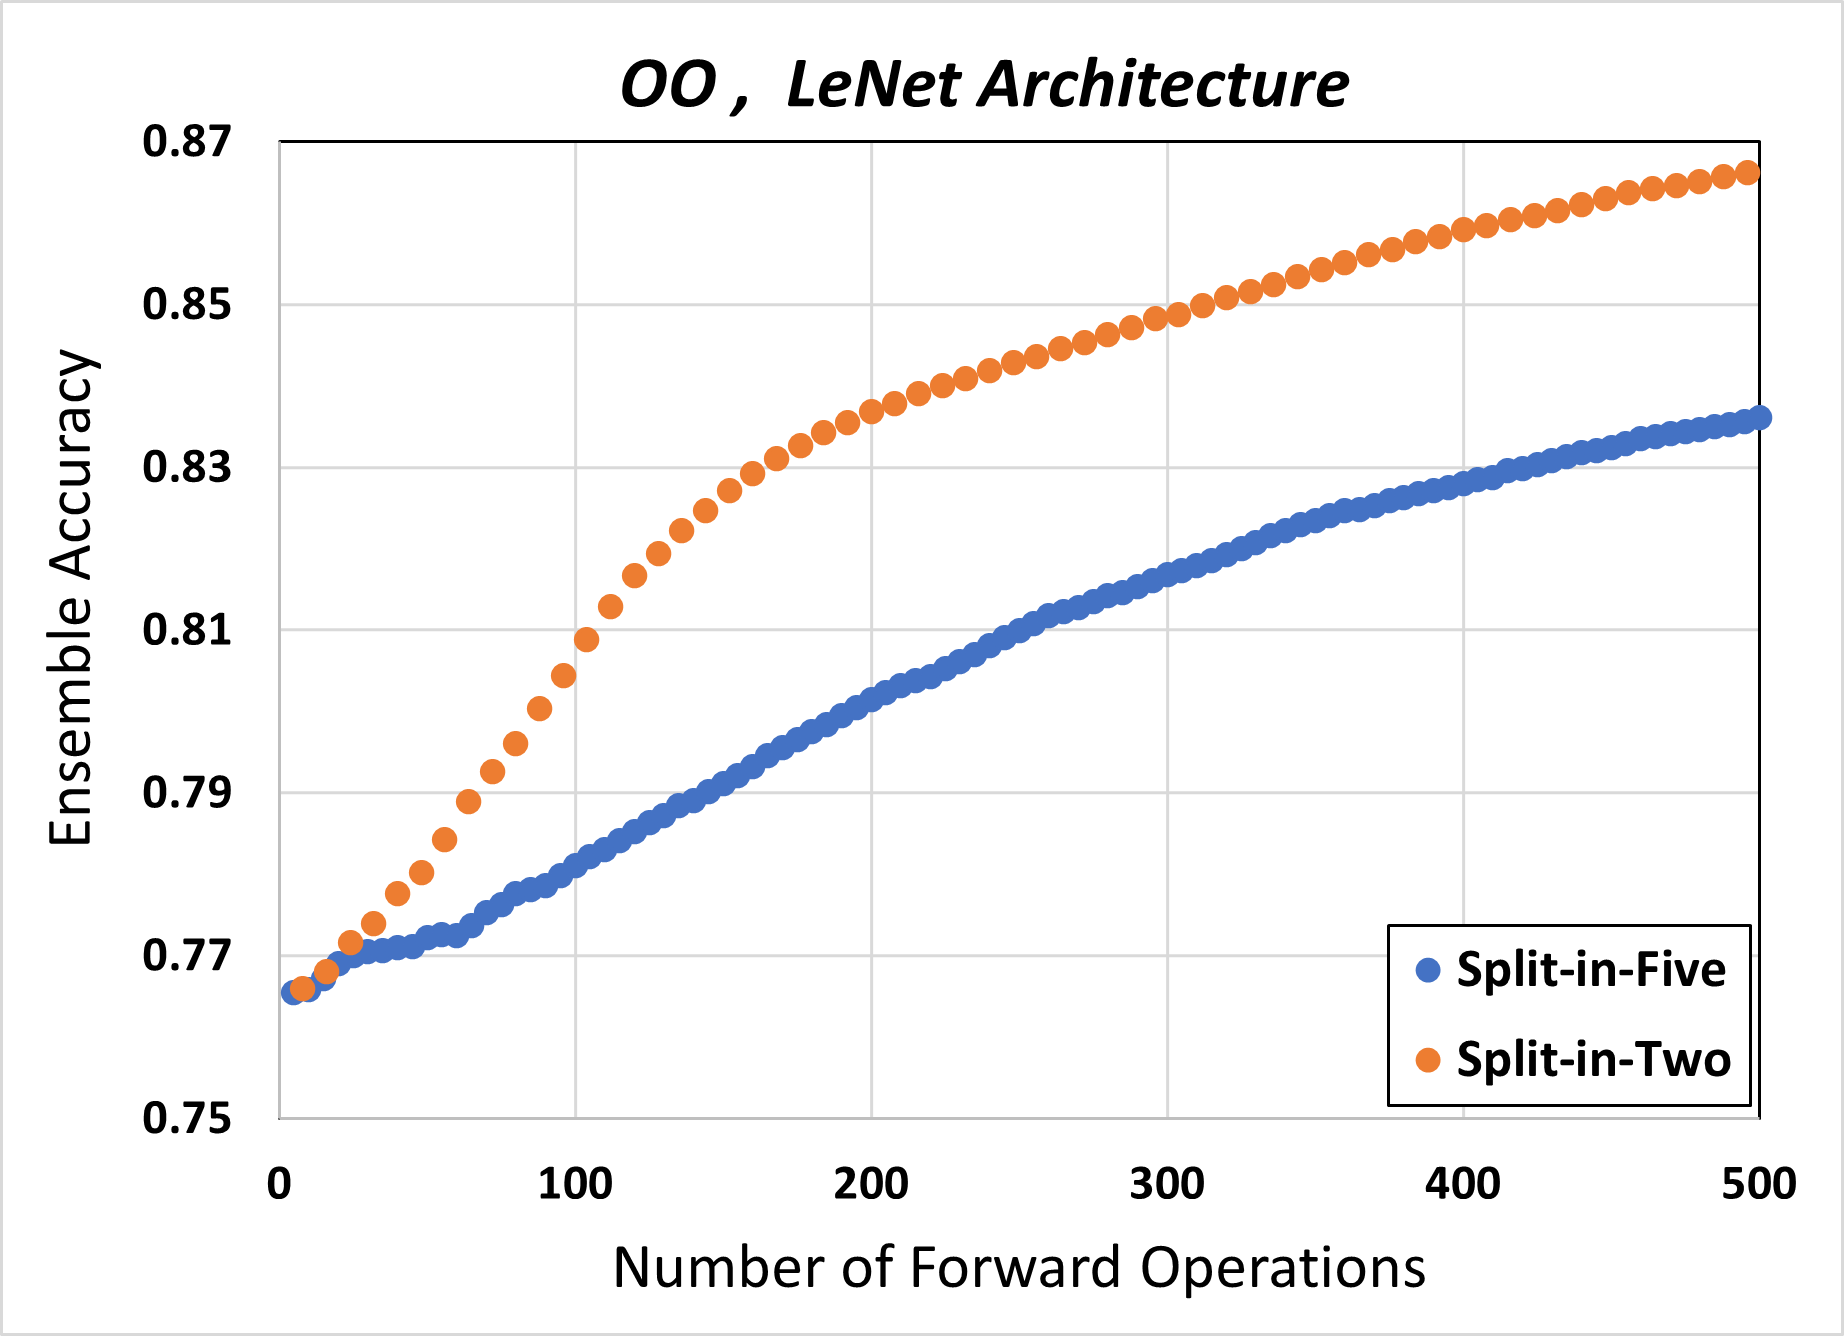}
\includegraphics[width=0.32\textwidth]{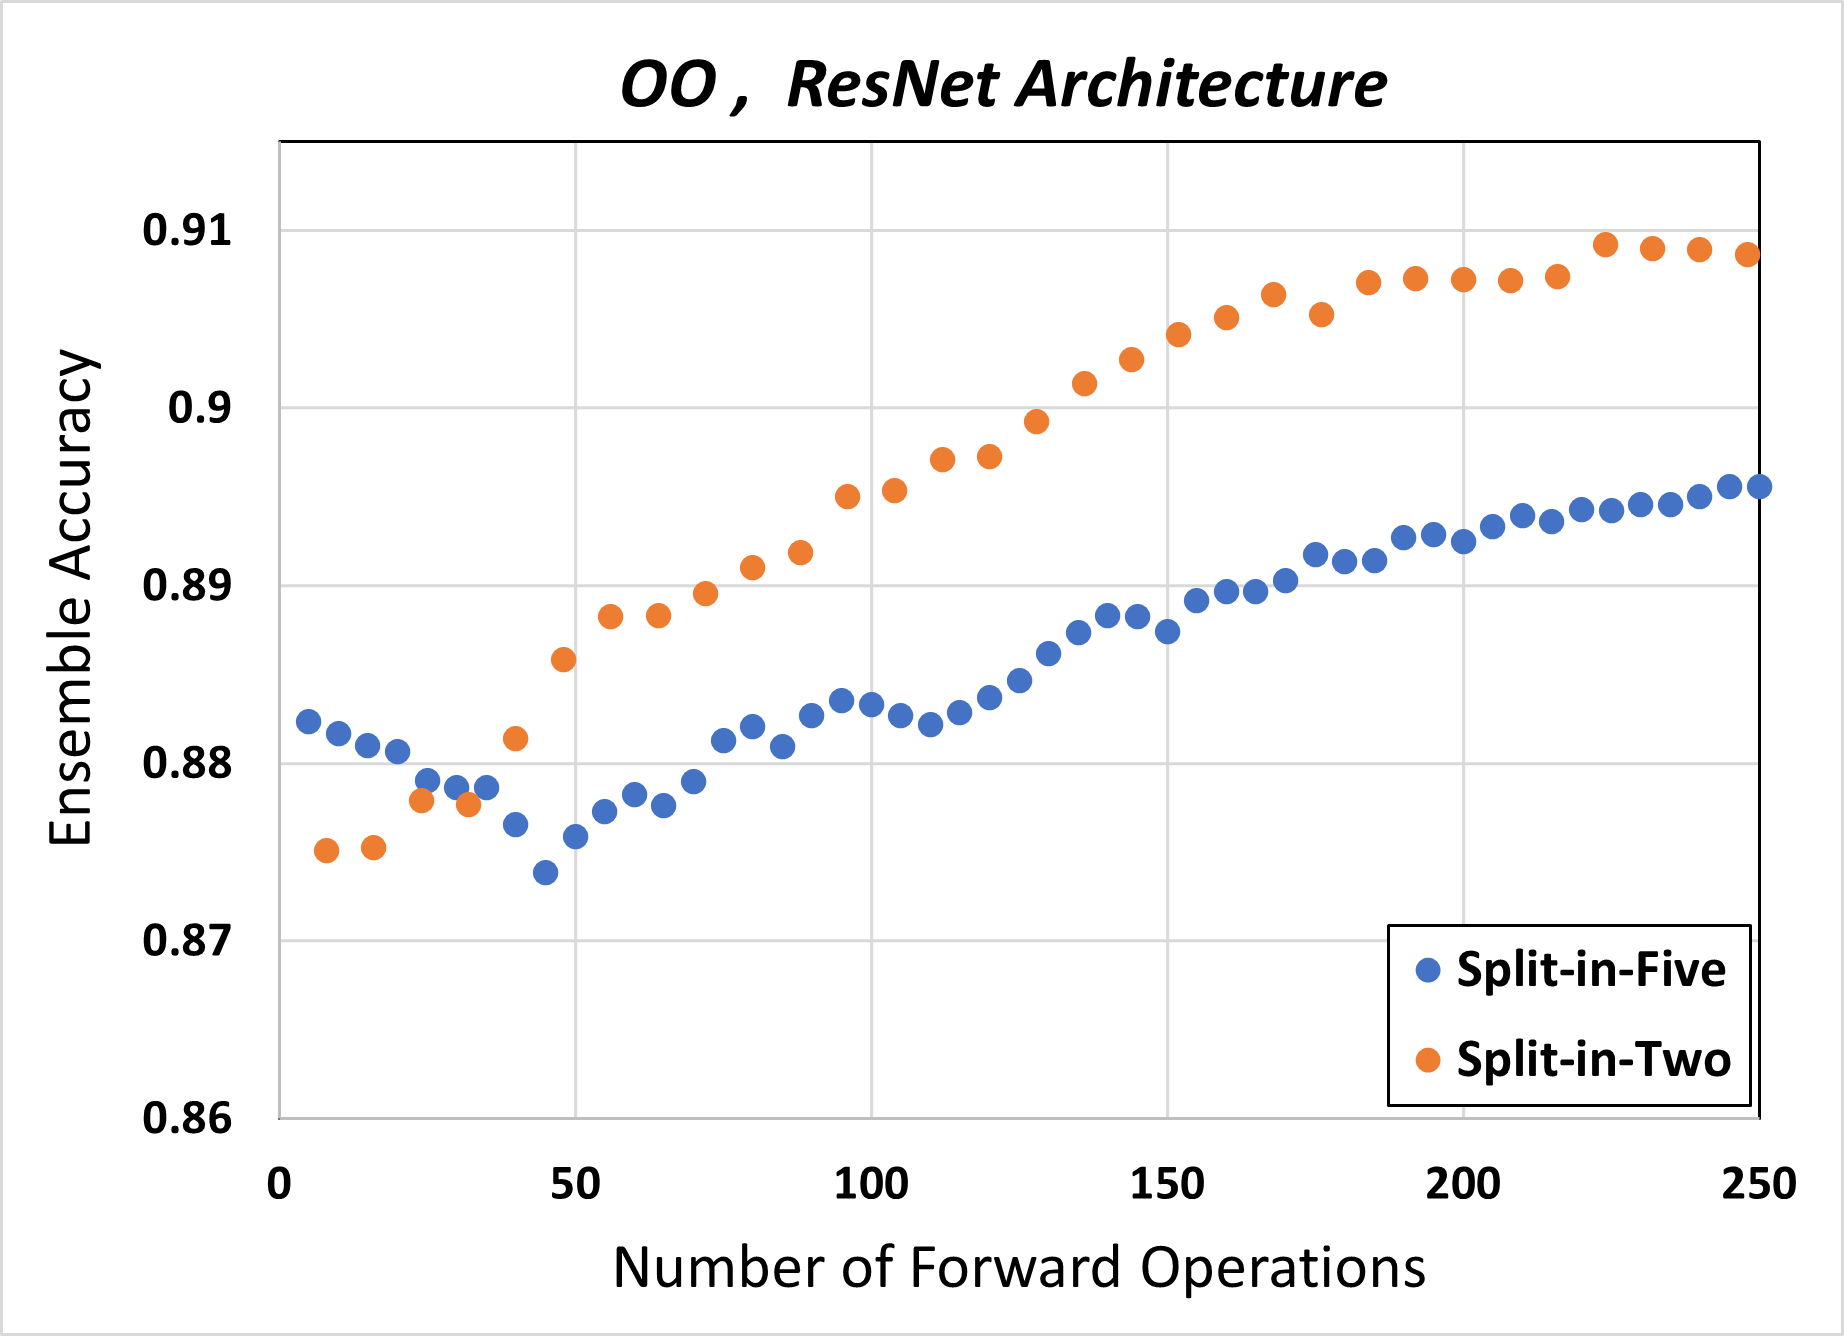}
\includegraphics[width=0.32\textwidth]{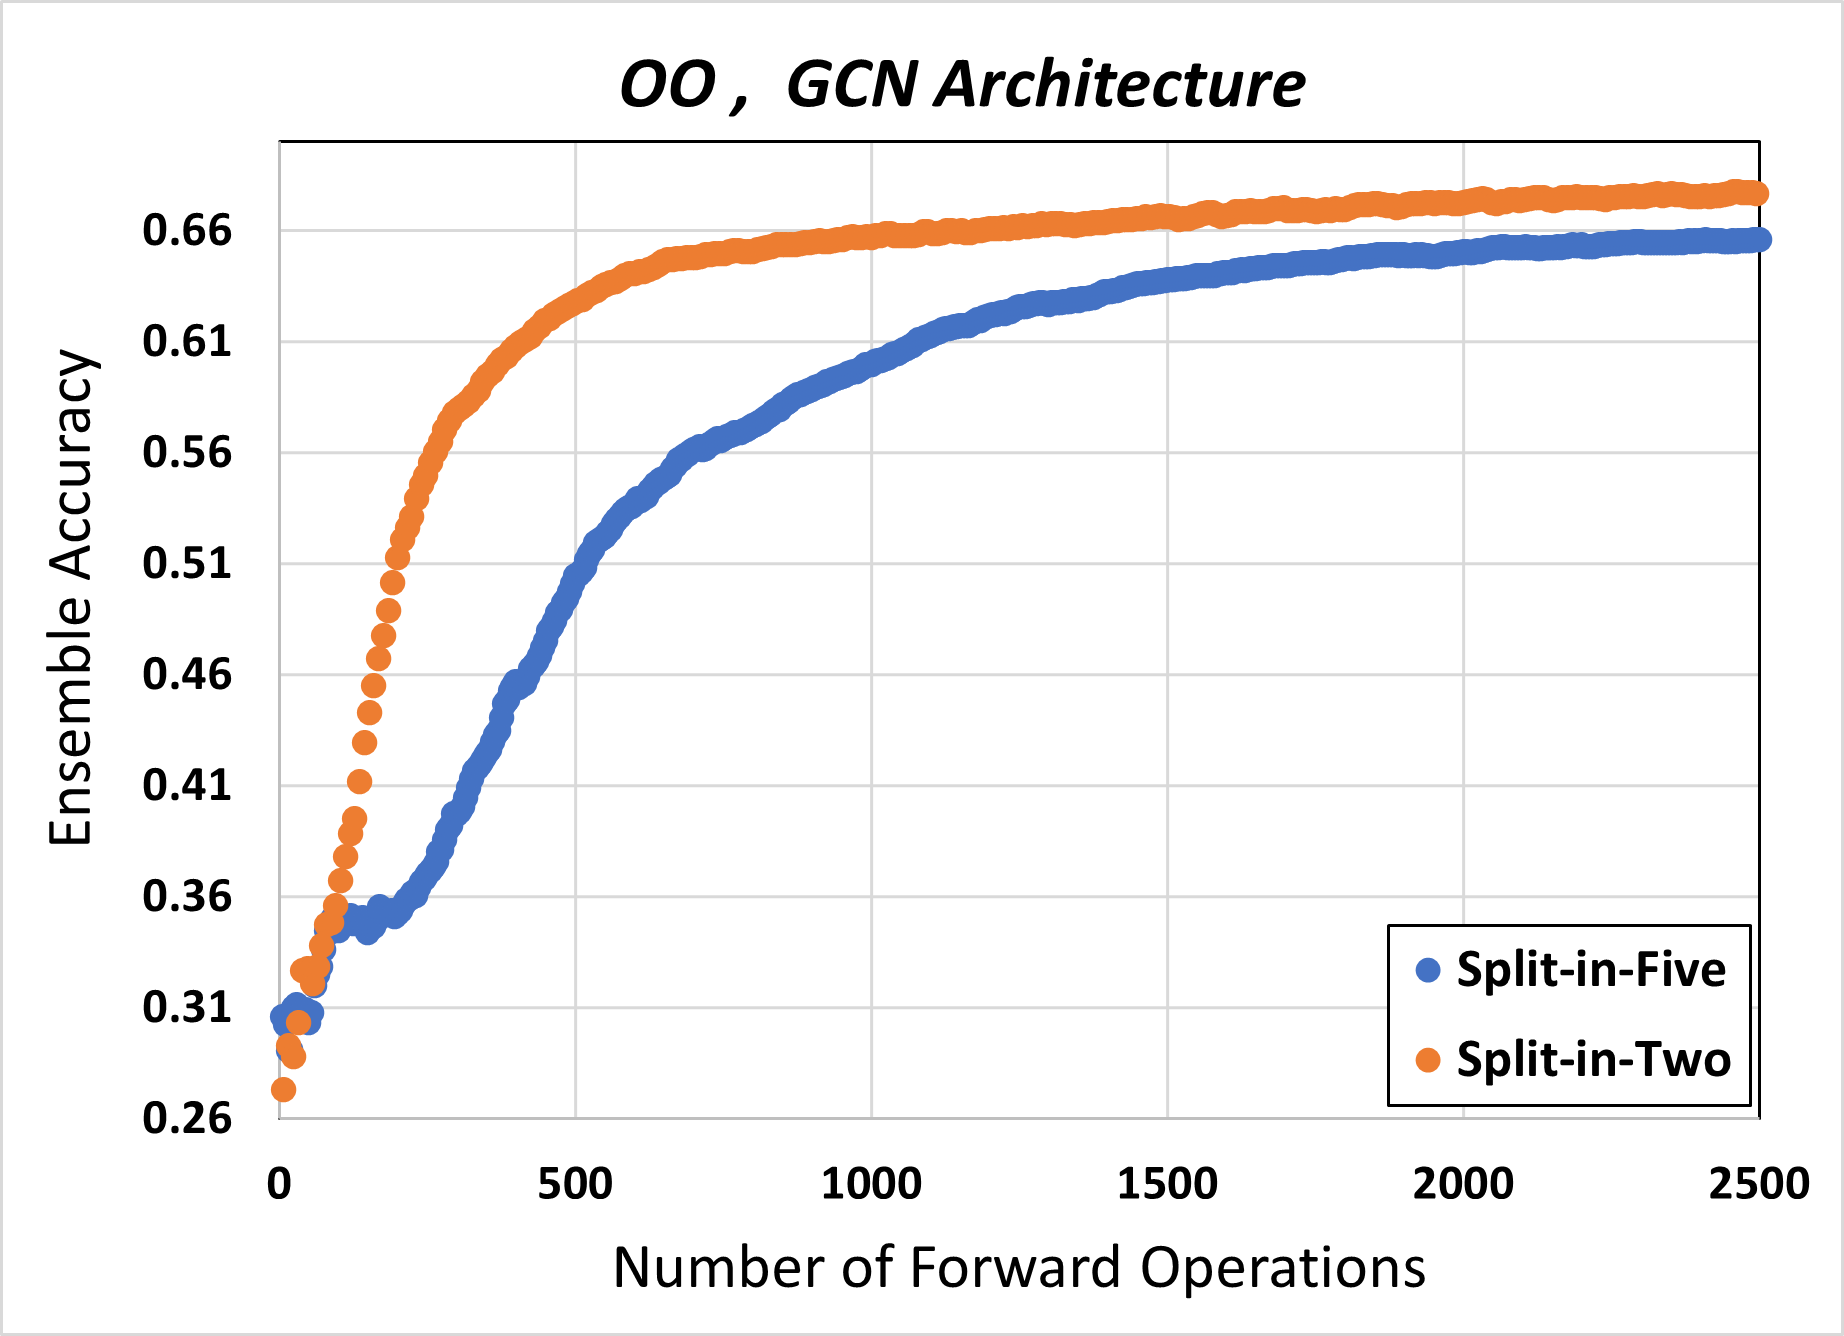}

\caption{Ensemble accuracy $acc_{\cal E}$ on test set as a function of number of \textit{Forward Operations}. As expected, Split-In-Two out performs Split-In-Five, since it makes 4X higher use of the training set}
\label{fig:forward-gcn}
\end{figure*}

% \input{Figures/Forward_Operations/GCN/Pretrain/fig.tex}
% \input{Figures/Forward_Operations/Lenet/Pretrain/fig.tex}
% \input{Figures/Forward_Operations/Resnet/Pretrain/fig.tex}

% % Ground: Supplementary
\begin{figure*}[h]
\centering
\includegraphics[width=0.3\textwidth]{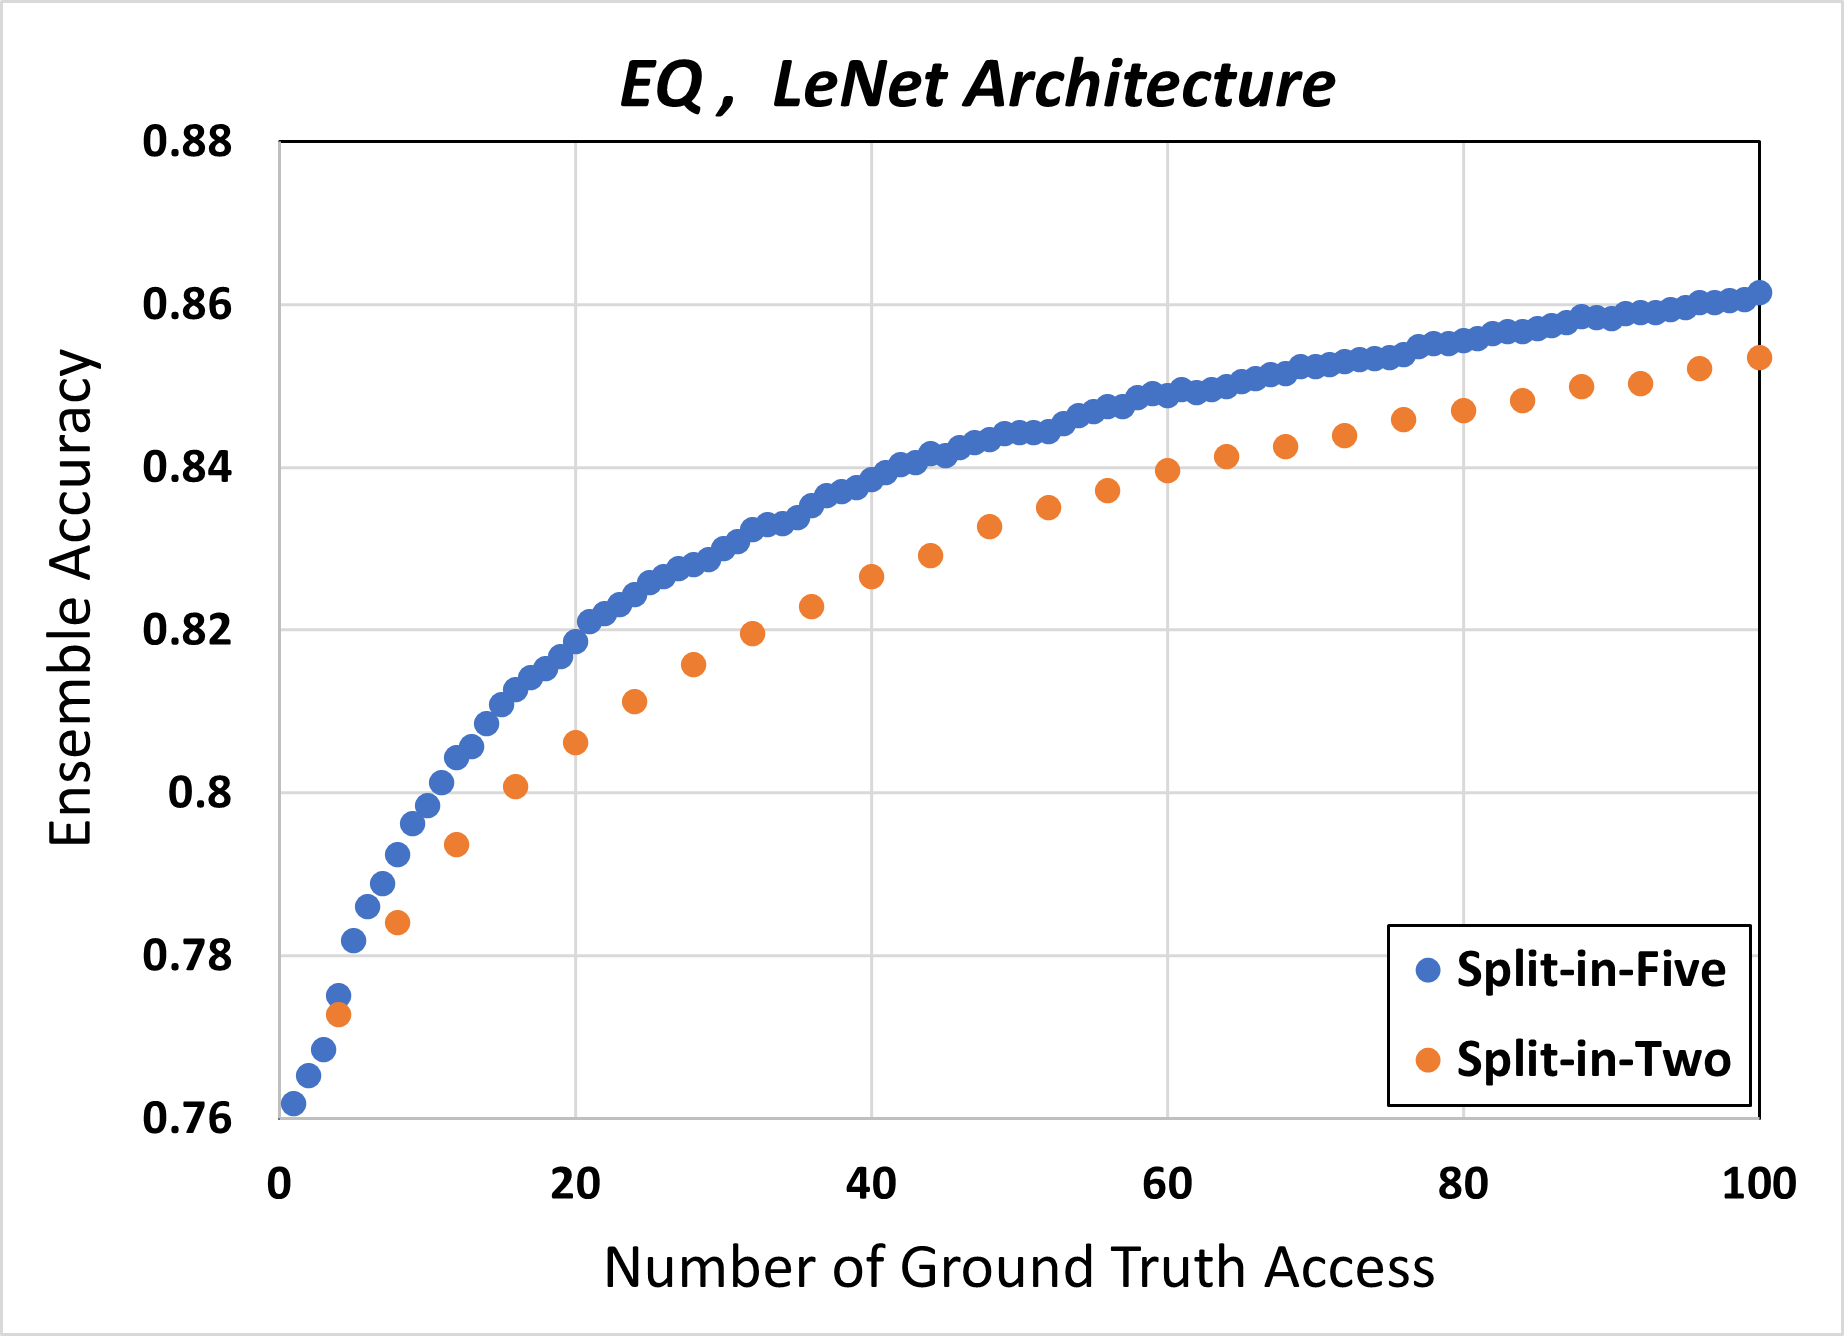}
\includegraphics[width=0.3\textwidth]{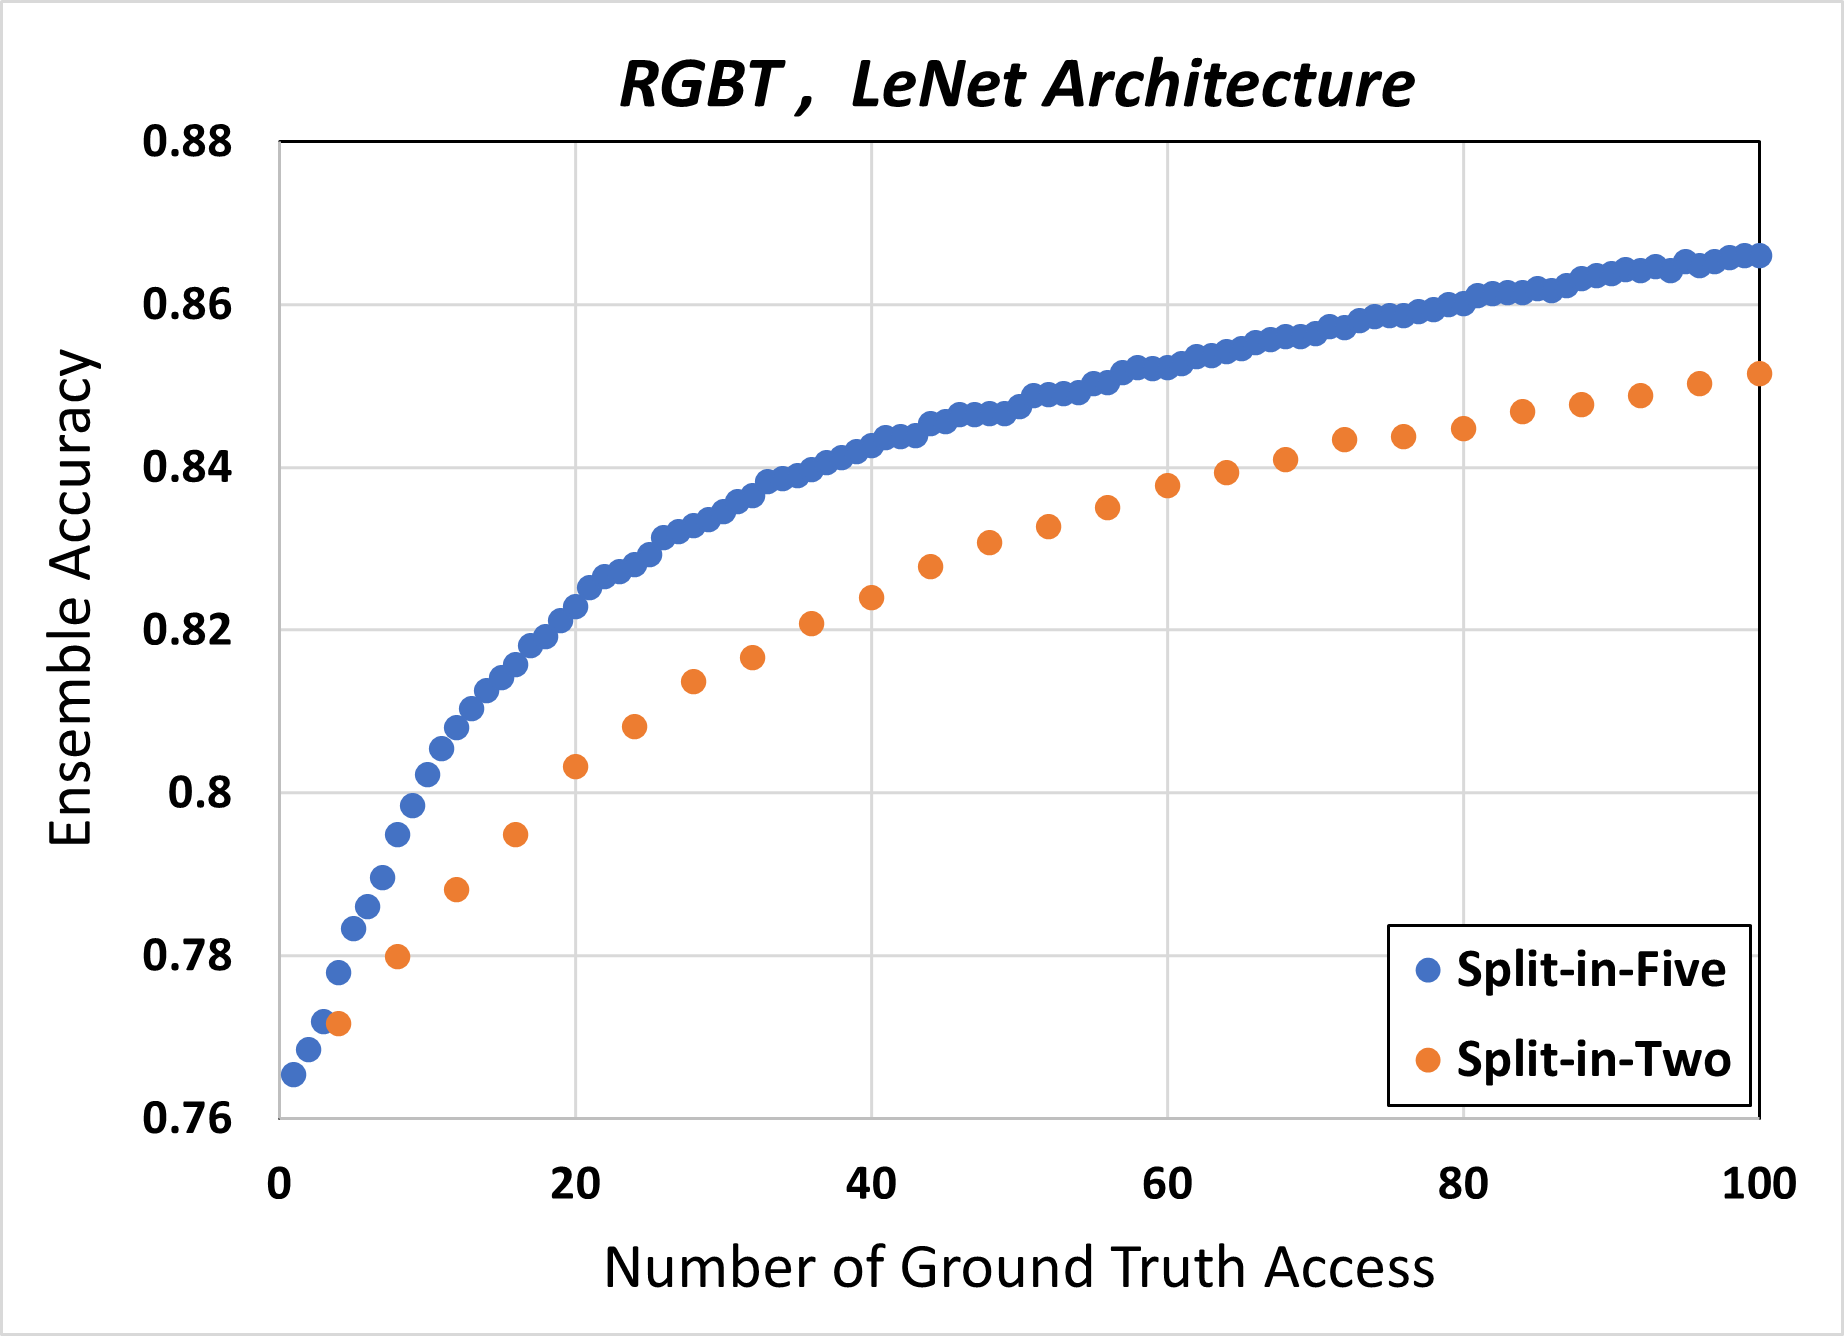}
\includegraphics[width=0.3\textwidth]{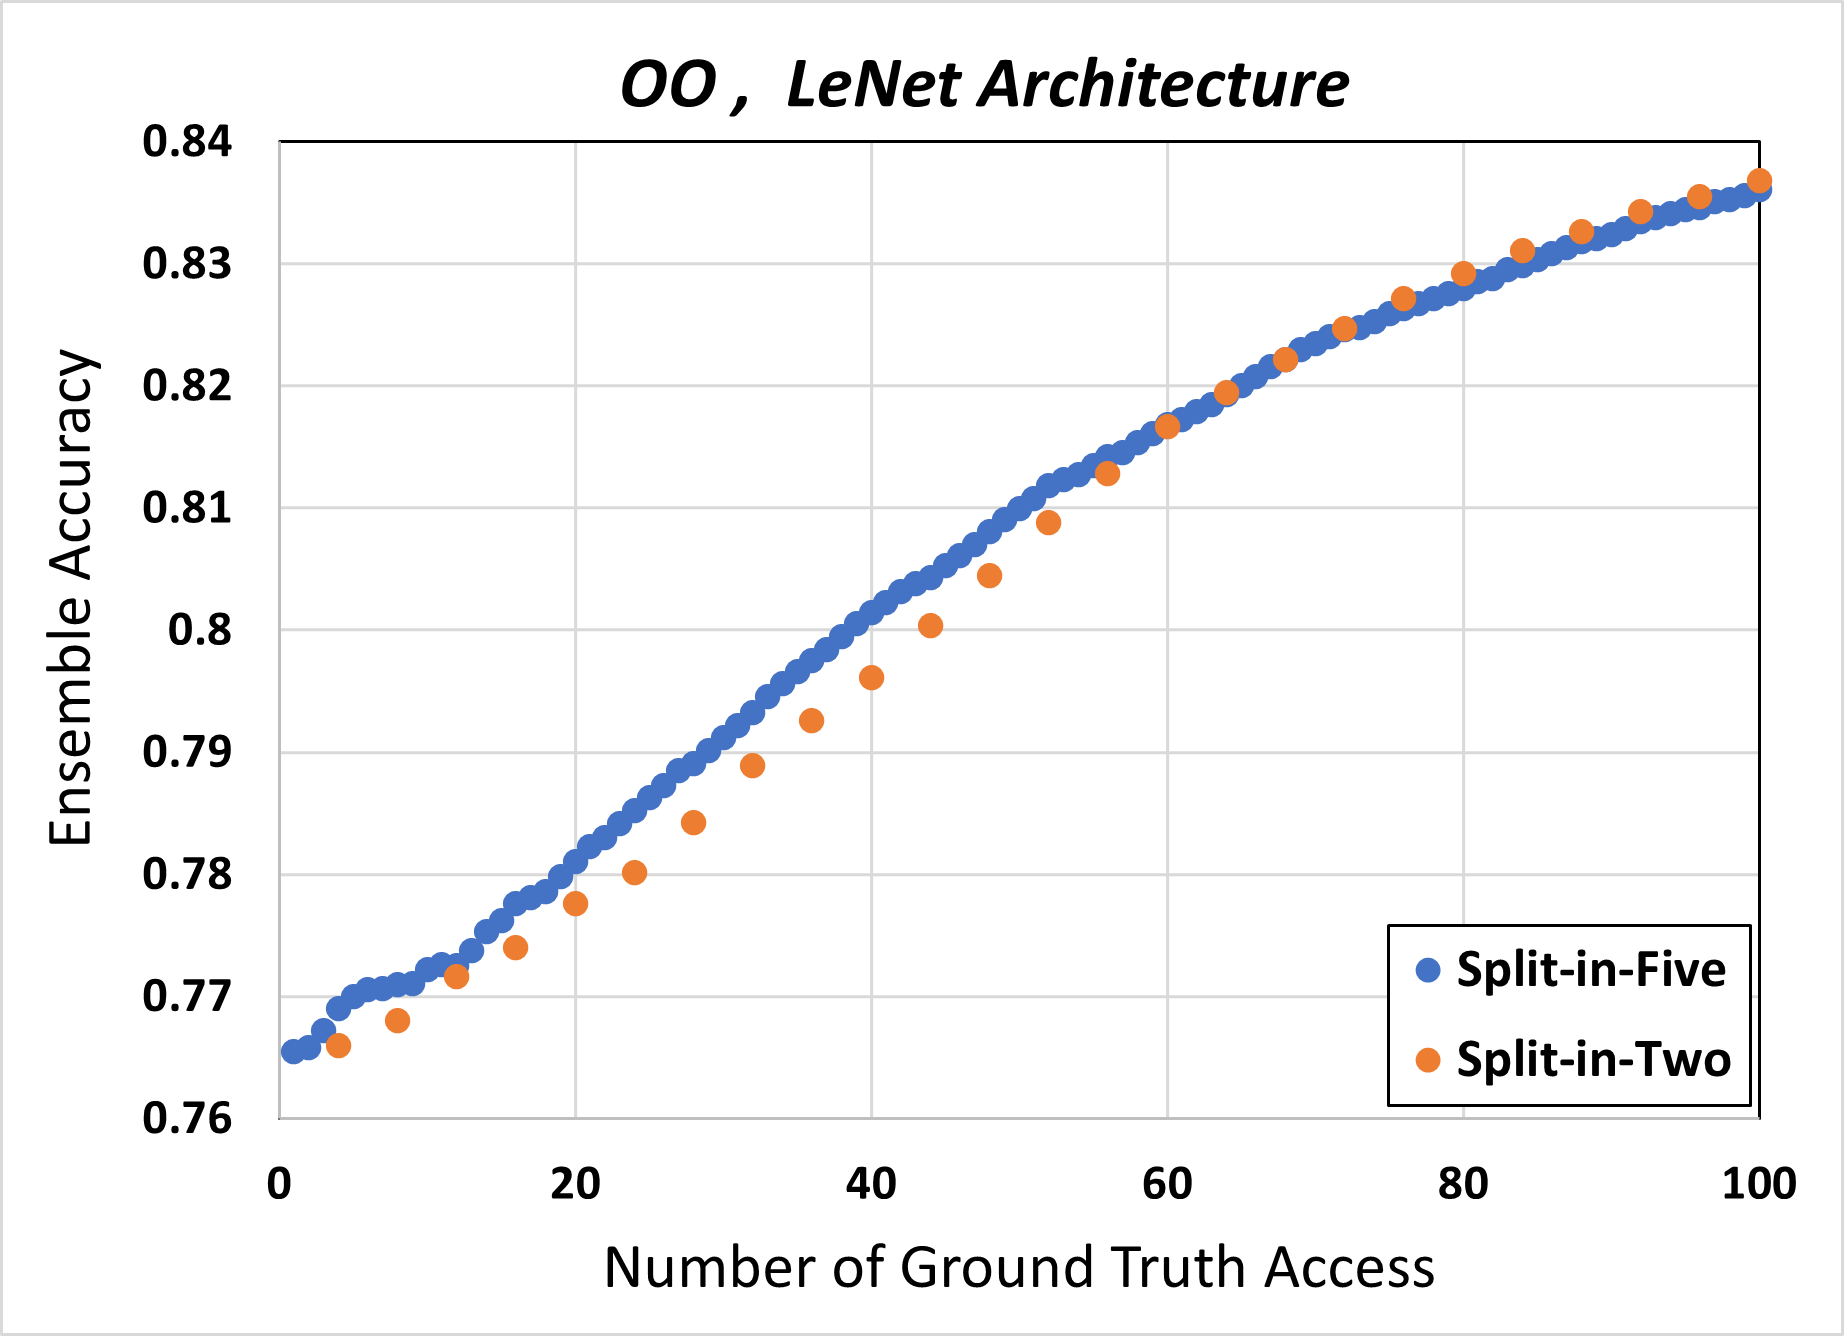}
\includegraphics[width=0.3\textwidth]{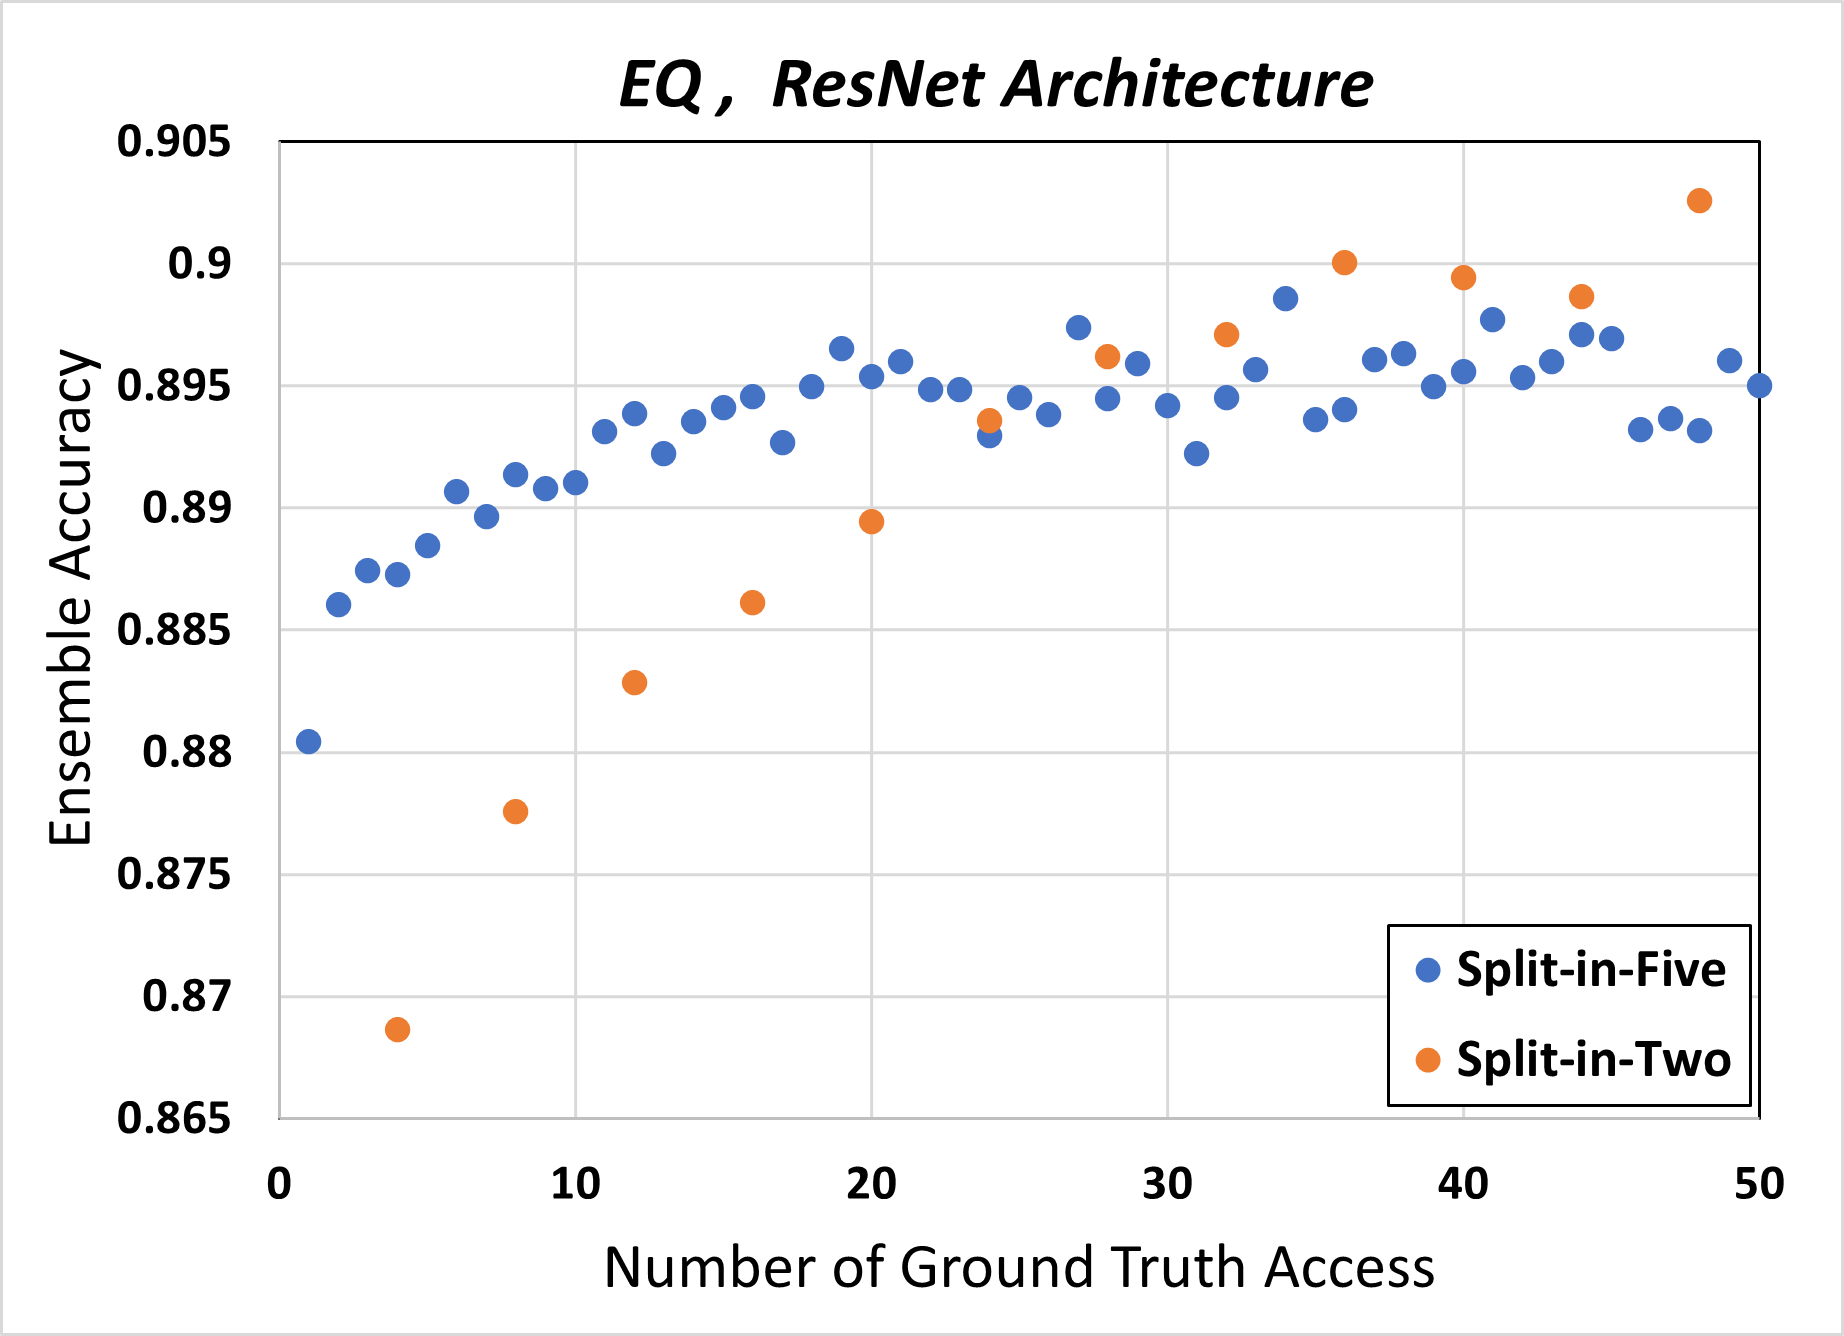}
\includegraphics[width=0.3\textwidth]{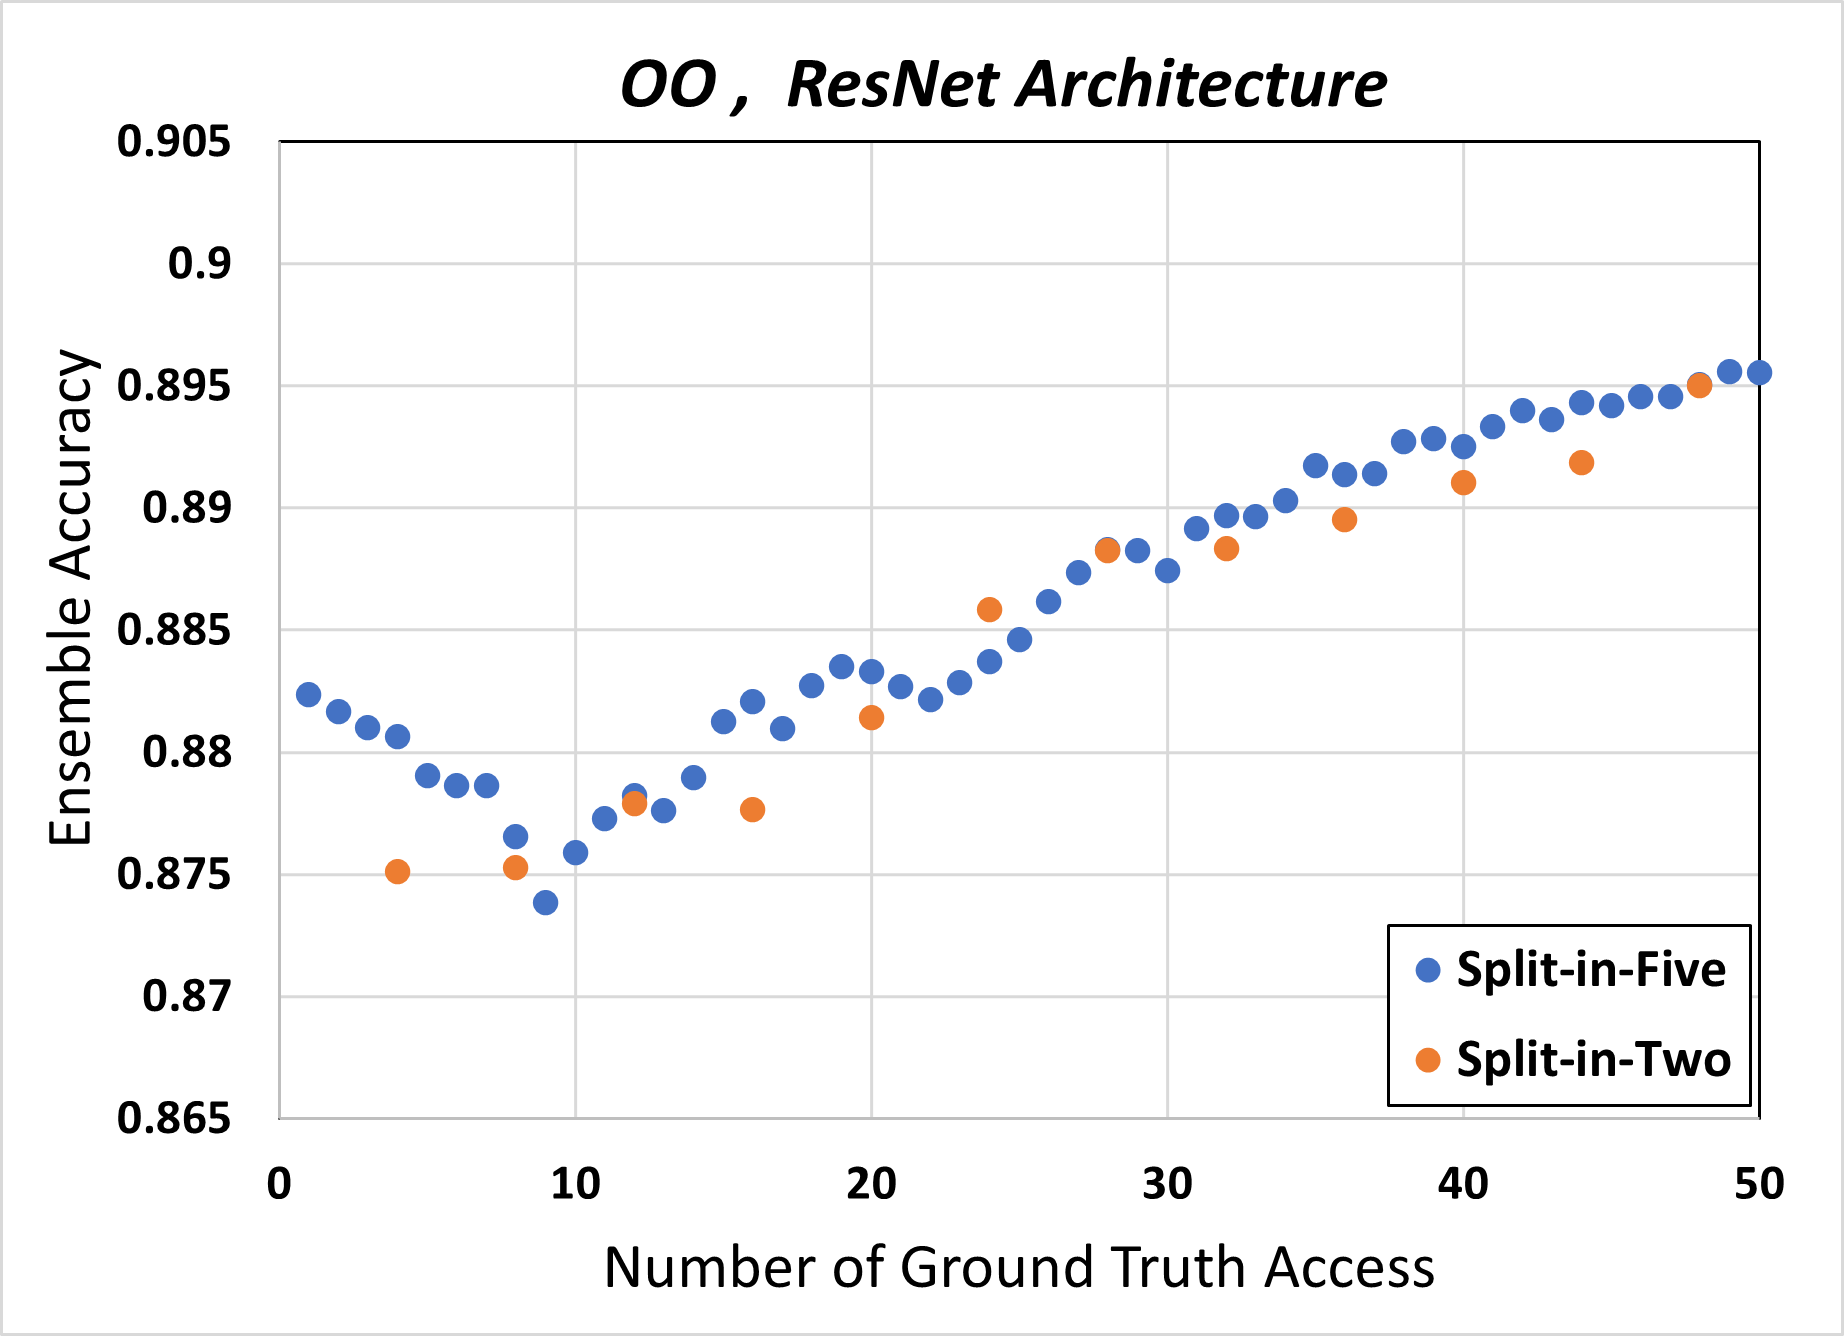}
\includegraphics[width=0.3\textwidth]{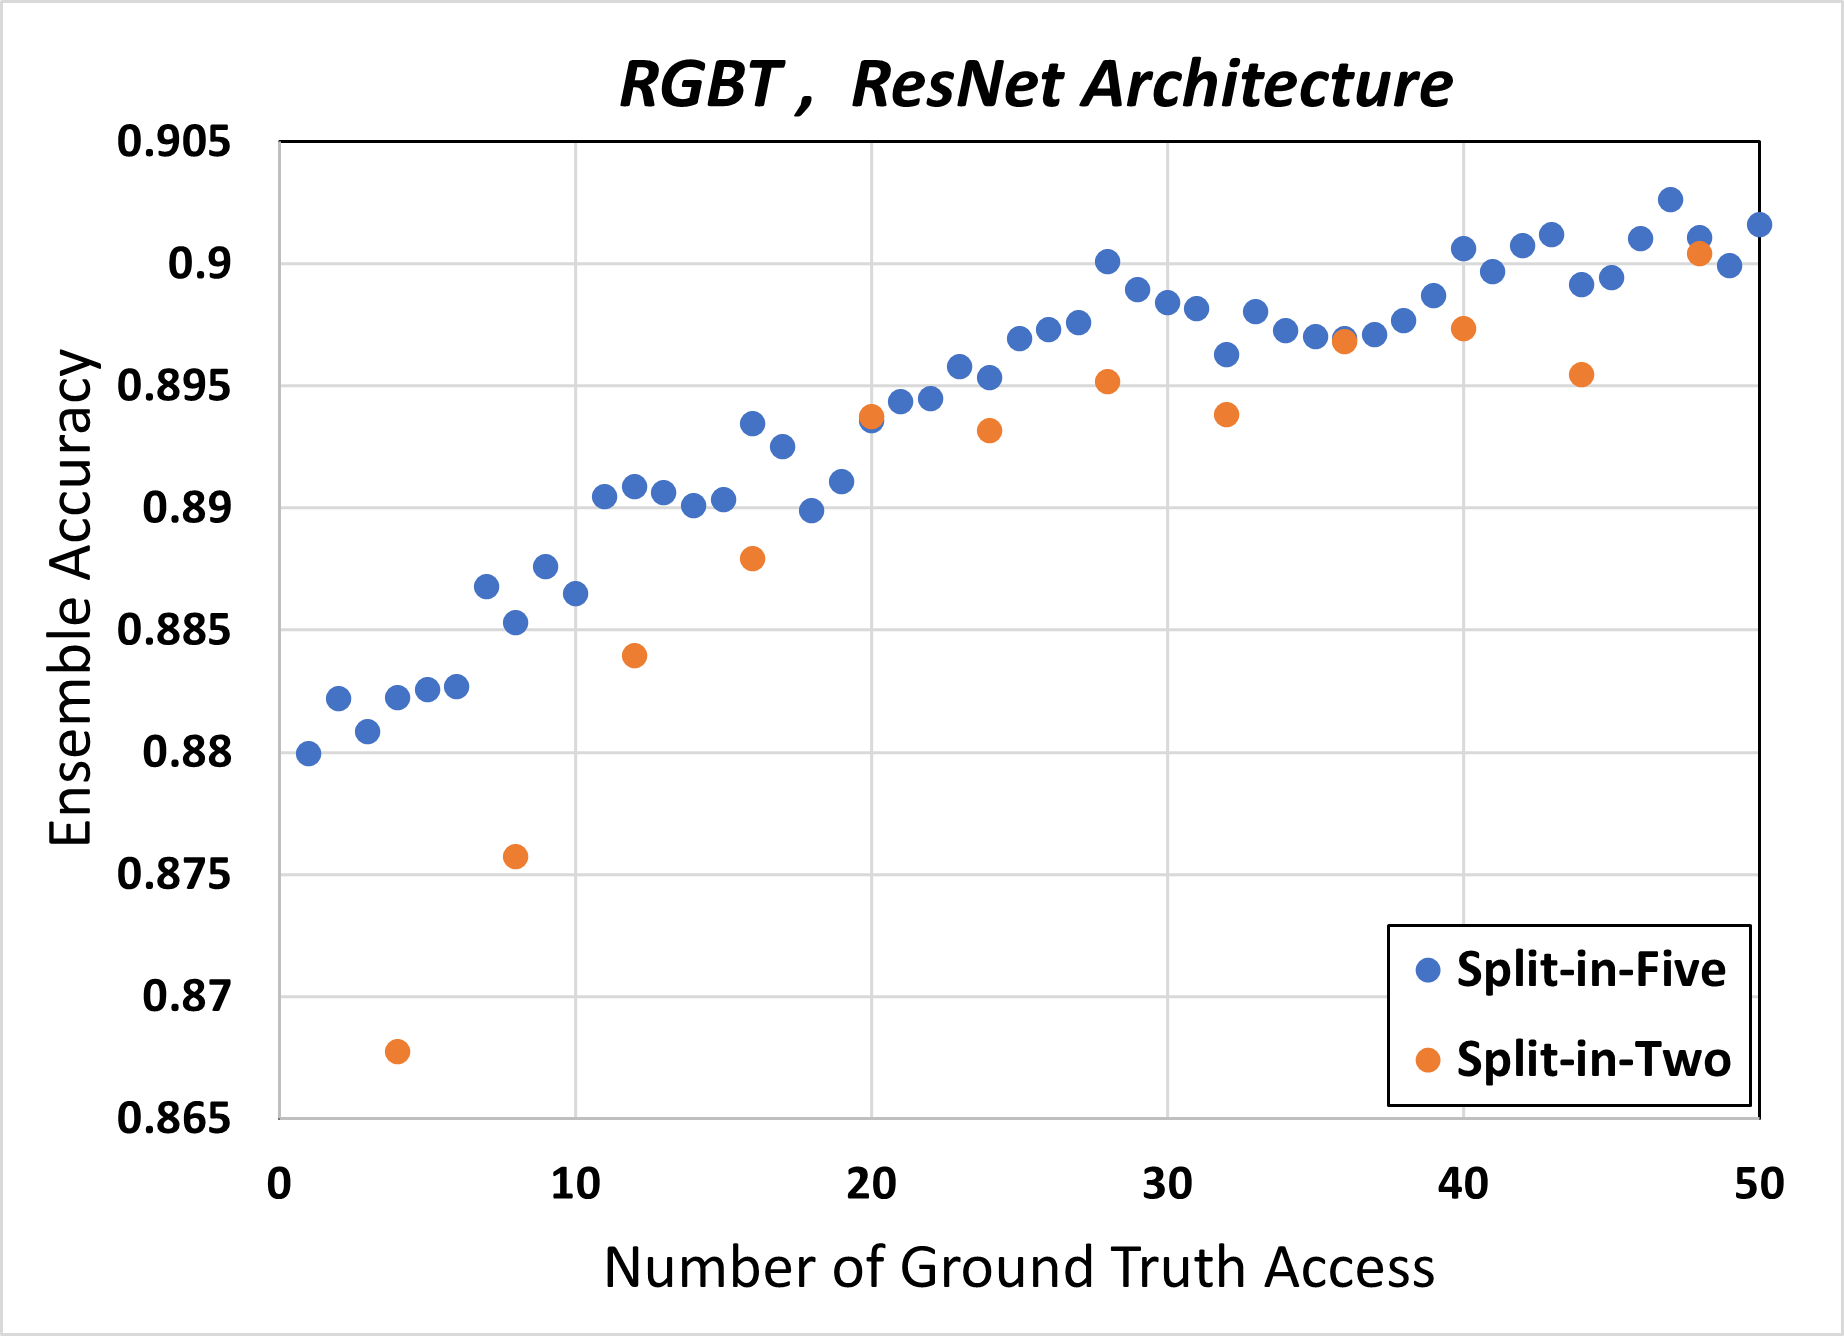}
\caption{Ensemble accuracy $acc_{\cal E}$ on test set as a function of the number $\alpha$ of oracle sessions, for \textit{C=2} and \textit{C=5}. Figures for \textit{EQ}, \textit{RGBT} and \textit{OO} are shown here, results for \textit{BTB} can be found in \textit{Training Resource Utilization} section.}
\label{fig:groun-truth-lenet}
\end{figure*}

\begin{figure*}[h]
\centering
\includegraphics[width=0.42\textwidth]{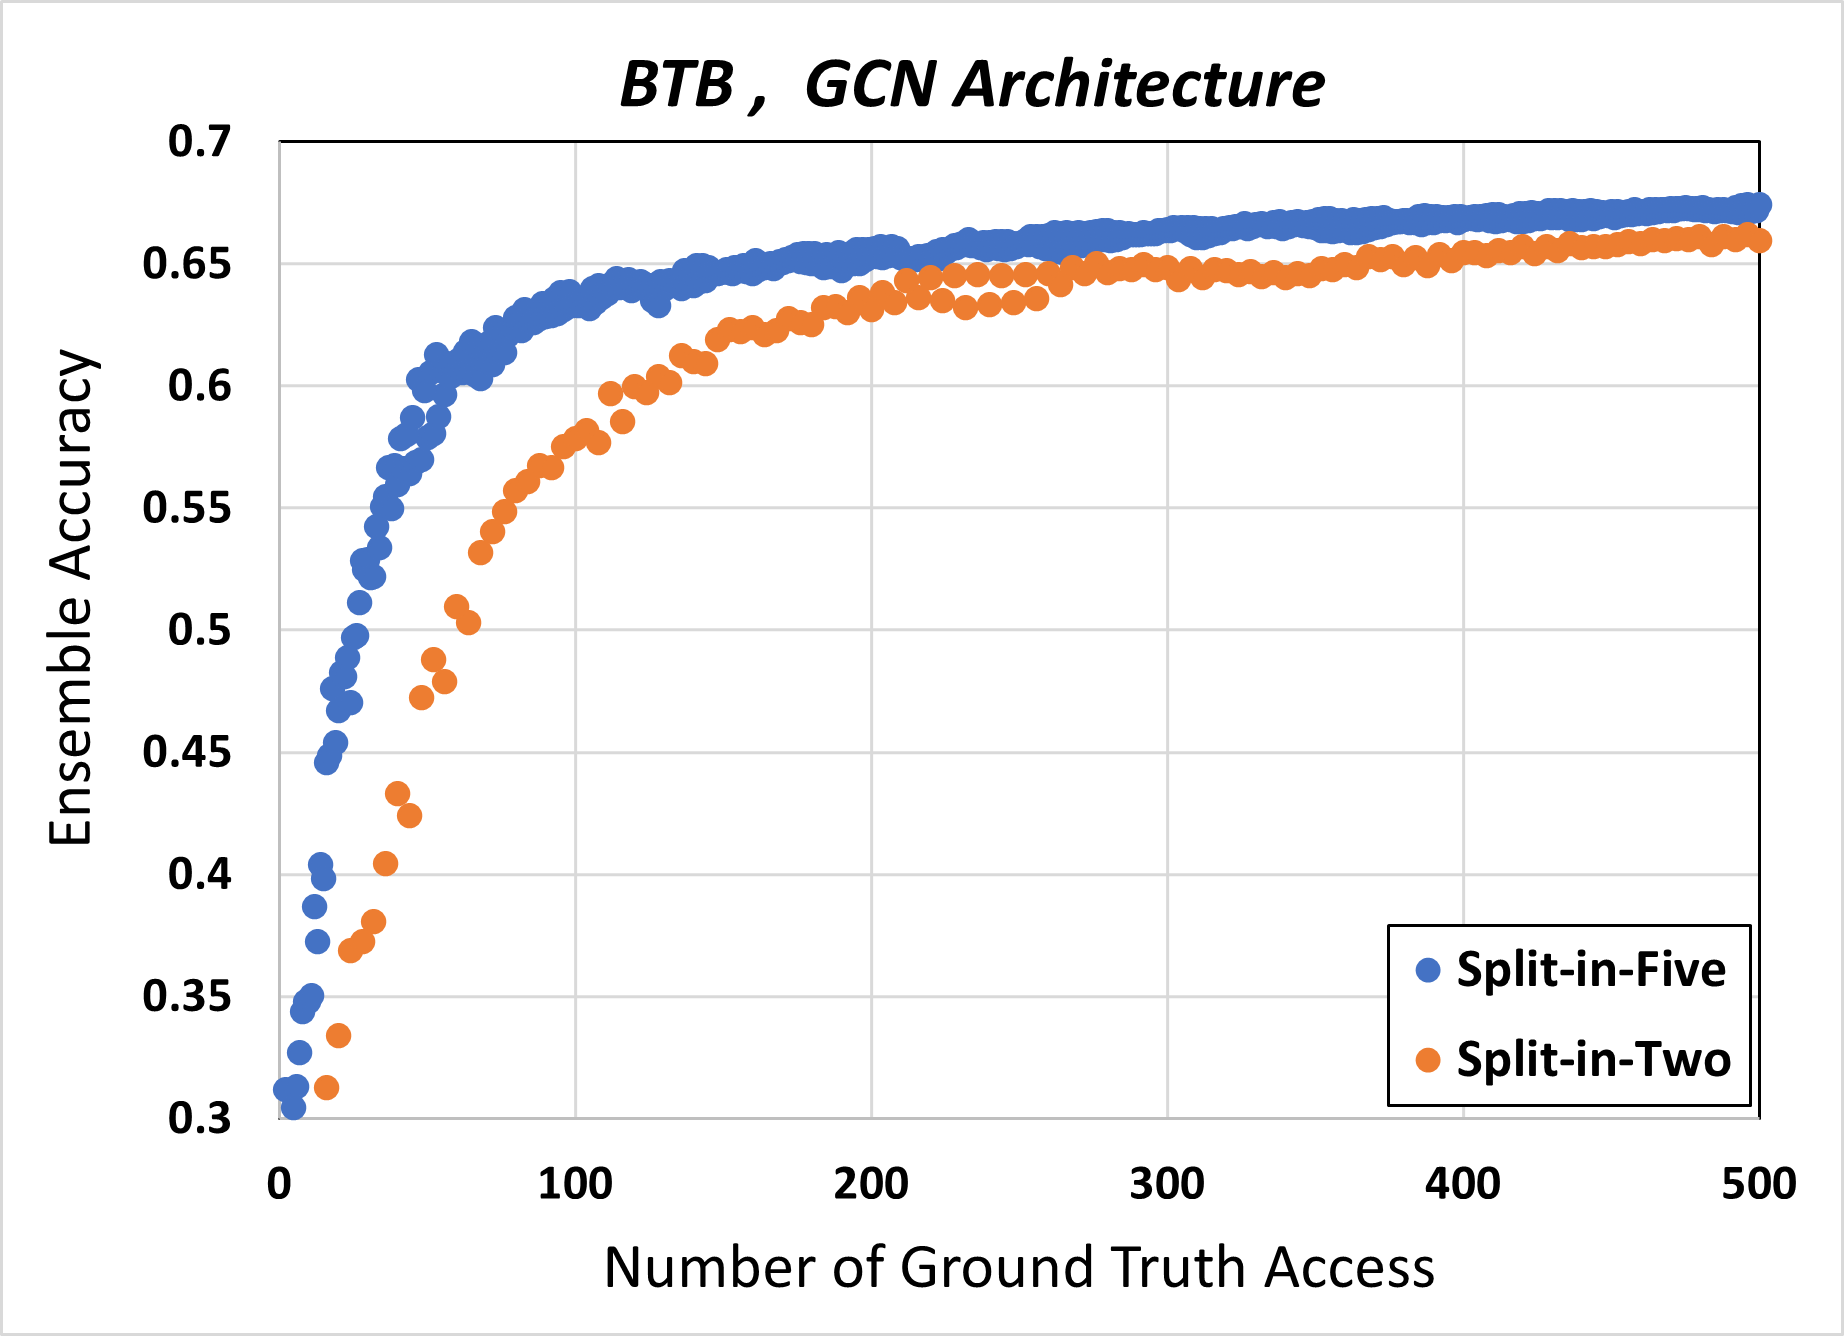}
\includegraphics[width=0.42\textwidth]{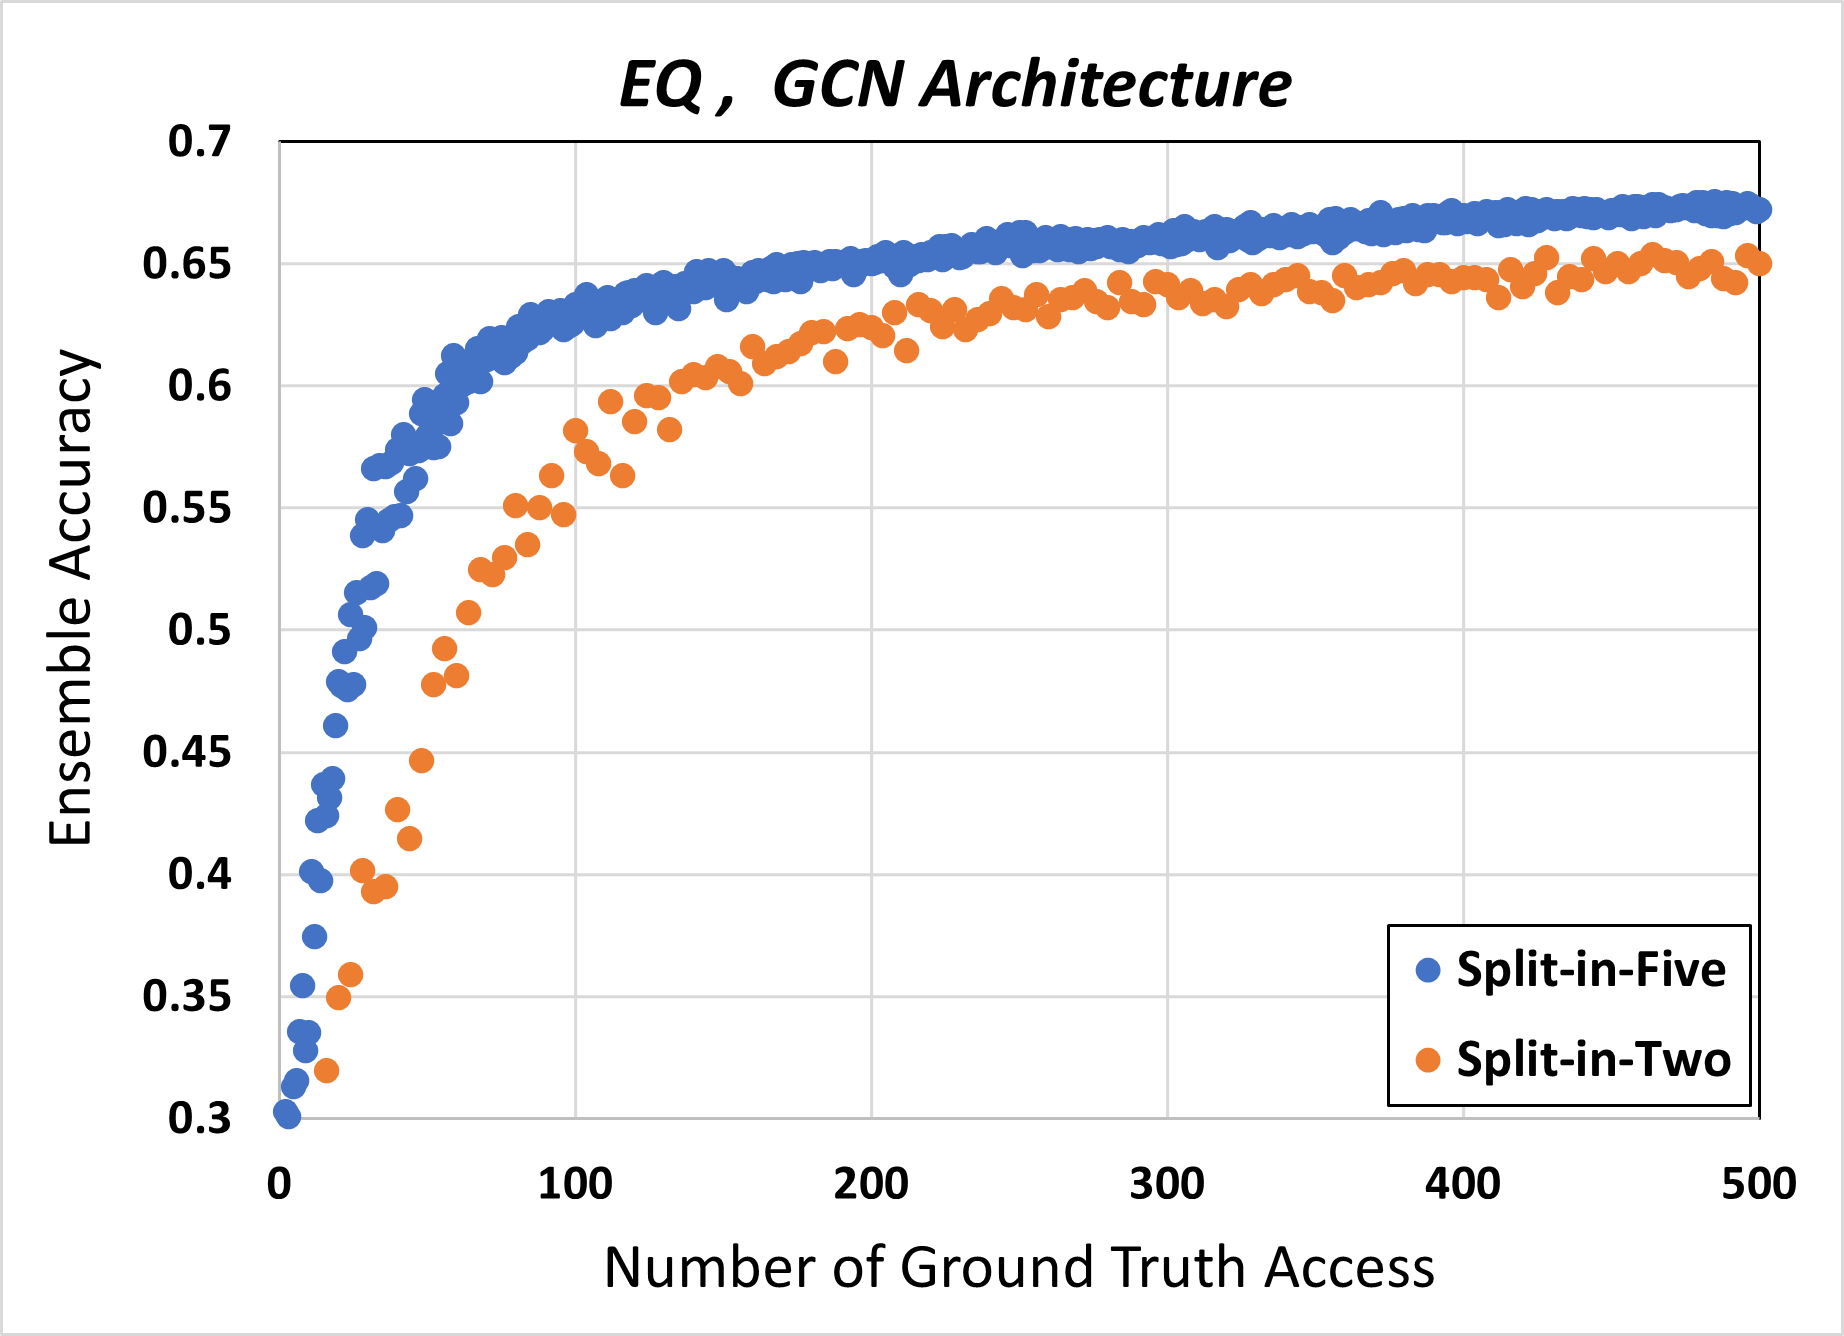}\\
\includegraphics[width=0.42\textwidth]{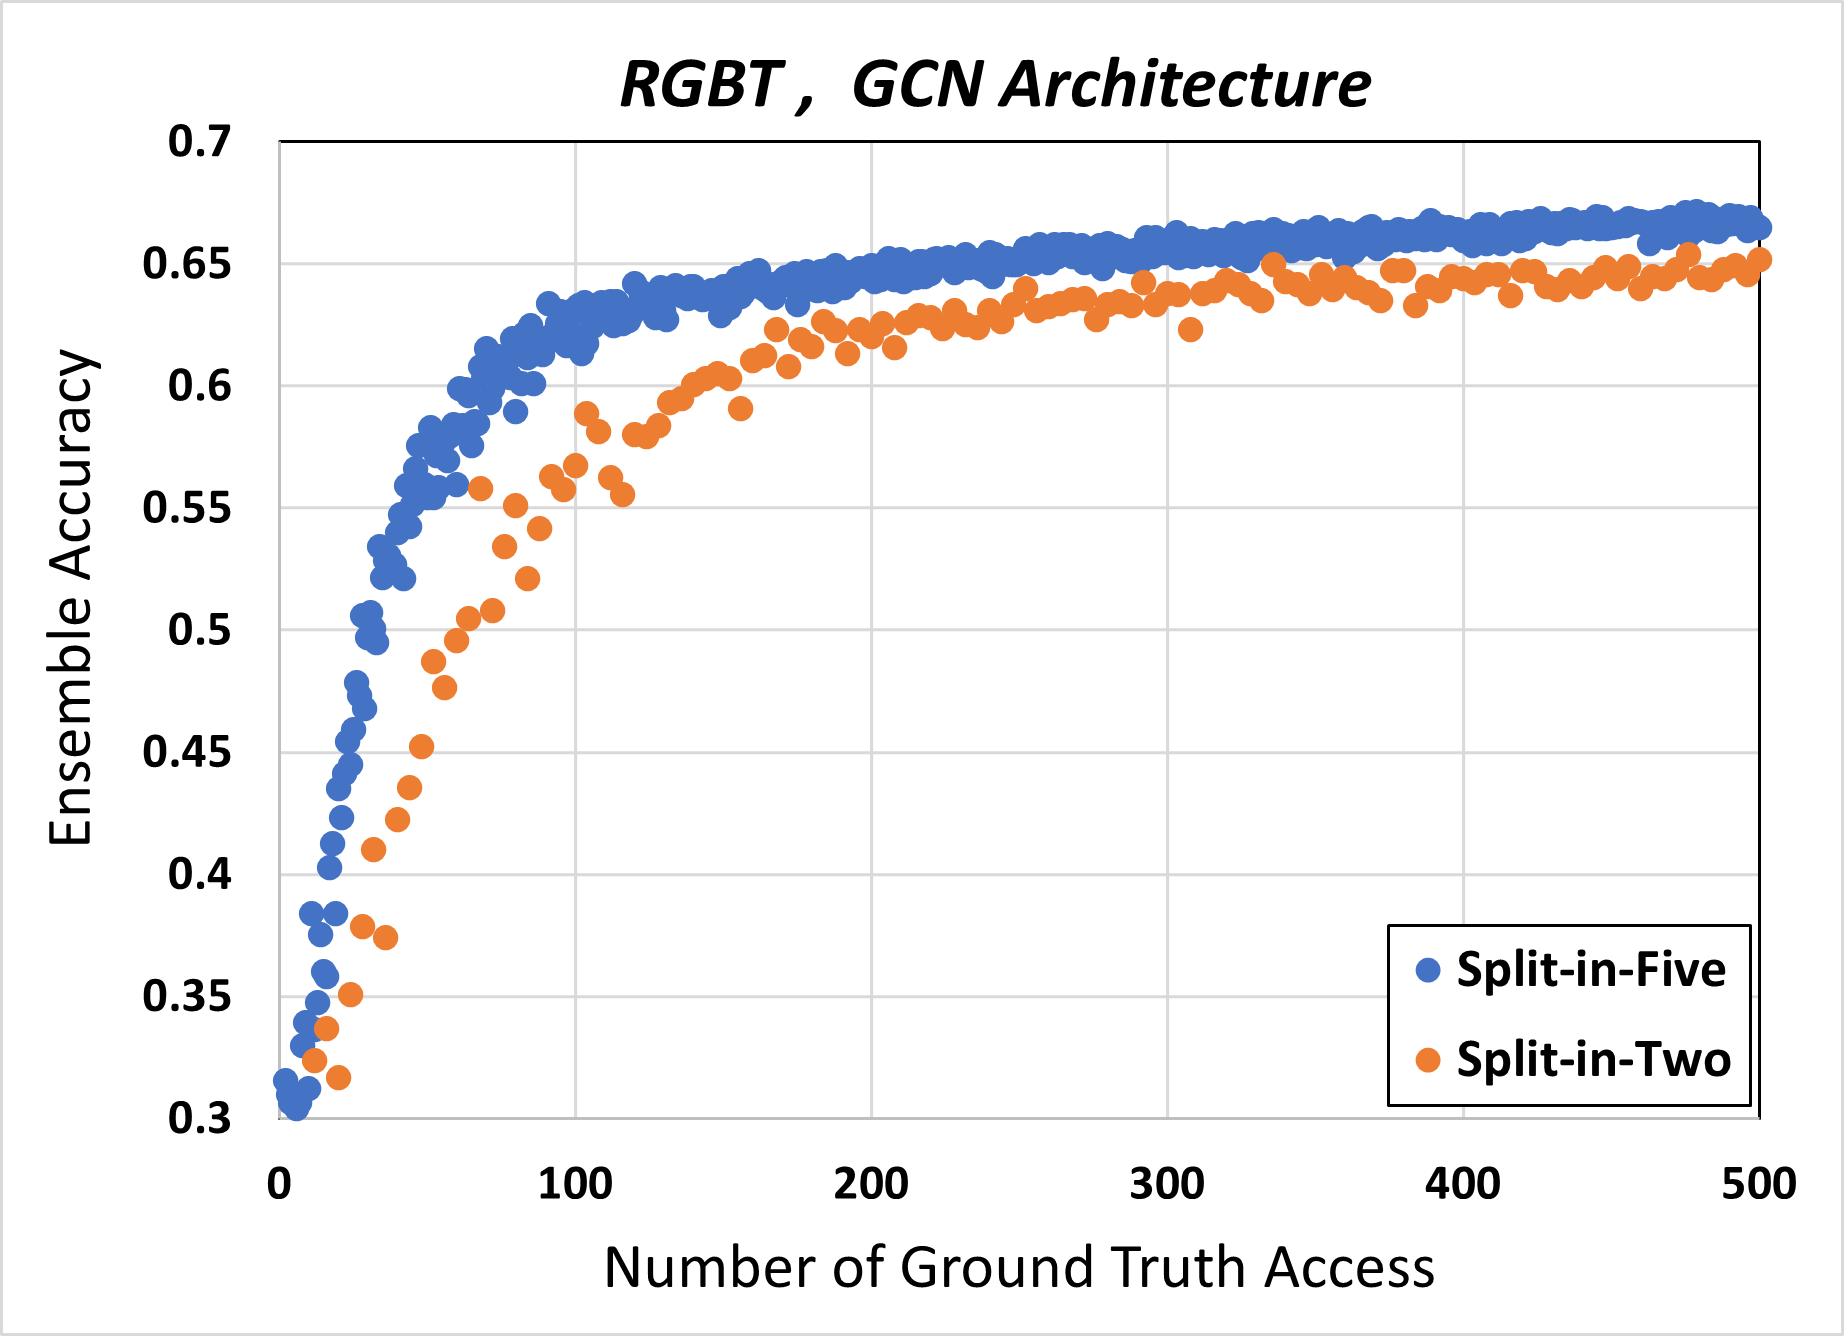}
\includegraphics[width=0.42\textwidth]{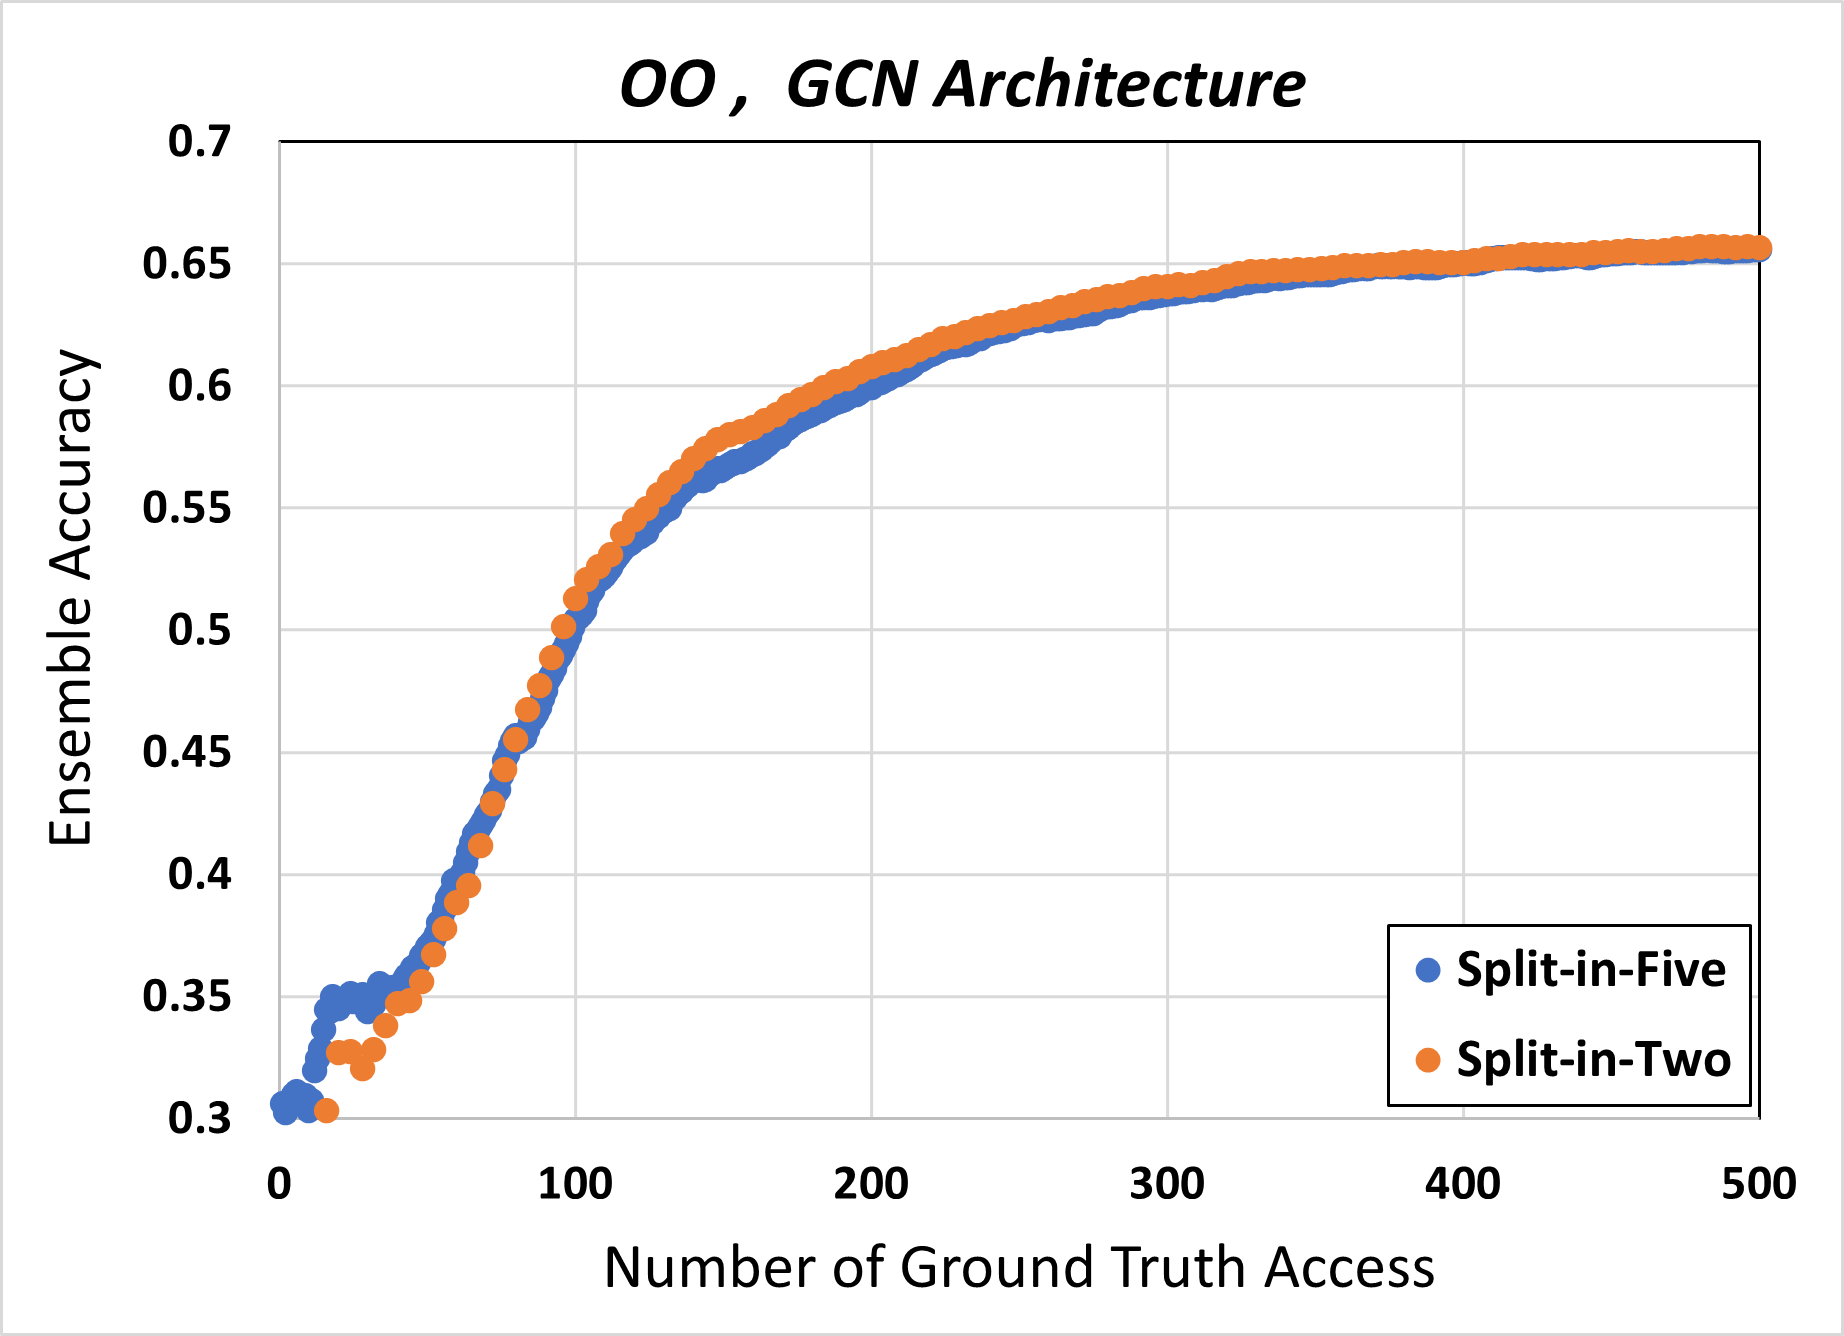}
    \caption{Ensemble accuracy $acc_{\cal E}$ on test set as a function of the number $\alpha$ of oracle sessions, for \textit{C=2}, \textit{C=5}.}
\label{fig:ground-truth-gcn}
\end{figure*}
